# Supplementary material for: Quadratic homogeneous polynomial maps $H$ and Keller maps $x+H$ with $3 \le {\rm rk} J H \le 4$
Source: arXiv:1711.00904 ancillary file (2017-11-02)
Supplement: Supplementary file 1 [file dim5qdr.pdf]

```

[ > restart;
  > efactors := proc (eq)
  >   local F, IF, i, c;
  >   F := factors (eq);
  >   for i from 1 to nops(F[2]) do
  >     c := content (F[2][i][1]);
  >     F[2][i][1] := F[2][i][1] / c;
  >     F[1] := F[1] * c ^ F[2][i][2];
  >   od;
  >   IF := ifactors (F[1]);
  >   return (IF[1], [op(IF[2]), op(F[2])]);
  > end;

```

*efactors* := **proc**(eq)

**local** F, IF, i, c;

F := factors(eq);

**for** i **to** nops(F[2]) **do**

c := content(F[2][i][1]);

F[2][i][1] := F[2][i][1] / c;

F[1] := F[1]\*c^F[2][i][2]

**end do**;

IF := ifactors(F[1]);

**return** IF[1], [op(IF[2]), op(F[2])]

**end proc**

```

[ > psqf := proc (eq)
  >   local EF, S, i;
  >   EF := efactors (eq);
  >   S := EF[1];
  >   for i from 1 to nops(EF[2]) do
  >     if (EF[2][i][2] > 0) then
  >       S := S * EF[2][i][1]
  >     fi
  >   od;
  >   return S
  > end;

```

*psqf* := **proc**(eq)

**local** EF, S, i;

EF := efactors(eq);

S := EF[1];

**for** i **to** nops(EF[2]) **do** **if** 0 < EF[2][i][2] **then** S := S\*EF[2][i][1] **end if** **end do**;

**return** S

**end proc**

```

[ > initcases := proc ()
  >   global nz, NZ, SV;

```

```

> if nargs = 0 then
>   nz := 1
> else
>   nz := args[1];
>   printf ("We assume the following in our calculation:");
>   print (psqf (nz) <> 0);
>   fi;
>   NZ := [convert (nz,string)];
>   SV := [[]];
>   return
> end;

```

*initcases* := **proc**()

**global** *nz, NZ, SV*;

if nargs = 0 then *nz* := 1

else

*nz* := args[ 1];

printf("We assume the following in our calculation:");

print(psqf(*nz*) ≠ 0)

end if;

*NZ* := [convert(*nz*, *string*)];

*SV* := [[ ]];

return

**end proc**

> **launchNZcase** := **proc** (*nz*)

> **global** *NZ, SV*;

> **local** *t*;

> *NZ* := [seq(*NZ*[*i*], *i*=1..*nops*(*NZ*)), convert (*nz*,string)];

> *SV* := [seq(*SV*[*i*], *i*=1..*nops*(*SV*)), []];

> printf ("Launching case level %d:", *nops*(*NZ*) - 1);

> print (*nz* <> 0);

> printf ("Assume from now on that:");

> *t* := mul (psqf (parse (*NZ*[*i*],statement)), *i*=1..*nops*(*NZ*));

> print (*t* <> 0)

> **end**;

*launchNZcase* := **proc**(*nz*)

**local** *t*;

**global** *NZ, SV*;

*NZ* := [seq(*NZ*[*i*], *i* = 1 .. *nops*(*NZ*)), convert(*nz*, *string*)];

*SV* := [seq(*SV*[*i*], *i* = 1 .. *nops*(*SV*)), [ ]];

printf("Launching case level %d:", *nops*(*NZ*) - 1);

print(*nz* ≠ 0);

printf("Assume from now on that:");

```

t := mul(psqf(parse(NZ[i], statement)), i = 1 .. nops(NZ));
print(t ≠ 0)

```

**end proc**

```

> contradict := proc (eq)
>   global NZ, SV, alph;
>   local t, EF, i, sv, nz;
>   t := mul (psqf (parse (NZ[i], statement)), i=1..nops(NZ));
>   EF := efactors (psqf (psqf (eq) / t));
>   if EF[1] = 0 or nops (EF[2]) > 0 then
>     error "No contradiction: 'eq' might be zero!"
>   fi;
>   printf ("Contradiction on case level %d, so:", nops(NZ) - 1);
>   for i from 1 to nops(SV[nops(SV)]) do
>     sv := cat (SV[nops(SV)][i], " := ");
>     sv := cat (sv, SV[nops(SV)][i], "");
>     parse (sv, statement)
>   od;
>   nz := parse (NZ[nops(NZ)], statement);
>   print (nz = 0);
>   if nops(SV[nops(SV)]) > 0 then
>     printf ("Variables to be uneliminated:");
>     for i from 1 to nops(SV[nops(SV)]) do
>       sv := cat (SV[nops(SV)][i], " := ");
>       sv := cat (sv, SV[nops(SV)][i], "");
>       print (sv);
>     od
>   fi;
>   if nops(NZ) <= 1 then
>     printf ("That is all, folks! ");
>     printf ("Check that all variables are uneliminated:");
>     print (alph);
>     return
>   fi;
>   NZ := [seq(NZ[i], i=1..nops(NZ)-1)];
>   SV := [seq(SV[i], i=1..nops(SV)-1)];
>   printf ("Proceed on case level %d with:", nops(NZ) - 1);
>   t := mul (psqf (parse (NZ[i], statement)), i=1..nops(NZ));
>   print (t <> 0);
>   printf ("On account of:");
>   print (nz = 0);
>   if nargs = 1 and nops(indets(nz)) = 1 and degree (nz) = 1 then
>     EF := efactors (psqf (psqf (coeff (nz, indets(nz)[1])) / t));
>     if nops (EF[2]) = 0 then
>       elimsolve(nz, indets(nz)[1]);
>       return
>     fi;
>   fi;

```

```

>   elif nargs > 1 then
>       elimsolve (nz, args[2]);
>       return
>   fi;
>   printf ("the following return value %s",
>           "can be used as an equation:");
>   return nz
> end;

contradict := proc(eq)
local t, EF, i, sv, nz;
global NZ, SV, alph;

    t := mul(psqf(parse(NZ[i], statement)), i = 1 .. nops(NZ));
    EF := efactors(psqf(psqf(eq) / t));
    if EF[1] = 0 or 0 < nops(EF[2]) then error "No contradiction: 'eq' might be zero!"
    end if;
    printf("Contradiction on case level %d, so:", nops(NZ) - 1);
    for i to nops(SV[nops(SV)]) do
        sv := cat(SV[nops(SV)][i], " := ");
        sv := cat(sv, SV[nops(SV)][i], "");
        parse(sv, statement)
    end do;
    nz := parse(NZ[nops(NZ)], statement);
    print(nz = 0);
    if 0 < nops(SV[nops(SV)]) then
        printf("Variables to be uneliminated:");
        for i to nops(SV[nops(SV)]) do
            sv := cat(SV[nops(SV)][i], " := ");
            sv := cat(sv, SV[nops(SV)][i], "");
            print(sv)
        end do
    end if;
    if nops(NZ) ≤ 1 then
        printf("That is all, folks! ");
        printf("Check that all variables are uneliminated:");
        print(alph);
        return
    end if;
    NZ := [seq(NZ[i], i = 1 .. nops(NZ) - 1)];
    SV := [seq(SV[i], i = 1 .. nops(SV) - 1)];
    printf("Proceed on case level %d with:", nops(NZ) - 1);

```

```

t := mul(psqf(parse(NZ[i], statement)), i = 1 .. nops(NZ));
print(t ≠ 0);
printf("On account of:");
print(nz = 0);
if nargs = 1 and nops(indets(nz)) = 1 and degree(nz) = 1 then
    EF := efactors(psqf(psqf(coeff(nz, indets(nz)[1]) / t));
    if nops(EF[2]) = 0 then elimsolve(nz, indets(nz)[1]); return end if
elif 1 < nargs then elimsolve(nz, args[2]); return
end if;
printf("the following return value %s", "can be used as an equation:");
return nz

```

**end proc**

```

> elimsolve := proc (eq, v)
>   global NZ, SV;
>   local t, EF, i, c1, c0, NZref, sv, F;
>   if not ({v} subset indets(v)) then
>     error "Second argument 'v' is not a variable!";
>   fi;
>   t := mul (psqf (parse (NZ[i], statement)), i=1..nops(NZ));
>   EF := efactors (psqf (psqf (eq) / t));
>   if EF[1] = 0 then error "First argument 'eq' is zero!" fi;
>   if nops(EF[2]) = 0 then
>     error "Contradiction: call 'contradict'!"
>   fi;
>   if nops(EF[2]) > 1 then
>     error "'eq' has different factors which may be zero!"
>   fi;
>   if degree (EF[2][1][1], v) <> 1 then
>     error "Degree of 'eq' w.r.t 'v' is not one!"
>   fi;
>   c1 := coeff(EF[2][1][1], v, 1);
>   c0 := coeff(EF[2][1][1], v, 0);
>   EF := efactors (psqf (psqf (c1) / t));
>   if nops(EF[2]) > 0 then
>     error "Coefficient of 'v' in 'eq' might be zero!"
>   fi;
>   EF := efactors (psqf (psqf (denom(eq)) / t));
>   if nops(EF[2]) > 0 then
>     error "Denominator of argument 'eq' may be zero!"
>   fi;
>   print ({c1 <> 0});
>   NZref := false;
>   for i from 1 to nops(NZ) do
>     NZref :=

```

```

>      NZref or ({v} subset indets (parse (NZ[i],statement)));
> od;
> sv := convert (v, string);
> F := factor (-c0/c1);
> SV[nops(SV)] :=
>   [sv, seq(SV[nops(SV)][i], i=1..nops(SV[nops(SV)]))];
> printf ("%s is set to:", sv);
> sv := cat (sv, " := ", convert (F, string));
> print (parse (sv,statement));
> if NZref then
>   printf ("Nonzero constraint refines to:");
>   t := mul (psqf (parse (NZ[i],statement)), i=1..nops (NZ));
>   print (t <> 0)
> fi;
> return
> end;

```

*elimsolve* := **proc**(eq, v)

**local** t, EF, i, c1, c0, NZref, sv, F;

**global** NZ, SV;

```

if not {v} subset indets(v) then error "Second argument 'v' is not a variable!" end if;
t := mul(psqf(parse(NZ[i], statement)), i = 1 .. nops(NZ));
EF := efactors(psqf(psqf(eq) / t));
if EF[1] = 0 then error "First argument 'eq' is zero!" end if;
if nops(EF[2]) = 0 then error "Contradiction: call 'contradict'!" end if;
if 1 < nops(EF[2]) then error "'eq' has different factors which may be zero!" end if;
if degree(EF[2][1][1], v) ≠ 1 then error "Degree of 'eq' w.r.t 'v' is not one!" end if;
c1 := coeff(EF[2][1][1], v, 1);
c0 := coeff(EF[2][1][1], v, 0);
EF := efactors(psqf(psqf(c1) / t));
if 0 < nops(EF[2]) then error "Coefficient of 'v' in 'eq' might be zero!" end if;
EF := efactors(psqf(psqf(denom(eq)) / t));
if 0 < nops(EF[2]) then error "Denominator of argument 'eq' may be zero!" end if;
print({c1 ≠ 0});
NZref := false;
for i to nops(NZ) do NZref := NZref or {v} subset indets(parse(NZ[i], statement))
end do;
sv := convert(v, string);
F := factor(-c0 / c1);
SV[nops(SV)] := [sv, seq(SV[nops(SV)][i], i = 1 .. nops(SV[nops(SV)]))];
printf ("%s is set to:", sv);
sv := cat(sv, " := ", convert(F, string));

```

```

print(parse(sv, statement));
if NZref then
    printf("Nonzero constraint refines to:");
    t := mul(psqf(parse(NZ[i], statement)), i = 1 .. nops(NZ));
    print(t ≠ 0)
end if;
return

```

**end proc**

```

> initcpcoeff := proc (cp)
>   global x1, x2, x3, x4, x5, T, S, n;
>   local deg0, deg1, deg2, deg3, deg4, deg5,
>       cp1, cp2, cp3, cp4, cp5;
>   S := Array (0..(deg-1)*n, 0..(deg-1)*n, 0..(deg-1)*n,
>               0..(deg-1)*n, 0..(deg-1)*n, 0..n,
>               storage=sparse);
>   for deg0 from 0 to n-1 do
>       cp1 := coeff (cp, T, deg0);
>       for deg1 from 0 to (deg-1)*(n-deg0) do
>           cp2 := coeff (cp1, x1, deg1);
>           for deg2 from 0 to (deg-1)*(n-deg0)-deg1 do
>               cp3 := coeff (cp2, x2, deg2);
>               for deg3 from 0 to (deg-1)*(n-deg0)-deg1-deg2 do
>                   cp4 := coeff (cp3, x3, deg3);
>                   for deg4 from 0 to (deg-1)*(n-deg0)-deg1-deg2-deg3 do
>                       cp5 := coeff (cp4, x4, deg4);
>                       deg5 := (deg-1)*(n-deg0)-deg1-deg2-deg3-deg4;
>                       S[deg0,deg1,deg2,deg3,deg4,deg5] :=
>                           coeff (cp5, x5, deg5);
>                   od
>               od
>           od
>       od
>   od;
>   return;
> end;

```

*initcpcoeff*:= **proc**(cp)

**local** deg0, deg1, deg2, deg3, deg4, deg5, cp1, cp2, cp3, cp4, cp5;

**global** x1, x2, x3, x4, x5, T, S, n;

S := Array(0 .. (deg - 1)\*n, 0 .. (deg - 1)\*n, 0 .. (deg - 1)\*n, 0 .. (deg - 1)\*n,  
 0 .. (deg - 1)\*n, 0 .. n, storage = sparse);

**for** deg0 **from** 0 **to** n - 1 **do**

cp1 := coeff(cp, T, deg0);

**for** deg1 **from** 0 **to** (deg - 1)\*(n - deg0) **do**

```

        cp2 := coeff(cp1, x1, deg1);
        for deg2 from 0 to (deg - 1)*(n - deg0) - deg1 do
            cp3 := coeff(cp2, x2, deg2);
            for deg3 from 0 to (deg - 1)*(n - deg0) - deg1 - deg2 do
                cp4 := coeff(cp3, x3, deg3);
                for deg4 from 0 to (deg - 1)*(n - deg0) - deg1 - deg2 - deg3 do
                    cp5 := coeff(cp4, x4, deg4);
                    deg5 := (deg - 1)*(n - deg0) - deg1 - deg2 - deg3 - deg4;
                    S[deg0, deg1, deg2, deg3, deg4, deg5] := coeff(cp5, x5, deg5)
                end do
            end do
        end do
    end do
end do;
return
end proc

```

```

> cpcoeff := proc (t)
>   global x1, x2, x3, x4, x5, T, S;
>   local deg0, deg1, deg2, deg3, deg4, deg5;
>   deg0 := degree (t, T);
>   deg1 := degree (t, x1);
>   deg2 := degree (t, x2);
>   deg3 := degree (t, x3);
>   deg4 := degree (t, x4);
>   deg5 := degree (t, x5);
>   factor (S[deg0, deg1, deg2, deg3, deg4, deg5]) ;
> end;

```

```

cpcoeff:=proc(t)
local deg0, deg1, deg2, deg3, deg4, deg5;
global x1, x2, x3, x4, x5, T, S;
    deg0 := degree(t, T);
    deg1 := degree(t, x1);
    deg2 := degree(t, x2);
    deg3 := degree(t, x3);
    deg4 := degree(t, x4);
    deg5 := degree(t, x5);
    factor(S[deg0, deg1, deg2, deg3, deg4, deg5])
end proc

```

```

end proc
> n := 5;
n := 5
> X := [seq(x||i, i=1..n)];

```



```

X := [x1, x2, x3, x4, x5]
> deg := 2;
deg := 2
> alph :=
> [[a1, b1, c1, d1, e1, f1, g1, h1, i1, j1, k1, l1, m1, n1, o1],
> [a2, b2, c2, d2, e2, f2, g2, h2, i2, j2, k2, l2, m2, n2, o2],
> [a3, b3, c3, d3, e3, f3, g3, h3, i3, j3, k3, l3, m3, n3, o3],
> [a4, b4, c4, d4, e4, f4, g4, h4, i4, j4, k4, l4, m4, n4, o4],
> [a5, b5, c5, d5, e5, f5, g5, h5, i5, j5, k5, l5, m5, n5, o5]] ;
alph := [[a1, b1, c1, d1, e1, f1, g1, h1, i1, j1, k1, l1, m1, n1, o1],
[a2, b2, c2, d2, e2, f2, g2, h2, i2, j2, k2, l2, m2, n2, o2],
[a3, b3, c3, d3, e3, f3, g3, h3, i3, j3, k3, l3, m3, n3, o3],
[a4, b4, c4, d4, e4, f4, g4, h4, i4, j4, k4, l4, m4, n4, o4],
[a5, b5, c5, d5, e5, f5, g5, h5, i5, j5, k5, l5, m5, n5, o5]]
> terms := [x1^2, x1*x2, x1*x3, x1*x4, x1*x5, x2^2, x2*x3,
> x2*x4, x2*x5, x3^2, x3*x4, x3*x5, x4^2, x4*x5, x5^2] ;
terms :=
[x1^2, x1 x2, x1 x3, x1 x4, x1 x5, x2^2, x2 x3, x2 x4, x2 x5, x3^2, x3 x4, x3 x5, x4^2, x4 x5, x5^2]
> M := evalm ([ [0, 0, 0, 0, 0], [1, 0, 0, 0, 0],
> [0, 1, 0, 0, 0], [0, 0, 1, 0, 0], [0, 0, 0, 1, 0] ] ) ;
M :=

$$\begin{bmatrix} 0 & 0 & 0 & 0 & 0 \\ 1 & 0 & 0 & 0 & 0 \\ 0 & 1 & 0 & 0 & 0 \\ 0 & 0 & 1 & 0 & 0 \\ 0 & 0 & 0 & 1 & 0 \end{bmatrix}$$

> H := Vector (evalm (M &* [seq(terms[k]/degree(terms[k]),
> [x1, x2, x3, x4, x5][k]), k=1..n]) +
> ['add (alph[1, k]*terms[k], k=n+1..nops(terms)) '$1=1..n])) ;
H := 
$$\left[ \begin{aligned} &f1 x2^2 + g1 x2 x3 + h1 x2 x4 + i1 x2 x5 + j1 x3^2 + k1 x3 x4 + l1 x3 x5 + m1 x4^2 \\ &+ n1 x4 x5 + o1 x5^2, \frac{x1^2}{2} + f2 x2^2 + g2 x2 x3 + h2 x2 x4 + i2 x2 x5 + j2 x3^2 + k2 x3 x4 \\ &+ l2 x3 x5 + m2 x4^2 + n2 x4 x5 + o2 x5^2, x1 x2 + f3 x2^2 + g3 x2 x3 + h3 x2 x4 + i3 x2 x5 \\ &+ j3 x3^2 + k3 x3 x4 + l3 x3 x5 + m3 x4^2 + n3 x4 x5 + o3 x5^2, x1 x3 + f4 x2^2 + g4 x2 x3 \\ &+ h4 x2 x4 + i4 x2 x5 + j4 x3^2 + k4 x3 x4 + l4 x3 x5 + m4 x4^2 + n4 x4 x5 + o4 x5^2, x1 x4 \\ &+ f5 x2^2 + g5 x2 x3 + h5 x2 x4 + i5 x2 x5 + j5 x3^2 + k5 x3 x4 + l5 x3 x5 + m5 x4^2 + n5 x4 x5 \\ &+ o5 x5^2 \end{aligned} \right]$$

> with (linalg):
Warning, the protected names norm and trace have been redefined and unprotected

```

```
[ > JH := jacobian (H, [x1,x2,x3,x4,x5]) :
[ > cp := expand (det (T-JH)-T^n) :
[ > initcpcoeff (cp);
[ > initcases (2);
```

We assume the following in our calculation:

$$2 \neq 0$$

```
> for i from 1 by -1 to 0 do
>   for j from 1-i by -1 to 0 do
>     for k from 0 to 1-i-j do
>       v := coeff (coeff (coeff (coeff (coeff (H[5],x1,0),
>       x2,i),x3,j),x4,k),x5,2-i-j-k);
>       m := cpcoeff (x2^i * x3^j * x4^k *
>       x5^(1-i-j-k) * T^4);
>       elimsolve (m,v);
>     od;
>   od;
> od;
```

$$\{1 \neq 0\}$$

i5 is set to:

$$-g^3 - h^4 - 2f^2$$

$$\{1 \neq 0\}$$

l5 is set to:

$$-k^4 - g^2 - 2j^3$$

$$\{2 \neq 0\}$$

o5 is set to:

$$-\frac{l^3}{2} - \frac{n^4}{2} - \frac{i^2}{2}$$

$$\{1 \neq 0\}$$

n5 is set to:

$$-k^3 - 2m^4 - h^2$$

```
> for i from 1 by -1 to 0 do
>   for j from 1-i by -1 to 0 do
>     for k from 0 to 1-i-j do
>       v := coeff (coeff (coeff (coeff (coeff (H[4],x1,0),
>       x2,i),x3,j),x4,k),x5,2-i-j-k);
>       m := cpcoeff (x1^1 * x2^i * x3^j * x4^k *
>       x5^(1-i-j-k) * T^3);
>       elimsolve (m,v);
>     od;
>   od;
> od;
```

$$\{1 \neq 0\}$$

i4 is set to:

$$-2fl - h^3 - g^2$$

$$\{1 \neq 0\}$$

l4 is set to:

$$\frac{-g1 - k3 - 2j2}{\{2 \neq 0\}}$$

o4 is set to:

$$\frac{-\frac{n3}{2} - \frac{l2}{2} - \frac{i1}{2}}{\{1 \neq 0\}}$$

n4 is set to:

$$-h1 - 2m3 - k2$$

```
> for i from 1 by -1 to 0 do
>   for j from 1-i by -1 to 0 do
>     for k from 0 to 1-i-j do
>       v := coeff (coeff (coeff (coeff (coeff (H[3],x1,0),
>         x2,i),x3,j),x4,k),x5,2-i-j-k);
>       m := cpcoeff (x1^2 * x2^i * x3^j * x4^k *
>         x5^(1-i-j-k) * T^2);
>       elimsolve (m,v);
>     od;
>   od;
> od;
```

$$\{1 \neq 0\}$$

i3 is set to:

$$\frac{-g1 - h2}{\{1 \neq 0\}}$$

l3 is set to:

$$\frac{-k2 - 2j1}{\{2 \neq 0\}}$$

o3 is set to:

$$\frac{-\frac{l1}{2} - \frac{n2}{2}}{\{1 \neq 0\}}$$

n3 is set to:

$$-k1 - 2m2$$

```
> for i from 1 by -1 to 0 do
>   for j from 1-i by -1 to 0 do
>     for k from 0 to 1-i-j do
>       v := coeff (coeff (coeff (coeff (coeff (H[2],x1,0),
>         x2,i),x3,j),x4,k),x5,2-i-j-k);
>       m := cpcoeff (x1^3 * x2^i * x3^j * x4^k *
>         x5^(1-i-j-k) * T);
>       elimsolve (m,v);
>     od;
>   od;
> od;
```

$$\{1 \neq 0\}$$

i2 is set to:

$$\begin{array}{c} -h l \\ \{1 \neq 0\} \end{array}$$

l2 is set to:

$$\begin{array}{c} -k l \\ \{2 \neq 0\} \end{array}$$

o2 is set to:

$$\begin{array}{c} -\frac{n l}{2} \\ \{1 \neq 0\} \end{array}$$

n2 is set to:

$$-2 m l$$

```
> for i from 1 by -1 to 0 do
>   for j from 1-i by -1 to 0 do
>     for k from 0 to 1-i-j do
>       v := coeff (coeff (coeff (coeff (coeff (H[1],x1,0),
>       x2,i),x3,j),x4,k),x5,2-i-j-k));
>       m := cpcoeff (x1^4 * x2^i * x3^j * x4^k *
>       x5^(1-i-j-k));
>       elimsolve (m,v);
>     od;
>   od;
> od;
```

$$\{1 \neq 0\}$$

i1 is set to:

$$0$$

$$\{1 \neq 0\}$$

l1 is set to:

$$0$$

$$\{1 \neq 0\}$$

o1 is set to:

$$0$$

$$\{1 \neq 0\}$$

n1 is set to:

$$0$$

```
> launchNZcase (m1);
```

Launching case level 1:

$$m l \neq 0$$

Assume from now on that:

$$2 m l \neq 0$$

```
> tmp1 := cpcoeff (x1^2*x5^2*T);
```

$$tmp1 := -4 k2 m l - 4 m l j l - 6 h l m l - 4 m l m3 - 2 k l^2 - 2 k l m2$$

```
> elimsolve (tmp1,k2);
```

$$\{2 m l \neq 0\}$$

k2 is set to:

$$- \frac{2 m l j l + 3 h l m l + 2 m l m 3 + k l^2 + k l m 2}{2 m l}$$

> **tmp1 := cpcoeff (x1^3\*x3\*x5);**

$$tmp1 := \frac{-k l h l m l - k l^3 - k l^2 m 2 + 2 g l m l^2 + 4 m l j l k l + 4 m l j l m 2}{m l}$$

> **elimsolve (tmp1,g1);**

$$\{2 m l^2 \neq 0\}$$

g1 is set to:

$$\frac{k l h l m l + k l^3 + k l^2 m 2 - 4 m l j l k l - 4 m l j l m 2}{2 m l^2}$$

> **tmp1 := cpcoeff (x1^3\*x2\*x5);**

tmp1 :=

$$\frac{4 f l m l^3 + k l^4 + 2 k l^3 m 2 + k l^2 m 2^2 - 4 m l j l k l^2 - 8 m l j l k l m 2 - 4 m l j l m 2^2 - h l^2 m l^2}{m l^2}$$

> **elimsolve (tmp1,f1);**

$$\{4 m l^3 \neq 0\}$$

f1 is set to:

$$\frac{-k l^4 - 2 k l^3 m 2 - k l^2 m 2^2 + 4 m l j l k l^2 + 8 m l j l k l m 2 + 4 m l j l m 2^2 + h l^2 m l^2}{4 m l^3}$$

> **tmp1 := cpcoeff (x1^3\*x4^2);**

$$tmp1 := -(4 m l^2 k 3 + 8 m l^2 m 4 + 4 m l^2 h 2 + k l h l m l + 2 k l m l m 3 - 2 m l j l k l - k l^3 - k l^2 m 2 + 4 h l m l m 2) / (2 m l)$$

> **elimsolve (tmp1,m4);**

$$\{8 m l^2 \neq 0\}$$

m4 is set to:

$$- \frac{4 m l^2 k 3 + 4 m l^2 h 2 + k l h l m l + 2 k l m l m 3 - 2 m l j l k l - k l^3 - k l^2 m 2 + 4 h l m l m 2}{8 m l^2}$$

> **tmp1 := cpcoeff (x1\*x5^2\*T^2);**

$$tmp1 := (3 k l m 2^2 + 2 k l h l m l + 2 m l j l m 2 + 2 m l j l k l - 2 m l^2 h 2 + 3 h l m l m 2 + 2 k l m l m 3 + 2 m l m 3 m 2 + 5 k l^2 m 2 + 2 k l^3) / m l$$

> **elimsolve (tmp1,h2);**

$$\{-2 m l^2 \neq 0\}$$

h2 is set to:

$$(3 k l m 2^2 + 2 k l h l m l + 2 m l j l m 2 + 2 m l j l k l + 3 h l m l m 2 + 2 k l m l m 3 + 2 m l m 3 m 2 + 5 k l^2 m 2 + 2 k l^3) / (2 m l^2)$$

> **tmp1 := cpcoeff (x1^2\*x4^2\*T);**

$$tmp1 := -(9 k l^4 - 16 m l^3 m 5 + 12 k l m 2^3 - 4 m l^2 m 3^2 + 4 m l^2 j l^2 + 24 m l j l k l m 2 + 20 k l h l m l m 2 + 8 m l j l m 2^2 + 12 m l j l k l^2 + 10 k l^2 h l m l + 12 k l m l m 3 m 2 + 8 m l m 3 m 2^2 + h l^2 m l^2 + 4 h l m l^2 j l + 4 h l m l m 2^2 + 4 k l m l^2 k 3 + 8 k l^2 m l m 3)$$

$$-8 h l m^3 m l^2 + 35 k l^2 m^2 + 32 k l^3 m^2) / (4 m l^2)$$

> **elimsolve (tmp1,m5);**

$$\{-16 m l^3 \neq 0\}$$

m5 is set to:

$$(9 k l^4 + 12 k l m^2 m^3 - 4 m l^2 m^3 + 4 m l^2 j l^2 + 24 m l j l k l m^2 + 20 k l h l m l m^2 + 8 m l j l m^2 + 12 m l j l k l^2 + 10 k l^2 h l m l + 12 k l m l m^3 m^2 + 8 m l m^3 m^2 + h l^2 m l^2 + 4 h l m l^2 j l + 4 h l m l m^2 + 4 k l m l^2 k^3 + 8 k l^2 m l m^3 - 8 h l m^3 m l^2 + 35 k l^2 m^2 + 32 k l^3 m^2) / (16 m l^3)$$

> **tmp1 := cpcoeff (x1^2\*x3\*x5\*T);**

$$tmp1 := (5 k l^4 + 8 m l^2 j l^2 + 16 m l^3 j^3 + 8 m l^3 k^4 - 16 m l j l k l m^2 + 10 k l h l m l m^2 - 18 m l j l k l^2 + 11 k l^2 h l m l + 16 g^2 m l^3 + 4 k l m l m^3 m^2 + 4 h l m l^2 j l + 4 k l m l^2 k^3 + 6 k l^2 m l m^3 - 8 m l^2 j l m^3 + 2 k l^2 m^2 + 7 k l^3 m^2 + 16 j^2 m l^2 m^2 + 24 k l j^2 m l^2) / (4 m l^2)$$

> **elimsolve (tmp1,k4);**

$$\{8 m l^3 \neq 0\}$$

k4 is set to:

$$-(5 k l^4 + 8 m l^2 j l^2 + 16 m l^3 j^3 - 16 m l j l k l m^2 + 10 k l h l m l m^2 - 18 m l j l k l^2 + 11 k l^2 h l m l + 16 g^2 m l^3 + 4 k l m l m^3 m^2 + 4 h l m l^2 j l + 4 k l m l^2 k^3 + 6 k l^2 m l m^3 - 8 m l^2 j l m^3 + 2 k l^2 m^2 + 7 k l^3 m^2 + 16 j^2 m l^2 m^2 + 24 k l j^2 m l^2) / (8 m l^3)$$

> **tmp1 := cpcoeff (x1^3\*x3\*x4);**

$$tmp1 := (8 m l^2 j l^2 + 10 m l j l k l m^2 + 6 k l h l m l m^2 + 8 m l j l m^2 + 5 k l^2 h l m l + 4 g^2 m l^3 + 2 k l m l m^3 m^2 + 3 h l^2 m l^2 + 2 h l m l^2 j l + 4 k l^2 m l m^3 + 2 h l m^3 m l^2 - 8 m l^2 j l m^3 - k l^2 m^2 - k l^3 m^2 + 8 j^2 m l^2 m^2 + 8 k l j^2 m l^2) / (2 m l^2)$$

> **elimsolve (tmp1,g2);**

$$\{4 m l^3 \neq 0\}$$

g2 is set to:

$$-(8 m l^2 j l^2 + 10 m l j l k l m^2 + 6 k l h l m l m^2 + 8 m l j l m^2 + 5 k l^2 h l m l + 2 k l m l m^3 m^2 + 3 h l^2 m l^2 + 2 h l m l^2 j l + 4 k l^2 m l m^3 + 2 h l m^3 m l^2 - 8 m l^2 j l m^3 - k l^2 m^2 - k l^3 m^2 + 8 j^2 m l^2 m^2 + 8 k l j^2 m l^2) / (4 m l^3)$$

> **tmp1 := cpcoeff (x1\*x4\*x5\*T^2);**

$$tmp1 := (10 k l^4 + 4 m l^2 m^3 - 20 m l^2 j l^2 - 56 m l j l k l m^2 + 14 k l h l m l m^2 - 32 m l j l m^2 - 18 m l j l k l^2 + 9 k l^2 h l m l + 4 k l m l m^3 m^2 + h l^2 m l^2 - 8 h l m l^2 j l + 8 h l m l m^2 + 8 k l m l^2 k^3 - 2 k l^2 m l m^3 - 4 h l m^3 m l^2 + 16 m l^2 j l m^3 + 13 k l^2 m^2 + 23 k l^3 m^2 + 8 h^3 m l^3 + 8 m^2 m l^2 k^3) / (4 m l^2)$$

> **elimsolve (tmp1,h3);**

$$\{8 m l^3 \neq 0\}$$

h3 is set to:

$$-(10 k l^4 + 4 m l^2 m^3 - 20 m l^2 j l^2 - 56 m l j l k l m^2 + 14 k l h l m l m^2 - 32 m l j l m^2$$

$$\begin{aligned}
& -18 m l j l k l^2 + 9 k l^2 h l m l + 4 k l m l m_3 m_2 + h l^2 m l^2 - 8 h l m l^2 j l + 8 h l m l m_2^2 \\
& + 8 k l m l^2 k_3 - 2 k l^2 m l m_3 - 4 h l m_3 m l^2 + 16 m l^2 j l m_3 + 13 k l^2 m_2^2 + 23 k l^3 m_2 \\
& + 8 m_2 m l^2 k_3) / (8 m l^3)
\end{aligned}$$

> **tmp1 := cpcoeff(x1^2\*x4\*x5^2) ;**

$$\begin{aligned}
tmp1 := & (-16 j_2 m l^2 k l m_2 - 8 m l^2 k_3 k l m_2 + 4 m l^2 j l k l h l + 4 k l h l m l m_2^2 \\
& + 120 k l m l j l m_2^2 - 4 k l^2 m l m_3 m_2 + 144 m l j l k l^2 m_2 - 16 m l^2 j l m_3 m_2 \\
& - 16 m l^2 j l m_3 k l + 8 m l^2 m_3 m_2 h l + 8 k l h l m_3 m l^2 - 8 k l^2 m_2^3 - 37 k l^3 m_2^2 + 32 m l^4 f_2 \\
& + 16 m l^4 h_4 + 16 m l^4 g_3 + 32 m l j l m_2^3 + 12 h l^2 m l^2 m_2 - 16 j_2 m l^2 k l^2 - 8 m l^2 k_3 k l^2 \\
& + 9 k l h l^2 m l^2 - 2 k l^3 m l m_3 + 54 m l j l k l^3 - 9 k l^3 h l m l - 4 k l m l^2 m_3^2 + 16 m l^2 j l^2 m_2 \\
& + 20 m l^2 j l^2 k l - 49 k l^4 m_2 - 20 k l^5 - 4 k l^2 h l m l m_2) / (4 m l^2)
\end{aligned}$$

> **elimsolve (tmp1,g3) ;**

$$\{16 m l^4 \neq 0\}$$

g3 is set to:

$$\begin{aligned}
- & (-16 j_2 m l^2 k l m_2 - 8 m l^2 k_3 k l m_2 + 4 m l^2 j l k l h l + 4 k l h l m l m_2^2 + 120 k l m l j l m_2^2 \\
& - 4 k l^2 m l m_3 m_2 + 144 m l j l k l^2 m_2 - 16 m l^2 j l m_3 m_2 - 16 m l^2 j l m_3 k l \\
& + 8 m l^2 m_3 m_2 h l + 8 k l h l m_3 m l^2 - 8 k l^2 m_2^3 - 37 k l^3 m_2^2 + 32 m l^4 f_2 + 16 m l^4 h_4 \\
& + 32 m l j l m_2^3 + 12 h l^2 m l^2 m_2 - 16 j_2 m l^2 k l^2 - 8 m l^2 k_3 k l^2 + 9 k l h l^2 m l^2 - 2 k l^3 m l m_3 \\
& + 54 m l j l k l^3 - 9 k l^3 h l m l - 4 k l m l^2 m_3^2 + 16 m l^2 j l^2 m_2 + 20 m l^2 j l^2 k l - 49 k l^4 m_2 \\
& - 20 k l^5 - 4 k l^2 h l m l m_2) / (16 m l^4)
\end{aligned}$$

> **tmp1 := cpcoeff(x1^2\*x2\*x5\*T) ;**

$$\begin{aligned}
tmp1 := & -(8 j_2 m l^2 k l m_2 + 2 m l^2 j l m_2 h l + 2 m l^2 j l k l h l + 2 k l m l m_3 m_2^2 \\
& + 6 k l h l m l m_2^2 + 18 k l m l j l m_2^2 + 6 k l^2 m l m_3 m_2 + 10 m l j l k l^2 m_2 - 8 m l^2 j l m_3 m_2 \\
& - 8 m l^2 j l m_3 k l + 2 m l^2 m_3 m_2 h l + 2 k l h l m_3 m l^2 + k l^3 m_2^2 - 4 m l^4 f_2 + 8 m l j l m_2^3 \\
& + 2 h l^2 m l^2 m_2 + 4 j_2 m l^2 k l^2 + 2 k l h l^2 m l^2 + 4 k l^3 m l m_3 + 5 k l^3 h l m l + 8 m l^2 j l^2 m_2 \\
& + 8 m l^2 j l^2 k l + 2 k l^4 m_2 + k l^5 + 4 j_2 m l^2 m_2^2 + 11 k l^2 h l m l m_2) / m l^3
\end{aligned}$$

> **elimsolve (tmp1,f2) ;**

$$\{-4 m l^4 \neq 0\}$$

f2 is set to:

$$\begin{aligned}
& (k l + m_2) (k l^4 + k l^3 m_2 + 4 k l^2 m l m_3 + 5 k l^2 h l m l + 10 m l j l k l m_2 + 4 k l j_2 m l^2 \\
& + 6 k l h l m l m_2 + 2 k l m l m_3 m_2 + 8 m l j l m_2^2 - 8 m l^2 j l m_3 + 8 m l^2 j l^2 + 2 h l^2 m l^2 \\
& + 4 j_2 m l^2 m_2 + 2 h l m l^2 j l + 2 h l m_3 m l^2) / (4 m l^4)
\end{aligned}$$

> **tmp1 := cpcoeff(x1\*x4^2\*T^2) ;**

$$\begin{aligned}
tmp1 := & (8 m l m_3 m_2^3 + 12 h l m l m_2^3 - 8 m l^3 j_3 k l + 8 k_5 m l^4 + 8 m_2 m l^2 m_3^2 + 12 k l m_2^4 \\
& + 8 j_2 m l^2 k l m_2 + 20 m l^2 k_3 k l m_2 + 12 m l^2 j l m_2 h l + 12 m l^2 j l k l h l + 36 k l m l m_3 m_2^2 \\
& + 52 k l h l m l m_2^2 - 12 k l m l j l m_2^2 + 42 k l^2 m l m_3 m_2 + 34 m l j l k l^2 m_2 \\
& + 32 m l^2 j l m_3 m_2 + 8 m l^2 j l m_3 k l + 12 m l^2 m_3 m_2 h l + 12 k l h l m_3 m l^2 + 60 k l^2 m_2^3 \\
& + 92 k l^3 m_2^2 + 8 m l^3 k_3 j l + 8 m_2^2 m l^2 k_3 - 24 m l j l m_2^3 + 8 h l^2 m l^2 m_2 + 4 j_2 m l^2 k l^2
\end{aligned}$$

$$+ 8 m l^2 k_3 k l^2 + 8 m l^3 k_3 h l + 11 k l h l^2 m l^2 + 18 k l^3 m l m_3 + 18 m l j l k l^3 + 22 k l^3 h l m l + 12 k l m l^2 m_3^2 - 8 m l^2 j l^2 m_2 + 12 m l^2 j l^2 k l + 55 k l^4 m_2 + 11 k l^5 + 63 k l^2 h l m l m_2) / (4 m l^3)$$

> **elimsolve (tmp1,k5);**

$$\{8 m l^4 \neq 0\}$$

k5 is set to:

$$- (8 m l m_3 m_2^3 + 12 h l m l m_2^3 - 8 m l^3 j_3 k l + 8 m_2 m l^2 m_3^2 + 12 k l m_2^4 + 8 j_2 m l^2 k l m_2 + 20 m l^2 k_3 k l m_2 + 12 m l^2 j l m_2 h l + 12 m l^2 j l k l h l + 36 k l m l m_3 m_2^2 + 52 k l h l m l m_2^2 - 12 k l m l j l m_2^2 + 42 k l^2 m l m_3 m_2 + 34 m l j l k l^2 m_2 + 32 m l^2 j l m_3 m_2 + 8 m l^2 j l m_3 k l + 12 m l^2 m_3 m_2 h l + 12 k l h l m_3 m l^2 + 60 k l^2 m_2^3 + 92 k l^3 m_2^2 + 8 m l^3 k_3 j l + 8 m_2^2 m l^2 k_3 - 24 m l j l m_2^3 + 8 h l^2 m l^2 m_2 + 4 j_2 m l^2 k l^2 + 8 m l^2 k_3 k l^2 + 8 m l^3 k_3 h l + 11 k l h l^2 m l^2 + 18 k l^3 m l m_3 + 18 m l j l k l^3 + 22 k l^3 h l m l + 12 k l m l^2 m_3^2 - 8 m l^2 j l^2 m_2 + 12 m l^2 j l^2 k l + 55 k l^4 m_2 + 11 k l^5 + 63 k l^2 h l m l m_2) / (8 m l^4)$$

> **tmp1 := cpcoeff(x4\*x5\*T^3);**

$$tmp1 := (-16 m l^3 j_3 k l + 16 m l^3 m_3 j_2 + 8 j_2 m l^2 k l m_2 + 28 m l^2 j l m_2 h l + 24 m l^2 j l k l h l + 16 k l h l m l m_2^2 + 132 k l m l j l m_2^2 + 6 k l^2 m l m_3 m_2 + 146 m l j l k l^2 m_2 - 8 m l^2 j l m_3 m_2 - 32 m l^2 j l m_3 k l + 16 m l^2 m_3 m_2 h l + 24 k l h l m_3 m l^2 - 8 k l^2 m_2^3 - 34 k l^3 m_2^2 + 8 m l^4 h_4 + 16 m l^3 k_3 j l - 16 m_2 m l^3 j_3 + 32 m l j l m_2^3 + 20 h l^2 m l^2 m_2 + 4 j_2 m l^2 k l^2 - 4 m l^2 k_3 k l^2 + 4 m l^3 k_3 h l + 15 k l h l^2 m l^2 + 10 k l^3 m l m_3 + 42 m l j l k l^3 + 4 k l^3 h l m l + 4 k l m l^2 m_3^2 + 24 m l^2 j l^2 m_2 + 44 m l^2 j l^2 k l - 41 k l^4 m_2 - 15 k l^5 + 21 k l^2 h l m l m_2) / (4 m l^3)$$

> **elimsolve (tmp1,h4);**

$$\{8 m l^4 \neq 0\}$$

h4 is set to:

$$- (-16 m l^3 j_3 k l + 16 m l^3 m_3 j_2 + 8 j_2 m l^2 k l m_2 + 28 m l^2 j l m_2 h l + 24 m l^2 j l k l h l + 16 k l h l m l m_2^2 + 132 k l m l j l m_2^2 + 6 k l^2 m l m_3 m_2 + 146 m l j l k l^2 m_2 - 8 m l^2 j l m_3 m_2 - 32 m l^2 j l m_3 k l + 16 m l^2 m_3 m_2 h l + 24 k l h l m_3 m l^2 - 8 k l^2 m_2^3 - 34 k l^3 m_2^2 + 16 m l^3 k_3 j l - 16 m_2 m l^3 j_3 + 32 m l j l m_2^3 + 20 h l^2 m l^2 m_2 + 4 j_2 m l^2 k l^2 - 4 m l^2 k_3 k l^2 + 4 m l^3 k_3 h l + 15 k l h l^2 m l^2 + 10 k l^3 m l m_3 + 42 m l j l k l^3 + 4 k l^3 h l m l + 4 k l m l^2 m_3^2 + 24 m l^2 j l^2 m_2 + 44 m l^2 j l^2 k l - 41 k l^4 m_2 - 15 k l^5 + 21 k l^2 h l m l m_2) / (8 m l^4)$$

> **tmp1 := cpcoeff(x3\*x5\*T^3);**

$$tmp1 := - (-48 j_2 m l^2 k l^3 + 32 j_2 m l^3 j l m_2 + 16 j_2 m l^3 j l k l + 32 h l j_3 m l^4 - 104 j_2 m l^2 k l^2 m_2 - 56 j_2 m l^3 k l h l - 56 m l^3 j l k l k_3 + 112 m l^2 j l h l m_2^2 + 20 m l^2 j l k l^2 h l + 340 m l^2 j l^2 k l m_2 - 96 j_2 m l^3 m_3 m_2 - 112 j_2 m l^3 k l m_3 - 80 j_2 m l^3 h l m_2 - 48 j_2 m l^2 k l m_2^2 - 26 m l j l k l^2 m_2^2 - 40 m l^2 j l k l^2 m_3 - 138 m l j l k l^4$$



$$\begin{aligned}
& -16 m l^3 j l m_2 k_3 - 300 m l j l k l^3 m_2 - 135 h l^2 m l^2 k l m_2 + 54 m l^3 j l h l^2 \\
& - 416 h l m l k l^3 m_2 + 88 m l^2 j l^2 k l^2 - 521 h l m l k l^2 m_2^2 + 192 m l^2 j l^2 m_2^2 + 56 m l^3 j l m_3^2 \\
& - 120 h l m l^2 k l^2 m_3 - 76 h l m l^3 k l k_3 - 36 h l m l^3 m_3^2 - 109 h l m l k l^4 + 76 m l^3 j l^2 h l \\
& - 160 m l^2 m_3 j l m_2^2 - 28 k l^6 - 280 m l^2 j l k l m_3 m_2 + 156 m l^2 j l k l h l m_2 \\
& - 72 h l m l^3 m_2 k_3 - 16 m l^3 m_3 m_2 k_3 - 224 m l m_3 k l^3 m_2 - 310 m l m_3 k l^2 m_2^2 \\
& - 8 m l^3 m_3 k l k_3 - 64 m l^2 m_3 h l m_2^2 - 72 h l^2 m l^2 k l^2 - 24 m l^3 m_3 h l j l \\
& - 108 m l^2 m_3^2 k l m_2 - 196 h l m l^2 k l m_3 m_2 - 66 m l m_3 k l^4 - 56 h l^2 m l^2 m_2^2 \\
& - 140 k l^2 m_2 m l^2 k_3 - 32 g_4 m l^5 - 96 m l^2 m_3^2 k l^2 + 224 k l m_2^3 m l j l - 30 m l^3 m_3 h l^2 \\
& - 120 m l^3 m_3 j l^2 - 264 k l m_2^3 h l m l + 64 j_5 m l^5 - 44 k l^3 m l^2 k_3 + 72 m l^3 j l^3 + 9 h l^3 m l^3 \\
& - 584 k l^4 m_2^2 - 8 m l^3 m_3^3 - 617 k l^3 m_2^3 - 235 k l^5 m_2 - 120 k l m_2^2 m l^2 k_3 - 288 k l^2 m_2^4 \\
& + 64 m l^3 j_3 k l^2 - 48 k l m_2^5 + 64 m_2 m l^3 j_3 k l - 176 k l m l m_3 m_2^3 - 32 m_2^2 m l^2 m_3^2 \\
& - 48 h l m l m_2^4 - 32 m l m_3 m_2^4 + 96 m l j l m_2^4 - 16 m l^4 k_3^2 - 32 m_2^3 m l^2 k_3 \\
& + 64 m l^4 j_3 m_3 - 64 m l^4 j_3 j l - 32 m l^4 k_3 j_2 - 64 j_4 m l^4 m_2 - 32 j_4 m l^4 k l) / (16 m l^4)
\end{aligned}$$

> **elimsolve (tmp1,g4) ;**

$$\{-32 m l^5 \neq 0\}$$

g4 is set to:

$$\begin{aligned}
& (-48 j_2 m l^2 k l^3 + 32 j_2 m l^3 j l m_2 + 16 j_2 m l^3 j l k l + 32 h l j_3 m l^4 - 104 j_2 m l^2 k l^2 m_2 \\
& - 56 j_2 m l^3 k l h l - 56 m l^3 j l k l k_3 + 112 m l^2 j l h l m_2^2 + 20 m l^2 j l k l^2 h l \\
& + 340 m l^2 j l^2 k l m_2 - 96 j_2 m l^3 m_3 m_2 - 112 j_2 m l^3 k l m_3 - 80 j_2 m l^3 h l m_2 \\
& - 48 j_2 m l^2 k l m_2^2 - 26 m l j l k l^2 m_2^2 - 40 m l^2 j l k l^2 m_3 - 138 m l j l k l^4 - 16 m l^3 j l m_2 k_3 \\
& - 300 m l j l k l^3 m_2 - 135 h l^2 m l^2 k l m_2 + 54 m l^3 j l h l^2 - 416 h l m l k l^3 m_2 \\
& + 88 m l^2 j l^2 k l^2 - 521 h l m l k l^2 m_2^2 + 192 m l^2 j l^2 m_2^2 + 56 m l^3 j l m_3^2 \\
& - 120 h l m l^2 k l^2 m_3 - 76 h l m l^3 k l k_3 - 36 h l m l^3 m_3^2 - 109 h l m l k l^4 + 76 m l^3 j l^2 h l \\
& - 160 m l^2 m_3 j l m_2^2 - 28 k l^6 - 280 m l^2 j l k l m_3 m_2 + 156 m l^2 j l k l h l m_2 \\
& - 72 h l m l^3 m_2 k_3 - 16 m l^3 m_3 m_2 k_3 - 224 m l m_3 k l^3 m_2 - 310 m l m_3 k l^2 m_2^2 \\
& - 8 m l^3 m_3 k l k_3 - 64 m l^2 m_3 h l m_2^2 - 72 h l^2 m l^2 k l^2 - 24 m l^3 m_3 h l j l \\
& - 108 m l^2 m_3^2 k l m_2 - 196 h l m l^2 k l m_3 m_2 - 66 m l m_3 k l^4 - 56 h l^2 m l^2 m_2^2 \\
& - 140 k l^2 m_2 m l^2 k_3 - 96 m l^2 m_3^2 k l^2 + 224 k l m_2^3 m l j l - 30 m l^3 m_3 h l^2 - 120 m l^3 m_3 j l^2 \\
& - 264 k l m_2^3 h l m l + 64 j_5 m l^5 - 44 k l^3 m l^2 k_3 + 72 m l^3 j l^3 + 9 h l^3 m l^3 - 584 k l^4 m_2^2 \\
& - 8 m l^3 m_3^3 - 617 k l^3 m_2^3 - 235 k l^5 m_2 - 120 k l m_2^2 m l^2 k_3 - 288 k l^2 m_2^4 + 64 m l^3 j_3 k l^2 \\
& - 48 k l m_2^5 + 64 m_2 m l^3 j_3 k l - 176 k l m l m_3 m_2^3 - 32 m_2^2 m l^2 m_3^2 - 48 h l m l m_2^4 \\
& - 32 m l m_3 m_2^4 + 96 m l j l m_2^4 - 16 m l^4 k_3^2 - 32 m_2^3 m l^2 k_3 + 64 m l^4 j_3 m_3 - 64 m l^4 j_3 j l \\
& - 32 m l^4 k_3 j_2 - 64 j_4 m l^4 m_2 - 32 j_4 m l^4 k l) / (32 m l^5)
\end{aligned}$$

> **tmp1 := cpcoeff(x4^2\*T^3) ;**

$$\begin{aligned}
& tmp1 := -(4 j_2 m l^2 k l^3 + 32 m_2^2 m l^3 j_3 + 8 j_2 m l^2 k l^2 m_2 + 24 m l^3 j l k l k_3 \\
& - 32 m l^2 j l h l m_2^2 + 20 m l^2 j l k l^2 h l - 100 m l^2 j l^2 k l m_2 + 16 j_2 m l^3 k l m_3
\end{aligned}$$

$$\begin{aligned}
& -160 m l j l k l^2 m^2 + 40 m l^2 j l k l^2 m^3 + 46 m l j l k l^4 + 66 m l j l k l^3 m^2 + 71 h l^2 m l^2 k l m^2 \\
& -8 m l^3 j l h l^2 + 243 h l m l k l^3 m^2 + 4 m l^2 j l^2 k l^2 + 296 h l m l k l^2 m^2 - 80 m l^2 j l^2 m^2 \\
& -32 m l^3 j l m^3 + 48 h l m l^2 k l^2 m^3 + 32 h l m l^3 k l k^3 + 24 h l m l^3 m^3 + 66 h l m l k l^4 \\
& -32 m l^3 j l^2 h l + 128 m l^2 m^3 j l m^2 + 27 k l^6 + 200 m l^2 j l k l m^3 m^2 - 16 m l^2 j l k l h l m^2 \\
& + 40 h l m l^3 m^2 k^3 + 16 m l^3 m^3 m^2 k^3 + 98 m l m^3 k l^3 m^2 + 154 m l m^3 k l^2 m^2 \\
& + 8 m l^3 m^3 k l k^3 + 32 m l^2 m^3 h l m^2 + 41 h l^2 m l^2 k l^2 + 8 m l^3 m^3 h l j l + 44 m l^2 m^3 k l m^2 \\
& + 80 h l m l^2 k l m^3 m^2 + 28 m l m^3 k l^4 + 28 h l^2 m l^2 m^2 + 72 k l^2 m^2 m l^2 k^3 \\
& + 36 m l^2 m^3 k l^2 - 288 k l m^2 m^3 m l j l + 14 m l^3 m^3 h l^2 + 40 m l^3 m^3 j l^2 + 144 k l m^2 m^3 h l m l \\
& + 20 k l^3 m l^2 k^3 - 16 m l^3 j l^3 + 2 h l^3 m l^3 + 402 k l^4 m^2 + 8 m l^3 m^3 + 399 k l^3 m^2 \\
& + 178 k l^5 m^2 + 64 k l m^2 m l^2 k^3 + 172 k l^2 m^2 + 8 m l^3 j^3 k l^2 + 24 k l m^2 + 16 m^2 m l^3 j^3 k l \\
& + 96 k l m l m^3 m^2 + 16 m^2 m l^2 m^3 + 24 h l m l m^2 + 16 m l m^3 m^2 - 112 m l j l m^2 \\
& + 8 m l^4 k^3 + 16 m^2 m l^2 k^3 - 32 m l^4 j^3 m^3 - 16 h^5 m l^5) / (8 m l^4)
\end{aligned}$$

> **elimsolve (tmp1, h5);**

$$\{-16 m l^5 \neq 0\}$$

h5 is set to:

$$\begin{aligned}
& (4 j^2 m l^2 k l^3 + 32 m^2 m l^3 j^3 + 8 j^2 m l^2 k l^2 m^2 + 24 m l^3 j l k l k^3 - 32 m l^2 j l h l m^2 \\
& + 20 m l^2 j l k l^2 h l - 100 m l^2 j l^2 k l m^2 + 16 j^2 m l^3 k l m^3 - 160 m l j l k l^2 m^2 \\
& + 40 m l^2 j l k l^2 m^3 + 46 m l j l k l^4 + 66 m l j l k l^3 m^2 + 71 h l^2 m l^2 k l m^2 - 8 m l^3 j l h l^2 \\
& + 243 h l m l k l^3 m^2 + 4 m l^2 j l^2 k l^2 + 296 h l m l k l^2 m^2 - 80 m l^2 j l^2 m^2 - 32 m l^3 j l m^3 \\
& + 48 h l m l^2 k l^2 m^3 + 32 h l m l^3 k l k^3 + 24 h l m l^3 m^3 + 66 h l m l k l^4 - 32 m l^3 j l^2 h l \\
& + 128 m l^2 m^3 j l m^2 + 27 k l^6 + 200 m l^2 j l k l m^3 m^2 - 16 m l^2 j l k l h l m^2 \\
& + 40 h l m l^3 m^2 k^3 + 16 m l^3 m^3 m^2 k^3 + 98 m l m^3 k l^3 m^2 + 154 m l m^3 k l^2 m^2 \\
& + 8 m l^3 m^3 k l k^3 + 32 m l^2 m^3 h l m^2 + 41 h l^2 m l^2 k l^2 + 8 m l^3 m^3 h l j l + 44 m l^2 m^3 k l m^2 \\
& + 80 h l m l^2 k l m^3 m^2 + 28 m l m^3 k l^4 + 28 h l^2 m l^2 m^2 + 72 k l^2 m^2 m l^2 k^3 \\
& + 36 m l^2 m^3 k l^2 - 288 k l m^2 m^3 m l j l + 14 m l^3 m^3 h l^2 + 40 m l^3 m^3 j l^2 + 144 k l m^2 m^3 h l m l \\
& + 20 k l^3 m l^2 k^3 - 16 m l^3 j l^3 + 2 h l^3 m l^3 + 402 k l^4 m^2 + 8 m l^3 m^3 + 399 k l^3 m^2 \\
& + 178 k l^5 m^2 + 64 k l m^2 m l^2 k^3 + 172 k l^2 m^2 + 8 m l^3 j^3 k l^2 + 24 k l m^2 + 16 m^2 m l^3 j^3 k l \\
& + 96 k l m l m^3 m^2 + 16 m^2 m l^2 m^3 + 24 h l m l m^2 + 16 m l m^3 m^2 - 112 m l j l m^2 \\
& + 8 m l^4 k^3 + 16 m^2 m l^2 k^3 - 32 m l^4 j^3 m^3) / (16 m l^5)
\end{aligned}$$

> **tmp1 := cpccoeff(x2\*x5\*T^3);**

$$\begin{aligned}
& tmp1 := -(-96 h l m l^4 j^3 k l + 32 h l m l^4 m^3 j^2 + 20 h l^2 m l^4 k^3 - 320 m l^2 j l k l^3 h l \\
& + 420 m l j l k l^4 m^2 - 440 m l^3 j l k l m^3 - 230 m l^3 j l k l h l^2 + 264 m l^2 j l k l^3 m^3 \\
& + 64 m l^3 j l k^3 k l^2 - 1548 m l^2 j l k l^2 h l m^2 - 272 m l^3 j l h l^2 m^2 - 160 m l^3 j l j^2 k l^2 \\
& - 328 m l^2 j l^2 k l^3 - 742 m l j l k l^3 m^2 + 256 m l^4 j l m^2 j^3 - 208 m l^4 j l^2 k^3 \\
& + 448 m l^3 j l m^3 m^2 h l + 248 m l^3 j l k l h l m^3 + 384 m l^3 j l^2 m^3 m^2 - 2640 m l j l k l^2 m^2 \\
& + 600 m l^3 j l^2 m^3 k l + 1768 m l^2 j l k l^2 m^3 m^2 - 1620 m l^2 j l^2 k l^2 m^2 - 768 m l^2 j l^2 m^2)
\end{aligned}$$

$$\begin{aligned}
& -516 m l^3 j l^2 k l h l - 2096 m l^2 j l^2 k l m^2 - 480 m l^3 j l j_2 k l m_2 - 2176 m l^2 j l k l h l m^2 \\
& + 512 h l m l^3 j_2 k l m_2 + 956 h l^2 m l^2 k l m^2 + 8 h l^3 m l^3 m_2 + 816 k l^3 j_2 m l^2 m_2 \\
& + 256 k l^4 j_2 m l^2 + 928 m l m_3 k l^4 m_2 + 220 k l^7 + 3872 k l^5 m^2 + 16 m l^4 m_3 k_3 h l \\
& + 368 m l^2 m_3^2 k l^3 + 288 m l^3 m_3 j_2 k l^2 + 48 m l^3 m_3 k_3 k l^2 + 104 m l^3 m_3^3 k l \\
& + 896 m l^2 m_3 j l m^2 + 1862 m l m_3 k l^3 m^2 - 384 m l^4 m_3 m_2 j_3 + 192 m l^4 m_3 k_3 j l \\
& + 1840 m l m_3 k l^2 m^2 + 320 m l^3 m_3^2 m_2 h l + 3884 k l^3 m^2 + 2432 m l^2 m_3 k l j l m^2 \\
& + 764 m l^2 m_3^2 k l^2 m_2 + 1168 m l^2 m_3 k l h l m^2 - 256 m l^3 m_3^2 j l m_2 + 963 h l^2 m l^2 k l^2 m_2 \\
& - 320 m l^4 m_3 j_3 k l + 2602 h l m l k l^4 m_2 + 640 m l^3 m_3 j_2 k l m_2 + 380 h l m l^3 k l m_3^2 \\
& + 312 h l m l^3 k_3 k l^2 + 412 h l m l^2 k l^3 m_3 - 128 h l m l^4 m_2 j_3 - 928 h l m l^2 j l m^2 \\
& + 224 h l m l^3 j_2 k l^2 + 4383 h l m l k l^3 m^2 + 222 h l^2 m l^3 k l m_3 + 3472 h l m l k l^2 m^2 \\
& + 1284 h l m l^2 k l^2 m_3 m_2 + 256 h l^2 m l^3 m_3 m_2 - 672 m l^3 j l^2 m_2 h l - 128 f_4 m l^6 \\
& + 64 g_5 m l^6 + 192 m l^4 j l j_3 k l + 64 k l m^2 m l^3 j_3 - 2304 k l m^2 m l j l - 80 k l m_2 m l^3 k_3 j l \\
& + 824 k l^2 m^2 j_2 m l^2 + 1447 k l^6 m_2 - 160 k l^2 m_2 m l^3 j_3 + 5313 k l^4 m^2 \\
& + 736 k l m_2 m l^3 k_3 h l + 528 k l m l^2 m_3^2 m^2 + 816 k l^3 m_2 m l^2 k_3 + 640 k l m^2 m l^2 k_3 \\
& + 1132 k l^2 m^2 m l^2 k_3 + 1296 k l m^2 h l m l + 256 j_2 m l^2 m^2 k l + 256 j_2 m l^3 m^2 m_3 \\
& + 320 j_2 m l^3 m^2 h l - 256 j_2 m l^3 m^2 j l + 5 h l^3 m l^3 k l + 194 m l j l k l^5 - 264 m l^3 j l^3 k l \\
& - 192 m l^3 j l^3 m_2 - 64 f_3 k l m l^5 + 288 m l^2 m_3 m^2 h l + 224 k l m l^3 m_3 m_2 k_3 \\
& + 416 h l m l^3 m^2 k_3 + 64 m l^3 m_3^3 m_2 + 304 h l^2 m l^2 m^2 + 204 k l^4 m l^2 k_3 - 96 k l^3 m l^3 j_3 \\
& + 194 m l m_3 k l^5 - 128 m l^3 j l m^2 k_3 + 160 m l^4 m_3^2 j_2 + 589 h l m l k l^5 + 322 h l^2 m l^2 k l^3 \\
& + 128 m l^3 m_3 m^2 k_3 + 96 m_2 m l^4 k^2 + 128 m^2 m l^2 k_3 - 640 m l j l m^2 + 128 m l m_3 m^2 \\
& + 192 h l m l m^2 + 128 m^2 m l^2 m_3^2 + 128 m^2 m l^3 j_3 + 8 j_2 m l^4 h l^2 - 160 j_2 m l^4 j l^2 \\
& + 32 j_4 m l^4 k l^2 + 128 j_4 m l^4 m^2 + 192 k l m^2 + 832 k l m l m_3 m^2 + 80 k l m l^4 k^2 \\
& + 16 m l^4 k_3 m^2 + 128 j_2 m l^4 m_2 k_3 + 96 j_2 m l^4 k l k_3 - 64 j_2 m l^4 h l j l + 1408 k l^2 m^2 \\
& - 64 j_5 m l^5 k l - 128 j_5 m l^5 m_2 + 128 j_4 m l^4 m_2 k l) / (32 m l^5)
\end{aligned}$$

> **elimsolve (tmp1,f4) ;**

$$\{-128 m l^6 \neq 0\}$$

f4 is set to:

$$\begin{aligned}
& (-96 h l m l^4 j_3 k l + 32 h l m l^4 m_3 j_2 + 20 h l^2 m l^4 k_3 - 320 m l^2 j l k l^3 h l + 420 m l j l k l^4 m_2 \\
& - 440 m l^3 j l k l m_3^2 - 230 m l^3 j l k l h l^2 + 264 m l^2 j l k l^3 m_3 + 64 m l^3 j l k_3 k l^2 \\
& - 1548 m l^2 j l k l^2 h l m_2 - 272 m l^3 j l h l^2 m_2 - 160 m l^3 j l j_2 k l^2 - 328 m l^2 j l^2 k l^3 \\
& - 742 m l j l k l^3 m^2 + 256 m l^4 j l m_2 j_3 - 208 m l^4 j l^2 k_3 + 448 m l^3 j l m_3 m_2 h l \\
& + 248 m l^3 j l k l h l m_3 + 384 m l^3 j l^2 m_3 m_2 - 2640 m l j l k l^2 m^2 + 600 m l^3 j l^2 m_3 k l \\
& + 1768 m l^2 j l k l^2 m_3 m_2 - 1620 m l^2 j l^2 k l^2 m_2 - 768 m l^2 j l^2 m^2 - 516 m l^3 j l^2 k l h l \\
& - 2096 m l^2 j l^2 k l m^2 - 480 m l^3 j l j_2 k l m_2 - 2176 m l^2 j l k l h l m^2 + 512 h l m l^3 j_2 k l m_2 \\
& + 956 h l^2 m l^2 k l m^2 + 8 h l^3 m l^3 m_2 + 816 k l^3 j_2 m l^2 m_2 + 256 k l^4 j_2 m l^2 \\
& + 928 m l m_3 k l^4 m_2 + 220 k l^7 + 3872 k l^5 m^2 + 16 m l^4 m_3 k_3 h l + 368 m l^2 m_3^2 k l^3
\end{aligned}$$

$$\begin{aligned}
& + 288 m l^3 m_3 j_2 k l^2 + 48 m l^3 m_3 k_3 k l^2 + 104 m l^3 m_3^3 k l + 896 m l^2 m_3 j l m_2^3 \\
& + 1862 m l m_3 k l^3 m_2^2 - 384 m l^4 m_3 m_2 j_3 + 192 m l^4 m_3 k_3 j l + 1840 m l m_3 k l^2 m_2^3 \\
& + 320 m l^3 m_3^2 m_2 h l + 3884 k l^3 m_2^4 + 2432 m l^2 m_3 k l j l m_2^2 + 764 m l^2 m_3^2 k l^2 m_2 \\
& + 1168 m l^2 m_3 k l h l m_2^2 - 256 m l^3 m_3^2 j l m_2 + 963 h l^2 m l^2 k l^2 m_2 - 320 m l^4 m_3 j_3 k l \\
& + 2602 h l m l k l^4 m_2 + 640 m l^3 m_3 j_2 k l m_2 + 380 h l m l^3 k l m_3^2 + 312 h l m l^3 k_3 k l^2 \\
& + 412 h l m l^2 k l^3 m_3 - 128 h l m l^4 m_2 j_3 - 928 h l m l^2 j l m_2^3 + 224 h l m l^3 j_2 k l^2 \\
& + 4383 h l m l k l^3 m_2^2 + 222 h l^2 m l^3 k l m_3 + 3472 h l m l k l^2 m_2^3 + 1284 h l m l^2 k l^2 m_3 m_2 \\
& + 256 h l^2 m l^3 m_3 m_2 - 672 m l^3 j l^2 m_2 h l + 64 g_5 m l^6 + 192 m l^4 j l j_3 k l + 64 k l m_2^2 m l^3 j_3 \\
& - 2304 k l m_2^4 m l j l - 80 k l m_2 m l^3 k_3 j l + 824 k l^2 m_2^2 j_2 m l^2 + 1447 k l^6 m_2 \\
& - 160 k l^2 m_2 m l^3 j_3 + 5313 k l^4 m_2^3 + 736 k l m_2 m l^3 k_3 h l + 528 k l m l^2 m_3^2 m_2^2 \\
& + 816 k l^3 m_2 m l^2 k_3 + 640 k l m_2^3 m l^2 k_3 + 1132 k l^2 m_2^2 m l^2 k_3 + 1296 k l m_2^4 h l m l \\
& + 256 j_2 m l^2 m_2^3 k l + 256 j_2 m l^3 m_2^2 m_3 + 320 j_2 m l^3 m_2^2 h l - 256 j_2 m l^3 m_2^2 j l \\
& + 5 h l^3 m l^3 k l + 194 m l j l k l^5 - 264 m l^3 j l^3 k l - 192 m l^3 j l^3 m_2 - 64 f_3 k l m l^5 \\
& + 288 m l^2 m_3 m_2^3 h l + 224 k l m l^3 m_3 m_2 k_3 + 416 h l m l^3 m_2^2 k_3 + 64 m l^3 m_3^3 m_2 \\
& + 304 h l^2 m l^2 m_2^3 + 204 k l^4 m l^2 k_3 - 96 k l^3 m l^3 j_3 + 194 m l m_3 k l^5 - 128 m l^3 j l m_2^2 k_3 \\
& + 160 m l^4 m_3^2 j_2 + 589 h l m l k l^5 + 322 h l^2 m l^2 k l^3 + 128 m l^3 m_3 m_2^2 k_3 + 96 m_2 m l^4 k_3^2 \\
& + 128 m_2^4 m l^2 k_3 - 640 m l j l m_2^5 + 128 m l m_3 m_2^5 + 192 h l m l m_2^5 + 128 m_2^3 m l^2 m_3^2 \\
& + 128 m_2^3 m l^3 j_3 + 8 j_2 m l^4 h l^2 - 160 j_2 m l^4 j l^2 + 32 j_4 m l^4 k l^2 + 128 j_4 m l^4 m_2^2 \\
& + 192 k l m_2^6 + 832 k l m l m_3 m_2^4 + 80 k l m l^4 k_3^2 + 16 m l^4 k_3 m_3^2 + 128 j_2 m l^4 m_2 k_3 \\
& + 96 j_2 m l^4 k l k_3 - 64 j_2 m l^4 h l j l + 1408 k l^2 m_2^5 - 64 j_5 m l^5 k l - 128 j_5 m l^5 m_2 \\
& + 128 j_4 m l^4 m_2 k l) / (128 m l^6)
\end{aligned}$$

> **tmp1 := cpcoeff(x2\*x4\*T^3) ;**

$$\begin{aligned}
tmp1 := & (384 m l^4 m_3 j_2 k l h l - 128 m l^4 m_3 j_2 j l m_2 - 192 m l^4 m_3 j_2 j l k l \\
& + 256 m l^4 m_3 j_2 h l m_2 - 80 m l^4 j l^4 - 9348 k l^3 m_2^5 - 3013 k l^7 m_2 - 8951 k l^6 m_2^2 \\
& - 15111 k l^5 m_2^3 + 256 f_5 m l^7 - 64 k l m l^6 - 384 k l m_2^7 + 256 m l^5 m_3 j_4 m_2 \\
& + 128 m l^5 m_3 j_4 k l - 256 m l^6 m_3 j_5 + 128 m_2 j_5 m l^5 k l - 64 m_2 j_4 m l^4 k l^2 \\
& - 256 j_4 m l^4 m_2^2 k l - 256 m_2^4 m l^3 j_3 - 256 j_4 m l^4 m_2^3 + 256 j_5 m l^5 m_2^2 + 64 g_5 m l^6 k l \\
& - 192 m_2^2 m l^4 k_3^2 - 256 m_2^5 m l^2 k_3 + 1280 m l j l m_2^6 - 256 m l m_3 m_2^6 - 384 h l m l m_2^6 \\
& + 320 m l^4 j l m_2 j_3 k l + 384 m l^3 j l m_2^2 j_2 k l + 1280 m l^2 j l^2 m_2^4 + 1344 m l^2 j l m_2^4 h l \\
& + 1568 m l^3 j l m_2^2 m_3^2 + 5120 m l j l m_2^5 k l + 880 m l^3 j l^2 m_2^2 h l + 632 m l^3 j l k l^2 m_3^2 \\
& - 192 m l^3 j l^3 k l m_2 - 2432 m l^2 j l m_2^4 m_3 - 208 m l^4 j l^2 k l k_3 + 3600 m l^2 j l^2 k l m_2^3 \\
& - 176 m l^3 j l k l^3 j_2 - 2672 m l^3 j l^2 k l m_3 m_2 - 248 m l^3 j l^3 k l^2 - 128 m l^3 j l k l^2 j_2 m_2 \\
& - 608 m l^3 j l k l m_2^2 k_3 - 7072 m l^2 j l k l m_3 m_2^3 + 2848 m l^3 j l k l m_2 m_3^2 \\
& + 3048 k l^2 m_2^2 m l^2 j l^2 + 192 m l^4 j l k l^2 j_3 - 600 m l^3 j l^2 k l^2 m_3 - 5704 k l^2 m_2^2 m l^2 j l m_3 \\
& - 1216 k l^2 m_2 m l^3 k_3 j l - 3168 k l^2 m_2^3 m l^2 k_3 + 7432 k l^2 m_2^4 m l j l - 3576 k l^2 m_2^4 m l m_3)
\end{aligned}$$

$$\begin{aligned}
& - 64 k l^3 m_2 m l^3 j_3 - 1248 k l^2 m_2^2 m l^2 m_3^2 - 4024 k l^3 m_2^2 j_2 m l^2 - 196 k l^4 m l^2 m_3^2 \\
& + 180 k l^4 m l^2 j l^2 - 32 m l^3 j l^3 m_2^2 - 332 h l^3 m l^3 m_2^2 - 128 m l^2 m_3^2 m_2^4 - 32 m l^3 m_3^3 m_2^2 \\
& + 640 m l^4 j l^2 m_3^2 + 988 k l^3 m l^2 j l^2 m_2 - 2908 k l^3 m_2^2 m l^2 k_3 + 4960 k l^3 m l j l m_2^3 \\
& - 444 k l^8 - 416 k l^5 j_2 m l^2 - 168 k l^5 m l^2 k_3 - 318 k l^6 m l m_3 + 86 k l^6 m l j l \\
& + 492 k l^5 m l j l m_2 + 224 k l^4 m l^2 j l m_3 - 360 k l^3 m l^3 k_3 j l - 2910 k l^4 m l m_3 m_2^2 \\
& + 1790 k l^4 m l j l m_2^2 - 1392 k l^5 m l m_3 m_2 - 888 k l^3 m l^2 j l m_3 m_2 + 80 k l h l m l^3 j l^2 m_2 \\
& - 2152 k l^4 j_2 m l^2 m_2 - 1172 k l^4 m l^2 k_3 m_2 + 340 k l^2 h l m l^3 m_3^2 - 284 k l^2 h l m l^3 j l^2 \\
& - 5578 k l^5 h l m l m_2 - 3153 k l^3 h l^2 m l^2 m_2 - 4052 k l^3 m l m_3 m_2^3 - 980 k l^3 m_2 m l^2 m_3^2 \\
& - 332 k l^3 h l m l^3 k_3 - 156 k l h l^2 m l^4 k_3 - 208 k l^4 h l m l^2 m_3 - 396 k l^4 h l m l^2 j l \\
& - 348 k l h l^2 m l^3 m_3 m_2 - 15308 k l^3 h l m l m_2^3 - 12903 k l^4 h l m l m_2^2 \\
& - 416 k l h l m l^4 k_3 j l - 1516 k l^3 h l m l^2 m_3 m_2 - 1172 k l^3 h l m l^2 j l m_2 \\
& - 1872 k l h l m l^3 j l m_3 m_2 - 15453 k l^4 m_2^4 - 768 k l h l^2 m l^3 j l m_2 \\
& - 3220 k l^2 h l m l^2 m_3 m_2^2 - 5050 k l^2 h l^2 m l^2 m_2^2 + 178 k l^2 h l^2 m l^3 m_3 \\
& - 1464 k l^2 h l m l^3 k_3 m_2 - 176 k l^2 h l m l^2 j l m_2^2 - 520 k l^2 h l m l^3 j l m_3 \\
& - 2112 k l h l m l^3 m_2^2 k_3 + 2032 k l h l m l^2 j l m_2^3 - 468 k l h l^3 m l^3 m_2 - 392 k l^3 h l m l^3 j_2 \\
& - 153 k l^2 h l^3 m l^3 - 2480 k l h l m l^2 m_3 m_2^3 - 160 k l h l m l^3 m_2 m_3^2 \\
& - 1584 k l^2 h l m l^3 j_2 m_2 - 386 k l^2 h l^2 m l^3 j l - 3356 k l h l^2 m l^2 m_2^3 - 32 k l^2 h l m l^4 j_3 \\
& - 9588 k l^2 h l m l m_2^4 - 715 k l^4 h l^2 m l^2 - 983 k l^6 h l m l - 80 k l^4 m l^3 j_3 \\
& - 192 m_2^3 m l^3 j_3 k l - 128 m_2^2 m l^4 j_3 j l + 320 m_2^2 m l^4 j_3 h l + 896 m_2^2 m l^4 j_3 m_3 \\
& + 480 m l^4 m_3^2 j_2 k l + 128 m l^4 m_3^2 j_2 m_2 - 704 m l^4 m_3 m_2 k_3 j l + 320 m l^4 m_3 m_2 k_3 h l \\
& - 192 m l^3 m_3 m_2^3 k_3 - 64 k l m l^3 m_3 m_2^2 k_3 + 224 k l m l^4 m_3 k_3 j l + 192 k l m l^4 m_3 k_3 h l \\
& + 576 m l^4 m_3 m_2 j_3 k l - 1856 m l^3 m_3 m_2^2 j_2 k l - 48 k l^3 m l^3 m_3 j_2 + 104 k l^3 m l^3 m_3 k_3 \\
& - 960 k l^2 m l^3 m_3 j_2 m_2 + 384 k l^2 m l^3 m_3 k_3 m_2 - 64 k l^2 m l^4 m_3 j_3 + 208 k l m l^3 m_3^3 m_2 \\
& + 408 k l^2 m l^3 m_3^3 - 256 h l^2 m l^4 m_2 k_3 - 928 h l m l^3 m_2^3 k_3 - 568 h l^2 m l^3 m_2^2 m_3 \\
& + 256 h l m l^4 m_2 j_3 k l - 2080 h l m l^3 m_2^2 j_2 k l - 512 h l m l^2 m_2^4 m_3 - 464 h l m l^3 m_2^2 m_3^2 \\
& - 736 h l^2 m l^2 m_2^4 - 1504 k l m_2^4 m l^2 k_3 + 80 k l^2 m_2^2 m l^3 j_3 - 624 k l m_2^3 m l^2 m_3^2 \\
& - 3200 k l^2 m_2^3 j_2 m l^2 - 1600 k l m_2^5 m l m_3 - 736 m l^4 j l m_2 k_3 h l - 2976 k l m_2^5 h l m l \\
& + 448 m l^4 j l^2 m_2 k_3 + 192 m l^3 j l m_2^3 k_3 - 280 m l^3 j l m_2^2 h l^2 - 3008 k l^2 m_2^6 \\
& - 1504 m l^3 j l^2 m_2^2 m_3 - 1824 m l^3 j l m_2^2 m_3 h l - 128 h l m l^5 j_3 m_3 - 48 h l m l^5 k_3^2 \\
& - 24 k l j_2 m l^4 h l^2 - 128 k l^2 j_2 m l^4 k_3 + 64 j_2 m l^4 m_2 h l j l - 256 j_2 m l^4 m_2 k l k_3 \\
& - 128 j_2 m l^4 m_2^2 k_3 + 96 k l j_2 m l^4 j l^2 + 256 j_2 m l^4 m_2 j l^2 - 32 j_2 m l^4 m_2 h l^2 \\
& + 304 h l m_3^3 m l^4 - 416 m l^4 j l m_3^3 + 32 h l m l^4 j l m_3^2 - 264 h l^2 m l^4 j l m_3 - 80 h l^3 m l^4 j l \\
& + 4 h l^3 m l^4 m_3 + 240 h l^2 m l^4 m_3^2 + 7 h l^4 m l^4 - 464 m l^4 j l^2 h l m_3 - 136 m l^4 j l^2 h l^2 \\
& + 64 m l^4 j l^3 h l - 224 m l^4 j l^3 m_3 - 768 j_2 m l^3 m_2^3 m_3 - 896 j_2 m l^2 m_2^4 k l \\
& + 256 j_2 m l^3 m_2^3 j l - 896 j_2 m l^3 m_2^3 h l - 272 k l m l^4 k_3^2 m_2 - 48 k l^2 m l^4 k_3^2
\end{aligned}$$

$$\begin{aligned}
& -16 kl ml^4 k3 m3^2 + 128 ml^5 j3 jl m3 + 128 ml^5 j3 m2 k3 + 128 ml^5 j3 kl k3 \\
& + 128 ml^5 j3 hl jl - 448 ml^5 j3 m3^2 + 320 ml^5 j3 jl^2 - 16 ml^5 j3 hl^2 + 96 ml^5 m3 k3^2 \\
& + 128 ml^4 m3^2 m2 k3 + 80 ml^4 m3^4 + 128 f3 ml^6 m3 + 64 f3 ml^5 kl^2 + 128 f3 ml^6 jl \\
& + 192 f3 ml^6 hl - 128 ml^5 k3 m3 j2 - 288 ml^5 k3^2 jl + 192 f3 ml^5 kl m2) / (64 ml^6)
\end{aligned}$$

> **elimsolve (tmp1,f5) ;**

$$\{256 ml^7 \neq 0\}$$

f5 is set to:

$$\begin{aligned}
& - (384 ml^4 m3 j2 kl hl - 128 ml^4 m3 j2 jl m2 - 192 ml^4 m3 j2 jl kl + 256 ml^4 m3 j2 hl m2 \\
& - 80 ml^4 jl^4 - 9348 kl^3 m2^5 - 3013 kl^7 m2 - 8951 kl^6 m2^2 - 15111 kl^5 m2^3 - 64 kl ml^6 \\
& - 384 kl m2^7 + 256 ml^5 m3 j4 m2 + 128 ml^5 m3 j4 kl - 256 ml^6 m3 j5 + 128 m2 j5 ml^5 kl \\
& - 64 m2 j4 ml^4 kl^2 - 256 j4 ml^4 m2^2 kl - 256 m2^4 ml^3 j3 - 256 j4 ml^4 m2^3 + 256 j5 ml^5 m2^2 \\
& + 64 g5 ml^6 kl - 192 m2^2 ml^4 k3^2 - 256 m2^5 ml^2 k3 + 1280 ml jl m2^6 - 256 ml m3 m2^6 \\
& - 384 hl ml m2^6 + 320 ml^4 jl m2 j3 kl + 384 ml^3 jl m2^2 j2 kl + 1280 ml^2 jl^2 m2^4 \\
& + 1344 ml^2 jl m2^4 hl + 1568 ml^3 jl m2^2 m3^2 + 5120 ml jl m2^5 kl + 880 ml^3 jl^2 m2^2 hl \\
& + 632 ml^3 jl kl^2 m3^2 - 192 ml^3 jl^3 kl m2 - 2432 ml^2 jl m2^4 m3 - 208 ml^4 jl^2 kl k3 \\
& + 3600 ml^2 jl^2 kl m2^3 - 176 ml^3 jl kl^3 j2 - 2672 ml^3 jl^2 kl m3 m2 - 248 ml^3 jl^3 kl^2 \\
& - 128 ml^3 jl kl^2 j2 m2 - 608 ml^3 jl kl m2^2 k3 - 7072 ml^2 jl kl m3 m2^3 \\
& + 2848 ml^3 jl kl m2 m3^2 + 3048 kl^2 m2^2 ml^2 jl^2 + 192 ml^4 jl kl^2 j3 - 600 ml^3 jl^2 kl^2 m3 \\
& - 5704 kl^2 m2^2 ml^2 jl m3 - 1216 kl^2 m2 ml^3 k3 jl - 3168 kl^2 m2^3 ml^2 k3 \\
& + 7432 kl^2 m2^4 ml jl - 3576 kl^2 m2^4 ml m3 - 64 kl^3 m2 ml^3 j3 - 1248 kl^2 m2^2 ml^2 m3^2 \\
& - 4024 kl^3 m2^2 j2 ml^2 - 196 kl^4 ml^2 m3^2 + 180 kl^4 ml^2 jl^2 - 32 ml^3 jl^3 m2^2 \\
& - 332 hl^3 ml^3 m2^2 - 128 ml^2 m3^2 m2^4 - 32 ml^3 m3^3 m2^2 + 640 ml^4 jl^2 m3^2 \\
& + 988 kl^3 ml^2 jl^2 m2 - 2908 kl^3 m2^2 ml^2 k3 + 4960 kl^3 ml jl m2^3 - 444 kl^8 - 416 kl^5 j2 ml^2 \\
& - 168 kl^5 ml^2 k3 - 318 kl^6 ml m3 + 86 kl^6 ml jl + 492 kl^5 ml jl m2 + 224 kl^4 ml^2 jl m3 \\
& - 360 kl^3 ml^3 k3 jl - 2910 kl^4 ml m3 m2^2 + 1790 kl^4 ml jl m2^2 - 1392 kl^5 ml m3 m2 \\
& - 888 kl^3 ml^2 jl m3 m2 + 80 kl hl ml^3 jl^2 m2 - 2152 kl^4 j2 ml^2 m2 - 1172 kl^4 ml^2 k3 m2 \\
& + 340 kl^2 hl ml^3 m3^2 - 284 kl^2 hl ml^3 jl^2 - 5578 kl^5 hl ml m2 - 3153 kl^3 hl^2 ml^2 m2 \\
& - 4052 kl^3 ml m3 m2^3 - 980 kl^3 m2 ml^2 m3^2 - 332 kl^3 hl ml^3 k3 - 156 kl hl^2 ml^4 k3 \\
& - 208 kl^4 hl ml^2 m3 - 396 kl^4 hl ml^2 jl - 348 kl hl^2 ml^3 m3 m2 - 15308 kl^3 hl ml m2^3 \\
& - 12903 kl^4 hl ml m2^2 - 416 kl hl ml^4 k3 jl - 1516 kl^3 hl ml^2 m3 m2 \\
& - 1172 kl^3 hl ml^2 jl m2 - 1872 kl hl ml^3 jl m3 m2 - 15453 kl^4 m2^4 - 768 kl hl^2 ml^3 jl m2 \\
& - 3220 kl^2 hl ml^2 m3 m2^2 - 5050 kl^2 hl^2 ml^2 m2^2 + 178 kl^2 hl^2 ml^3 m3 \\
& - 1464 kl^2 hl ml^3 k3 m2 - 176 kl^2 hl ml^2 jl m2^2 - 520 kl^2 hl ml^3 jl m3 \\
& - 2112 kl hl ml^3 m2^2 k3 + 2032 kl hl ml^2 jl m2^3 - 468 kl hl^3 ml^3 m2 - 392 kl^3 hl ml^3 j2 \\
& - 153 kl^2 hl^3 ml^3 - 2480 kl hl ml^2 m3 m2^3 - 160 kl hl ml^3 m2 m3^2 \\
& - 1584 kl^2 hl ml^3 j2 m2 - 386 kl^2 hl^2 ml^3 jl - 3356 kl hl^2 ml^2 m2^3 - 32 kl^2 hl ml^4 j3
\end{aligned}$$

$$\begin{aligned}
& -9588 k l^2 h l m l m 2^4 - 715 k l^4 h l^2 m l^2 - 983 k l^6 h l m l - 80 k l^4 m l^3 j 3 \\
& - 192 m 2^3 m l^3 j 3 k l - 128 m 2^2 m l^4 j 3 j l + 320 m 2^2 m l^4 j 3 h l + 896 m 2^2 m l^4 j 3 m 3 \\
& + 480 m l^4 m 3^2 j 2 k l + 128 m l^4 m 3^2 j 2 m 2 - 704 m l^4 m 3 m 2 k 3 j l + 320 m l^4 m 3 m 2 k 3 h l \\
& - 192 m l^3 m 3 m 2^3 k 3 - 64 k l m l^3 m 3 m 2^2 k 3 + 224 k l m l^4 m 3 k 3 j l + 192 k l m l^4 m 3 k 3 h l \\
& + 576 m l^4 m 3 m 2 j 3 k l - 1856 m l^3 m 3 m 2^2 j 2 k l - 48 k l^3 m l^3 m 3 j 2 + 104 k l^3 m l^3 m 3 k 3 \\
& - 960 k l^2 m l^3 m 3 j 2 m 2 + 384 k l^2 m l^3 m 3 k 3 m 2 - 64 k l^2 m l^4 m 3 j 3 + 208 k l m l^3 m 3^3 m 2 \\
& + 408 k l^2 m l^3 m 3^3 - 256 h l^2 m l^4 m 2 k 3 - 928 h l m l^3 m 2^3 k 3 - 568 h l^2 m l^3 m 2^2 m 3 \\
& + 256 h l m l^4 m 2 j 3 k l - 2080 h l m l^3 m 2^2 j 2 k l - 512 h l m l^2 m 2^4 m 3 - 464 h l m l^3 m 2^2 m 3^2 \\
& - 736 h l^2 m l^2 m 2^4 - 1504 k l m 2^4 m l^2 k 3 + 80 k l^2 m 2^2 m l^3 j 3 - 624 k l m 2^3 m l^2 m 3^2 \\
& - 3200 k l^2 m 2^3 j 2 m l^2 - 1600 k l m 2^5 m l m 3 - 736 m l^4 j l m 2 k 3 h l - 2976 k l m 2^5 h l m l \\
& + 448 m l^4 j l^2 m 2 k 3 + 192 m l^3 j l m 2^3 k 3 - 280 m l^3 j l m 2^2 h l^2 - 3008 k l^2 m 2^6 \\
& - 1504 m l^3 j l^2 m 2^2 m 3 - 1824 m l^3 j l m 2^2 m 3 h l - 128 h l m l^5 j 3 m 3 - 48 h l m l^5 k 3^2 \\
& - 24 k l j 2 m l^4 h l^2 - 128 k l^2 j 2 m l^4 k 3 + 64 j 2 m l^4 m 2 h l j l - 256 j 2 m l^4 m 2 k l k 3 \\
& - 128 j 2 m l^4 m 2^2 k 3 + 96 k l j 2 m l^4 j l^2 + 256 j 2 m l^4 m 2 j l^2 - 32 j 2 m l^4 m 2 h l^2 \\
& + 304 h l m 3^3 m l^4 - 416 m l^4 j l m 3^3 + 32 h l m l^4 j l m 3^2 - 264 h l^2 m l^4 j l m 3 - 80 h l^3 m l^4 j l \\
& + 4 h l^3 m l^4 m 3 + 240 h l^2 m l^4 m 3^2 + 7 h l^4 m l^4 - 464 m l^4 j l^2 h l m 3 - 136 m l^4 j l^2 h l^2 \\
& + 64 m l^4 j l^3 h l - 224 m l^4 j l^3 m 3 - 768 j 2 m l^3 m 2^3 m 3 - 896 j 2 m l^2 m 2^4 k l \\
& + 256 j 2 m l^3 m 2^3 j l - 896 j 2 m l^3 m 2^3 h l - 272 k l m l^4 k 3^2 m 2 - 48 k l^2 m l^4 k 3^2 \\
& - 16 k l m l^4 k 3 m 3^2 + 128 m l^5 j 3 j l m 3 + 128 m l^5 j 3 m 2 k 3 + 128 m l^5 j 3 k l k 3 \\
& + 128 m l^5 j 3 h l j l - 448 m l^5 j 3 m 3^2 + 320 m l^5 j 3 j l^2 - 16 m l^5 j 3 h l^2 + 96 m l^5 m 3 k 3^2 \\
& + 128 m l^4 m 3^2 m 2 k 3 + 80 m l^4 m 3^4 + 128 f 3 m l^6 m 3 + 64 f 3 m l^5 k l^2 + 128 f 3 m l^6 j l \\
& + 192 f 3 m l^6 h l - 128 m l^5 k 3 m 3 j 2 - 288 m l^5 k 3^2 j l + 192 f 3 m l^5 k l m 2) / (256 m l^7)
\end{aligned}$$

> **launchNZcase** **(-k1^2+4\*m1\*j1);**

Launching case level 2:

$$-k l^2 + 4 m l j l \neq 0$$

Assume from now on that:

$$2 m l (-k l^2 + 4 m l j l) \neq 0$$

> **tmp1 := cpcoeff(x1^3\*x3^2);**

$$\begin{aligned}
tmp1 := & -(-k l^2 + 4 m l j l) (-12 m l j l m 2 - 10 m l j l k l + 8 j 2 m l^2 + 4 m l^2 k 3 + 9 k l h l m l \\
& + 2 k l m l m 3 + 6 h l m l m 2 + 4 m l m 3 m 2 + 6 k l m 2^2 + 7 k l^3 + 13 k l^2 m 2) / (8 m l^3)
\end{aligned}$$

> **elimsolve** **(tmp1,k3);**

$$\{4 m l^2 \neq 0\}$$

k3 is set to:

$$\begin{aligned}
& -(-12 m l j l m 2 - 10 m l j l k l + 8 j 2 m l^2 + 9 k l h l m l + 2 k l m l m 3 + 6 h l m l m 2 \\
& + 4 m l m 3 m 2 + 6 k l m 2^2 + 7 k l^3 + 13 k l^2 m 2) / (4 m l^2)
\end{aligned}$$

> **launchNZcase** **(2\*m1\*m3+3\*k1^2+h1\*m1-2\*m1\*j1+3\*k1\*m2);**

Launching case level 3:

$$2 m l m 3 + 3 k l^2 + h l m l - 2 m l j l + 3 k l m 2 \neq 0$$

Assume from now on that:

$$2ml(-kl^2 + 4mljl)(2mlm3 + 3kl^2 + hlml - 2mljl + 3klm2) \neq 0$$

> **tmp1 := cpcoeff(x4^3\*x5^2);**

$$tmp1 := (-kl^2 + 4mljl)(-4ml^2jl^2 - 8hlml^2jl - 16mljl m2^2 - 40mljl kl m2 - 22mljl kl^2 + hl^2ml^2 + 4hl m3 ml^2 + 4ml^2 m3^2 + 10kl^2 ml m3 + 12kl ml m3 m2 + 7kl^2 hl ml + 6kl hl ml m2 + 13kl^2 m2^2 + 12kl^4 + 25kl^3 m2) / (4ml^2)$$

> **tmp2 := cpcoeff(x5^3\*T^2);**

$$tmp2 := -(2ml m3 + 3kl^2 + hlml - 2mljl + 3kl m2)(-12ml^2jl^2 - 12hlml^2jl + 8ml^2jl m3 - 32mljl kl^2 - 32mljl m2^2 - 68mljl kl m2 + hl^2ml^2 + 4hl m3 ml^2 + 4ml^2 m3^2 + 12kl ml m3 m2 + 8kl^2 hl ml + 8kl^2 ml m3 + 6kl hl ml m2 + 32kl^3 m2 + 17kl^2 m2^2 + 15kl^4) / (8ml^3)$$

> **tmp3 := factor((2\*ml\*m3+3\*k1^2+hl\*ml-2\*ml\*j1+3\*k1\*m2)\*tmp1 + m1\*(-k1^2+4\*ml\*j1)\*tmp2);**

$$tmp3 := \frac{(2ml m3 + 3kl^2 + hlml - 2mljl + 3kl m2)^3 (-kl^2 + 4mljl)}{8ml^2}$$

> **contradict(tmp3, 'h1');**

Contradiction on case level 3, so:

$$2ml m3 + 3kl^2 + hlml - 2mljl + 3kl m2 = 0$$

Proceed on case level 2 with:

$$2ml(-kl^2 + 4mljl) \neq 0$$

On account of:

$$2ml m3 + 3kl^2 + hlml - 2mljl + 3kl m2 = 0$$

$$\{ml \neq 0\}$$

h1 is set to:

$$\frac{-2ml m3 - 3kl^2 + 2mljl - 3kl m2}{ml}$$

> **tmp1 := cpcoeff(x4^3\*x5^2);**

$$tmp1 := -\frac{(-kl^2 + 4mljl)^2 (mljl - ml m3 + kl m2 + m2^2)}{ml^2}$$

> **elimsolve(tmp1, m3);**

$$\{-ml \neq 0\}$$

m3 is set to:

$$\frac{mljl + kl m2 + m2^2}{ml}$$

> **tmp1 := cpcoeff(x4^4\*x5);**

$$tmp1 := -\frac{(-kl^2 + 4mljl)^2 (3mljl kl + 3mljl m2 - j2 ml^2 + 2kl^2 m2 + kl m2^2 + kl^3)}{ml^3}$$

> **elimsolve(tmp1, j2);**

$$\{-ml^2 \neq 0\}$$

j2 is set to:



$$\frac{(kl + m2)(kl^2 + kl\ m2 + 3\ ml\ j1)}{ml^2}$$

> **tmp1 := cpcoeff (x1\*x3\*x4\*T^2);**

$$tmp1 := -\frac{2(2\ m2^2\ j3 - 2\ j5\ ml^2 + 3\ j3\ kl^2 + 5\ m2\ j3\ kl - j4\ ml\ kl)}{ml}$$

> **elimsolve (tmp1, j5);**

$$\{-2\ ml^2 \neq 0\}$$

j5 is set to:

$$\frac{2\ m2^2\ j3 + 3\ j3\ kl^2 + 5\ m2\ j3\ kl - j4\ ml\ kl}{2\ ml^2}$$

> **tmp1 := cpcoeff (x1^2\*x4^2\*x5);**

$$tmp1 := -2(-kl^2 + 4\ ml\ j1)(4\ ml\ j1\ m2^2 + 4\ ml\ j1\ kl^2 + 8\ ml\ j1\ kl\ m2 - ml^3\ j3 + 12\ kl^2\ m2^2 + 10\ kl^3\ m2 + m2^4 + 3\ kl^4 + 6\ kl\ m2^3) / ml^3$$

> **elimsolve (tmp1, j3);**

$$\{-ml^3 \neq 0\}$$

j3 is set to:

$$\frac{(kl + m2)^2(3\ kl^2 + 4\ kl\ m2 + 4\ ml\ j1 + m2^2)}{ml^3}$$

> **tmp1 := cpcoeff (x1\*x4^2\*x5\*T);**

$$tmp1 := -4\ ml^2$$

> **contradict (tmp1, 'j1');**

Contradiction on case level 2, so:

$$-kl^2 + 4\ ml\ j1 = 0$$

Variables to be uneliminated:

"j3 := 'j3'"

"j5 := 'j5'"

"j2 := 'j2'"

"m3 := 'm3'"

"h1 := 'h1'"

"k3 := 'k3'"

Proceed on case level 1 with:

$$2\ ml \neq 0$$

On account of:

$$-kl^2 + 4\ ml\ j1 = 0$$

$$\{4\ ml \neq 0\}$$

j1 is set to:

$$\frac{kl^2}{4\ ml}$$

> **tmp1 := cpcoeff (x5^3\*T^2);**

$$tmp1 := -\frac{(2\ h1\ ml + 4\ ml\ m3 + 6\ kl\ m2 + 5\ kl^2)^3}{64\ ml^3}$$

> **elimsolve (tmp1,h1);**

$$\{2\,m\,l \neq 0\}$$

h1 is set to:

$$-\frac{4\,m\,l\,m^3+6\,k\,l\,m^2+5\,k\,l^2}{2\,m\,l}$$

> **tmp1 := cpcoeff(x1\*x3\*x5^2\*T);**

$$\begin{aligned} tmp1 := & -(-480\,k\,l^3\,j_2\,m\,l^2\,m^2 - 136\,k\,l^4\,j_2\,m\,l^2 + 3728\,m\,l\,m^3\,k\,l^4\,m^2 + 601\,k\,l^7 \\ & + 4356\,k\,l^5\,m^2 + 688\,m\,l^2\,m^3\,k\,l^3 + 128\,m\,l^3\,m^3\,j_2\,k\,l^2 - 304\,m\,l^3\,m^3\,k^3\,k\,l^2 \\ & + 192\,m\,l^3\,m^3\,k\,l + 4064\,m\,l\,m^3\,k\,l^3\,m^2 + 960\,m\,l\,m^3\,k\,l^2\,m^2 + 144\,k\,l^3\,m^2 \\ & + 1792\,m\,l^2\,m^3\,k\,l^2\,m^2 - 64\,g_5\,m\,l^6 - 544\,k\,l^2\,m^2\,j_2\,m\,l^2 + 2712\,k\,l^6\,m^2 + 32\,k\,l^2\,m^2\,m\,l^3\,j_3 \\ & + 2680\,k\,l^4\,m^2 + 960\,k\,l\,m\,l^2\,m^3\,m^2 - 352\,k\,l^3\,m^2\,m\,l^2\,k^3 + 96\,k\,l\,m^2\,m\,l^2\,k^3 \\ & - 80\,k\,l^2\,m^2\,m\,l^2\,k^3 - 192\,j_2\,m\,l^2\,m^2\,k\,l - 128\,j_2\,m\,l^3\,m^2\,m^3 - 288\,k\,l\,m\,l^3\,m^3\,m^2\,k^3 \\ & + 256\,m\,l^3\,m^3\,m^2 - 180\,k\,l^4\,m\,l^2\,k^3 + 32\,k\,l^3\,m\,l^3\,j_3 + 1028\,m\,l\,m^3\,k\,l^5 + 128\,m\,l^4\,m^3\,j_2 \\ & + 64\,m\,l^3\,m^3\,m^2\,k^3 - 128\,m^2\,m\,l^2\,m^3\,m^2 - 32\,j_4\,m\,l^4\,k\,l^2 - 384\,k\,l\,m\,l\,m^3\,m^2 + 16\,k\,l\,m\,l^4\,k^3 \\ & - 128\,m\,l^4\,k^3\,m^3 + 32\,j_2\,m\,l^4\,k\,l\,k^3 - 288\,k\,l^2\,m^2 - 192\,j_5\,m\,l^5\,k\,l - 128\,j_5\,m\,l^5\,m^2) / (16 \\ & m\,l^4) \end{aligned}$$

> **elimsolve (tmp1,g5);**

$$\{-64\,m\,l^6 \neq 0\}$$

g5 is set to:

$$\begin{aligned} & (-480\,k\,l^3\,j_2\,m\,l^2\,m^2 - 136\,k\,l^4\,j_2\,m\,l^2 + 3728\,m\,l\,m^3\,k\,l^4\,m^2 + 601\,k\,l^7 + 4356\,k\,l^5\,m^2 \\ & + 688\,m\,l^2\,m^3\,k\,l^3 + 128\,m\,l^3\,m^3\,j_2\,k\,l^2 - 304\,m\,l^3\,m^3\,k^3\,k\,l^2 + 192\,m\,l^3\,m^3\,k\,l \\ & + 4064\,m\,l\,m^3\,k\,l^3\,m^2 + 960\,m\,l\,m^3\,k\,l^2\,m^2 + 144\,k\,l^3\,m^2 + 1792\,m\,l^2\,m^3\,k\,l^2\,m^2 \\ & - 544\,k\,l^2\,m^2\,j_2\,m\,l^2 + 2712\,k\,l^6\,m^2 + 32\,k\,l^2\,m^2\,m\,l^3\,j_3 + 2680\,k\,l^4\,m^2 \\ & + 960\,k\,l\,m\,l^2\,m^3\,m^2 - 352\,k\,l^3\,m^2\,m\,l^2\,k^3 + 96\,k\,l\,m^2\,m\,l^2\,k^3 - 80\,k\,l^2\,m^2\,m\,l^2\,k^3 \\ & - 192\,j_2\,m\,l^2\,m^2\,k\,l - 128\,j_2\,m\,l^3\,m^2\,m^3 - 288\,k\,l\,m\,l^3\,m^3\,m^2\,k^3 + 256\,m\,l^3\,m^3\,m^2 \\ & - 180\,k\,l^4\,m\,l^2\,k^3 + 32\,k\,l^3\,m\,l^3\,j_3 + 1028\,m\,l\,m^3\,k\,l^5 + 128\,m\,l^4\,m^3\,j_2 + 64\,m\,l^3\,m^3\,m^2\,k^3 \\ & - 128\,m^2\,m\,l^2\,m^3\,m^2 - 32\,j_4\,m\,l^4\,k\,l^2 - 384\,k\,l\,m\,l\,m^3\,m^2 + 16\,k\,l\,m\,l^4\,k^3 - 128\,m\,l^4\,k^3\,m^3 \\ & + 32\,j_2\,m\,l^4\,k\,l\,k^3 - 288\,k\,l^2\,m^2 - 192\,j_5\,m\,l^5\,k\,l - 128\,j_5\,m\,l^5\,m^2) / (64\,m\,l^6) \end{aligned}$$

> **tmp1 := cpcoeff(x1\*x2\*x5\*T^2);**

$$\begin{aligned} tmp1 := & (-16\,j_2\,m\,l^2\,k\,l^3 - 128\,m^2\,m\,l^3\,j_3 - 80\,j_2\,m\,l^2\,k\,l^2\,m^2 + 64\,j_2\,m\,l^3\,m^3\,m^2 \\ & + 64\,j_2\,m\,l^3\,k\,l\,m^3 - 128\,j_2\,m\,l^2\,k\,l\,m^2 + 225\,k\,l^6 + 32\,m\,l^3\,m^3\,m^2\,k^3 + 224\,m\,l\,m^3\,k\,l^3\,m^2 \\ & + 976\,m\,l\,m^3\,k\,l^2\,m^2 - 320\,m\,l^2\,m^3\,k\,l\,m^2 - 96\,m\,l\,m^3\,k\,l^4 + 24\,k\,l^2\,m^2\,m\,l^2\,k^3 \\ & - 368\,m\,l^2\,m^3\,k\,l^2 + 2324\,k\,l^4\,m^2 - 128\,m\,l^3\,m^3 + 2168\,k\,l^3\,m^2 + 1164\,k\,l^5\,m^2 \\ & + 880\,k\,l^2\,m^2 - 80\,m\,l^3\,j_3\,k\,l^2 + 96\,k\,l\,m^2 - 192\,m^2\,m\,l^3\,j_3\,k\,l + 736\,k\,l\,m\,l\,m^3\,m^2 \\ & + 128\,m^2\,m\,l^2\,m^3 + 64\,m\,l\,m^3\,m^2 - 16\,m\,l^4\,k^3 - 32\,m^2\,m\,l^2\,k^3 + 64\,m\,l^4\,j_3\,m^3 \\ & - 64\,j_2\,m\,l^2\,m^2 + 64\,f_3\,m\,l^5) / (16\,m\,l^4) \end{aligned}$$

> **elimsolve (tmp1, f3);**

$$\{64 m l^5 \neq 0\}$$

f3 is set to:

$$\begin{aligned} & -(-16 j_2 m l^2 k l^3 - 128 m^2 m l^3 j_3 - 80 j_2 m l^2 k l^2 m_2 + 64 j_2 m l^3 m_3 m_2 + 64 j_2 m l^3 k l m_3 \\ & - 128 j_2 m l^2 k l m_2^2 + 225 k l^6 + 32 m l^3 m_3 m_2 k_3 + 224 m l m_3 k l^3 m_2 + 976 m l m_3 k l^2 m_2^2 \\ & - 320 m l^2 m_3^2 k l m_2 - 96 m l m_3 k l^4 + 24 k l^2 m_2 m l^2 k_3 - 368 m l^2 m_3^2 k l^2 + 2324 k l^4 m_2^2 \\ & - 128 m l^3 m_3^3 + 2168 k l^3 m_2^3 + 1164 k l^5 m_2 + 880 k l^2 m_2^4 - 80 m l^3 j_3 k l^2 + 96 k l m_2^5 \\ & - 192 m_2 m l^3 j_3 k l + 736 k l m l m_3 m_2^3 + 128 m^2 m l^2 m_3^2 + 64 m l m_3 m_2^4 - 16 m l^4 k_3^2 \\ & - 32 m_2^3 m l^2 k_3 + 64 m l^4 j_3 m_3 - 64 j_2 m l^2 m_2^3) / (64 m l^5) \end{aligned}$$

> **launchNZcase** (4\*m2^2+k1^2+4\*k1\*m2-4\*m1\*m3) ;

Launching case level 2:

$$4 m_2^2 + k l^2 + 4 k l m_2 - 4 m l m_3 \neq 0$$

Assume from now on that:

$$2 m l (4 m_2^2 + k l^2 + 4 k l m_2 - 4 m l m_3) \neq 0$$

> **tmp1 := cpcoeff(x1\*x3\*x5\*T^2) ;**

$$tmp1 := (4 m_2^2 + k l^2 + 4 k l m_2 - 4 m l m_3)$$

$$(3 k l^3 - 2 k l^2 m_2 - 6 k l m_2^2 - 4 m l m_3 m_2 - 4 j_2 m l^2 + 2 m l^2 k_3) / (4 m l^3)$$

> **elimsolve** (tmp1,j2) ;

$$\{-4 m l^2 \neq 0\}$$

j2 is set to:

$$\frac{3 k l^3 - 2 k l^2 m_2 - 6 k l m_2^2 - 4 m l m_3 m_2 + 2 m l^2 k_3}{4 m l^2}$$

> **tmp1 := cpcoeff(x1^2\*x3^2\*T) ;**

$$tmp1 := - \frac{(3 k l^3 + 9 k l^2 m_2 + 6 k l m_2^2 - 2 m l^2 k_3 + 4 k l m l m_3 + 4 m l m_3 m_2)^2}{2 m l^4}$$

> **elimsolve** (tmp1,k3) ;

$$\{-2 m l^2 \neq 0\}$$

k3 is set to:

$$\frac{(k l + m_2) (3 k l^2 + 6 k l m_2 + 4 m l m_3)}{2 m l^2}$$

> **tmp1 := cpcoeff(x1^2\*x2\*x4\*T) ;**

$$tmp1 := -(4 m_2^2 + k l^2 + 4 k l m_2 - 4 m l m_3)$$

$$(12 k l^4 + 27 k l^3 m_2 + 15 k l^2 m l m_3 + 15 k l^2 m_2^2 + 16 k l m l m_3 m_2 + 4 m l^2 m_3^2 - 4 m l^3 j_3) / (4 m l^4)$$

> **elimsolve** (tmp1,j3) ;

$$\{-4 m l^3 \neq 0\}$$

j3 is set to:

$$\frac{12 k l^4 + 27 k l^3 m_2 + 15 k l^2 m l m_3 + 15 k l^2 m_2^2 + 16 k l m l m_3 m_2 + 4 m l^2 m_3^2}{4 m l^3}$$

> **tmp1 := cpcoeff(x1^2\*x4^3) ;**

$$tmp1 := 4 m1^2$$

> **contradict** (tmp1, 'm3');

Contradiction on case level 2, so:

$$4 m2^2 + k1^2 + 4 k1 m2 - 4 m1 m3 = 0$$

Variables to be uneliminated:

$$j3 := j3$$

$$k3 := k3$$

$$j2 := j2$$

Proceed on case level 1 with:

$$2 m1 \neq 0$$

On account of:

$$4 m2^2 + k1^2 + 4 k1 m2 - 4 m1 m3 = 0$$

$$\{-4 m1 \neq 0\}$$

m3 is set to:

$$\frac{(k1 + 2 m2)^2}{4 m1}$$

> **tmp1 := cpcoeff** (x1^2\*x4^2\*x5);

$$tmp1 := -\frac{2 (-m1^2 k3 + 2 k1^3 + 7 k1^2 m2 + 7 k1 m2^2 + 2 m2^3)^2}{m1^3}$$

> **elimsolve** (tmp1, k3);

$$\{-m1^2 \neq 0\}$$

k3 is set to:

$$\frac{(k1 + 2 m2) (m2 + 2 k1) (k1 + m2)}{m1^2}$$

> **tmp1 := cpcoeff** (x1\*x4^2\*x5\*T);

$$tmp1 := -4 m1^2$$

> **contradict** (tmp1);

Contradiction on case level 1, so:

$$m1 = 0$$

Variables to be uneliminated:

$$k3 := k3$$

$$m3 := m3$$

$$f3 := f3$$

$$g5 := g5$$

$$h1 := h1$$

$$j1 := j1$$

$$f5 := f5$$

$$f4 := f4$$

$$h5 := h5$$

$$g4 := g4$$

$$h4 := h4$$

$$k5 := k5$$

"f2 := 'f2'"

"g3 := 'g3'"

"h3 := 'h3'"

"g2 := 'g2'"

"k4 := 'k4'"

"m5 := 'm5'"

"h2 := 'h2'"

"m4 := 'm4'"

"f1 := 'f1'"

"g1 := 'g1'"

"k2 := 'k2'"

Proceed on case level 0 with:

$$2 \neq 0$$

On account of:

$$m1 = 0$$

$$\{1 \neq 0\}$$

m1 is set to:

$$0$$

> **launchNZcase (k1);**

Launching case level 1:

$$k1 \neq 0$$

Assume from now on that:

$$2 k1 \neq 0$$

> **tmp1 := cpcoeff(x1^2\*x5^2\*T);**

$$tmp1 := -2 k1 (k1 + m2)$$

> **elimsolve (tmp1,m2);**

$$\{1 \neq 0\}$$

m2 is set to:

$$-k1$$

> **tmp1 := cpcoeff(x1\*x5^2\*T^2);**

$$tmp1 := k1 (2 m3 + k2)$$

> **elimsolve (tmp1,k2);**

$$\{1 \neq 0\}$$

k2 is set to:

$$-2 m3$$

> **tmp1 := cpcoeff(x1^2\*x4\*x5\*T);**

$$tmp1 := -2 k1 (-m3 + j1 + h1)$$

> **elimsolve (tmp1,m3);**

$$\{-1 \neq 0\}$$

m3 is set to:

$$j1 + h1$$

> **tmp1 := cpcoeff(x1\*x4\*x5\*T^2);**

$$tmp1 := -k1 (-h2 + 2 g1 + 2 j2)$$

```
> elimsolve (tmp1,h2);
```

$$\{-1 \neq 0\}$$

h2 is set to:

$$2\,g1 + 2\,j2$$

```
> tmp1 := cpcoeff(x1^2*x3*x5*T);
```

$$tmp1 := -2\,kl\,m4 - 2\,hl\,j1 - 2\,hl^2$$

```
> elimsolve (tmp1,m4);
```

$$\{kl \neq 0\}$$

m4 is set to:

$$-\frac{hl\,(j1 + hl)}{kl}$$

```
> tmp1 := cpcoeff(x5^2*T^3);
```

$$tmp1 := -2\,kl\,g1 - 3\,hl^2 + kl\,k3$$

```
> elimsolve (tmp1,k3);
```

$$\{-kl \neq 0\}$$

k3 is set to:

$$\frac{2\,kl\,g1 + 3\,hl^2}{kl}$$

```
> tmp1 := cpcoeff(x5^3*T^2);
```

$$tmp1 := hl^3 - 2\,kl^2\,f1 - kl^2\,h3 - kl^2\,g2$$

```
> elimsolve (tmp1,h3);
```

$$\{kl^2 \neq 0\}$$

h3 is set to:

$$-\frac{-hl^3 + 2\,kl^2\,f1 + kl^2\,g2}{kl^2}$$

```
> tmp1 := cpcoeff(x1^2*x4^2*T);
```

$$tmp1 := 6\,kl\,g1 + 4\,j2\,kl + 2\,hl^2$$

```
> elimsolve (tmp1,j2);
```

$$\{2\,kl \neq 0\}$$

j2 is set to:

$$-\frac{3\,kl\,g1 + hl^2}{2\,kl}$$

```
> tmp1 := cpcoeff(x1^2*x2*x5*T);
```

$$tmp1 := \frac{2\,(-hl\,kl\,g1 + hl^2\,j1 + kl^2\,f1)}{kl}$$

```
> elimsolve (tmp1,f1);
```

$$\{kl^2 \neq 0\}$$

f1 is set to:

$$\frac{hl\,(kl\,g1 - hl\,j1)}{kl^2}$$

```
> tmp1 := cpcoeff(x4*x5*T^3);
```

$$tmp1 := -\frac{2(4hlklgl - 4hl^2jl + 2hl^3 - j3kl^2)}{kl}$$

> **elimsolve** (tmp1,j3);

$$\{-kl^2 \neq 0\}$$

j3 is set to:

$$\frac{2hl(2klgl - 2hljl + hl^2)}{kl^2}$$

> **tmp1 := cpcoeff**(x1\*x3\*x5\*T^2);

$$tmp1 := -\frac{2(2hlklgl + 3hl^3 + k4kl^2)}{kl}$$

> **elimsolve** (tmp1,k4);

$$\{kl^2 \neq 0\}$$

k4 is set to:

$$-\frac{hl(2klgl + 3hl^2)}{kl^2}$$

> **tmp1 := cpcoeff**(x1^3\*x3^2);

$$tmp1 := -\frac{-4hl^2jl + 4hlklgl + hl^3 + kl^2g2}{kl}$$

> **elimsolve** (tmp1,g2);

$$\{kl^2 \neq 0\}$$

g2 is set to:

$$-\frac{hl(-4hljl + 4klgl + hl^2)}{kl^2}$$

> **tmp1 := cpcoeff**(x1^2\*x4^3);

$$tmp1 := -\frac{h4kl^3 + 2hl^4 + 2hl^2klgl - 2hl^3jl}{kl}$$

> **elimsolve** (tmp1,h4);

$$\{kl^3 \neq 0\}$$

h4 is set to:

$$-\frac{2hl^2(hl^2 + klgl - hljl)}{kl^3}$$

> **tmp1 := cpcoeff**(x4^4\*T);

$$tmp1 := -kl(klgl + hl^2 - 2hljl)$$

> **elimsolve** (tmp1,g1);

$$\{kl \neq 0\}$$

g1 is set to:

$$-\frac{hl(hl - 2jl)}{kl}$$

> **tmp1 := cpcoeff**(x1\*x2\*x5\*T^2);

$$tmp1 := -\frac{2(-hl^3 jl + hl^4 - f2 kl^3)}{kl^2}$$

> **elimsolve** (tmp1,f2);

$$\{-kl^3 \neq 0\}$$

f2 is set to:

$$\frac{hl^3(hl - jl)}{kl^3}$$

> **tmp1** := **cpcoeff**(x3\*x5\*T^3);

$$tmp1 := \frac{2(2hl^4 - 4hl^3 jl - j4 kl^3)}{kl^2}$$

> **elimsolve** (tmp1,j4);

$$\{-kl^3 \neq 0\}$$

j4 is set to:

$$\frac{2hl^3(hl - 2jl)}{kl^3}$$

> **tmp1** := **cpcoeff**(x4\*x5^2\*T^2);

$$tmp1 := -\frac{3hl^4 + g3 kl^3 - 4hl^3 jl}{kl}$$

> **elimsolve** (tmp1,g3);

$$\{kl^3 \neq 0\}$$

g3 is set to:

$$-\frac{hl^3(-4jl + 3hl)}{kl^3}$$

> **tmp1** := **cpcoeff**(x3\*x5^2\*T^2);

$$tmp1 := -\frac{-4hl^4 jl + 3hl^5 - g4 kl^4}{kl^2}$$

> **elimsolve** (tmp1,g4);

$$\{-kl^4 \neq 0\}$$

g4 is set to:

$$\frac{hl^4(-4jl + 3hl)}{kl^4}$$

> **tmp1** := **cpcoeff**(x2\*x5^2\*T^2);

$$tmp1 := 2kl(f4 kl + f3 hl)$$

> **elimsolve** (tmp1,f4);

$$\{kl \neq 0\}$$

f4 is set to:

$$-\frac{f3 hl}{kl}$$

> **tmp1** := **cpcoeff**(x1\*x4^2\*T^2);



$$tmp1 := \frac{2(hl^3 + hl^2 j1 - kl^2 m5)}{kl}$$

> **elimsolve** (tmp1,m5);

$$\{-kl^2 \neq 0\}$$

m5 is set to:

$$\frac{(j1 + hl) hl^2}{kl^2}$$

> **tmp1 := cpcoeff**(x2\*x5\*T^3);

$$tmp1 := \frac{2(hl^5 - hl^4 j1 + f3 kl^4)}{kl^3}$$

> **elimsolve** (tmp1,f3);

$$\{kl^4 \neq 0\}$$

f3 is set to:

$$-\frac{hl^4 (hl - j1)}{kl^4}$$

> **tmp1 := cpcoeff**(x4^2\*T^3);

$$tmp1 := \frac{hl^4 + 4 hl^3 j1 - k5 kl^3}{kl^2}$$

> **elimsolve** (tmp1,k5);

$$\{-kl^3 \neq 0\}$$

k5 is set to:

$$\frac{hl^3 (hl + 4 j1)}{kl^3}$$

> **tmp1 := cpcoeff**(x1\*x2\*x4\*T^2);

$$tmp1 := \frac{-kl^4 h5 + 2 hl^4 j1}{kl^3}$$

> **elimsolve** (tmp1,h5);

$$\{-kl^4 \neq 0\}$$

h5 is set to:

$$\frac{2 hl^4 j1}{kl^4}$$

> **tmp1 := cpcoeff**(x4^3\*T^2);

$$tmp1 := -kl^2$$

> **contradict** (tmp1);

Contradiction on case level 1, so:

$$kl = 0$$

Variables to be uneliminated:

"h5 := 'h5'"

"k5 := 'k5'"

"f3 := 'f3'"

```

"m5 := 'm5'"
"f4 := 'f4'"
"g4 := 'g4'"
"g3 := 'g3'"
"j4 := 'j4'"
"f2 := 'f2'"
"g1 := 'g1'"
"h4 := 'h4'"
"g2 := 'g2'"
"k4 := 'k4'"
"j3 := 'j3'"
"f1 := 'f1'"
"j2 := 'j2'"
"h3 := 'h3'"
"k3 := 'k3'"
"m4 := 'm4'"
"h2 := 'h2'"
"m3 := 'm3'"
"k2 := 'k2'"
"m2 := 'm2'"

```

Proceed on case level 0 with:

$$2 \neq 0$$

On account of:

$$k1 = 0$$

$$\{1 \neq 0\}$$

k1 is set to:

$$0$$

```
> launchNZcase (m2);
```

Launching case level 1:

$$m2 \neq 0$$

Assume from now on that:

$$2 \, m2 \neq 0$$

```
> tmp1 := cpcoeff(x1^3*x4^2);
```

$$tmp1 := -2 \, h1 \, m2$$

```
> elimsolve (tmp1,h1);
```

$$\{1 \neq 0\}$$

h1 is set to:

$$0$$

```
> tmp1 := cpcoeff(x1^3*x3*x5);
```

$$tmp1 := 4 \, j1 \, m2$$

```
> elimsolve (tmp1,j1);
```

$$\{1 \neq 0\}$$

j1 is set to:

$$0$$

> tmp1 := cpcoeff(x1^3\*x2\*x5);

$$tmp1 := 2\ g1\ m2$$

> elimsolve (tmp1,g1);

$$\{1 \neq 0\}$$

g1 is set to:

$$0$$

> tmp1 := cpcoeff(x1^3\*x2\*x4);

$$tmp1 := -4\ f1\ m2$$

> elimsolve (tmp1,f1);

$$\{1 \neq 0\}$$

f1 is set to:

$$0$$

> tmp1 := cpcoeff(x1\*x5^2\*T^2);

$$tmp1 := -2\ m2\ (3\ k2 + 2\ m3)$$

> elimsolve (tmp1,m3);

$$\{2 \neq 0\}$$

m3 is set to:

$$-\frac{3\ k2}{2}$$

> tmp1 := cpcoeff(x1^2\*x3\*x5\*T);

$$tmp1 := 4\ j2\ m2 - k2^2$$

> elimsolve (tmp1,j2);

$$\{4\ m2 \neq 0\}$$

j2 is set to:

$$\frac{k2^2}{4\ m2}$$

> tmp1 := cpcoeff(x1^2\*x2\*x5\*T);

$$tmp1 := -h2\ k2 + 2\ g2\ m2$$

> elimsolve (tmp1,g2);

$$\{2\ m2 \neq 0\}$$

g2 is set to:

$$\frac{h2\ k2}{2\ m2}$$

> tmp1 := cpcoeff(x5^2\*T^3);

$$tmp1 := -4\ k2^2 + 4\ m2\ m4 + 2\ m2\ h2$$

> elimsolve (tmp1,m4);

$$\{2\ m2 \neq 0\}$$

m4 is set to:

$$-\frac{-2\ k2^2 + m2\ h2}{2\ m2}$$

> tmp1 := cpcoeff(x1\*x4\*x5\*T^2);

```

|                                      $tmp1 := 2 k2^2 + 2 k3 m2 + 2 m2 h2$ 
| > elimsolve (tmp1,k3);
|                                      $\{m2 \neq 0\}$ 
| k3 is set to:
|                                      $-\frac{k2^2 + m2 h2}{m2}$ 
| > tmp1 := cpcoeff(x1*x3*x5*T^2);
|                                      $tmp1 := 3 h2 k2 + 2 k4 m2 + 8 j3 m2$ 
| > elimsolve (tmp1,k4);
|                                      $\{2 m2 \neq 0\}$ 
| k4 is set to:
|                                      $-\frac{3 h2 k2 + 8 j3 m2}{2 m2}$ 
| > tmp1 := cpcoeff(x5^3*T^2);
|                                      $tmp1 := k2^3 + 4 h2 k2 m2 + 8 m2^2 j3$ 
| > elimsolve (tmp1,j3);
|                                      $\{8 m2^2 \neq 0\}$ 
| j3 is set to:
|                                      $-\frac{k2 (k2^2 + 4 m2 h2)}{8 m2^2}$ 
| > tmp1 := cpcoeff(x1*x2*x5*T^2);
|                                      $tmp1 := 4 g3 m2 + 2 h2^2 + 2 h4 m2 + 4 f2 m2$ 
| > elimsolve (tmp1,h4);
|                                      $\{m2 \neq 0\}$ 
| h4 is set to:
|                                      $-\frac{2 g3 m2 + h2^2 + 2 f2 m2}{m2}$ 
| > tmp1 := cpcoeff(x4*x5*T^3);
|                                      $tmp1 := \frac{2 (3 h2 k2 m2 - k2^3 - 2 m2^2 m5 + h3 m2^2)}{m2}$ 
| > elimsolve (tmp1,m5);
|                                      $\{-2 m2^2 \neq 0\}$ 
| m5 is set to:
|                                      $\frac{3 h2 k2 m2 - k2^3 + h3 m2^2}{2 m2^2}$ 
| > tmp1 := cpcoeff(x4*x5^2*T^2);
|                                      $tmp1 := -\frac{-k2^4 + 2 h2 k2^2 m2 - 4 k5 m2^3 + 4 m2^2 h2^2 + 4 m2^3 g3}{m2}$ 
| > elimsolve (tmp1,g3);
|                                      $\{4 m2^3 \neq 0\}$ 
| g3 is set to:

```

$$- \frac{-k^2^4 + 2 h_2 k^2^2 m_2 - 4 k_5 m_2^3 + 4 m_2^2 h_2^2}{4 m_2^3}$$

> tmp1 := cpcoeff(x1^2\*x2\*x4\*T);

$$tmp1 := - \frac{-k^2^4 - 4 k_5 m_2^3 + 3 h_2 k^2^2 m_2 + 2 k_2 h_3 m_2^2 + 8 f_2 m_2^3}{2 m_2^2}$$

> elimsolve (tmp1,f2);

$$\{8 m_2^3 \neq 0\}$$

f2 is set to:

$$- \frac{-k^2^4 - 4 k_5 m_2^3 + 3 h_2 k^2^2 m_2 + 2 k_2 h_3 m_2^2}{8 m_2^3}$$

> tmp1 := cpcoeff(x3\*x5\*T^3);

$$tmp1 := \frac{4 h_2 k^2^2 m_2 + 4 k_2 h_3 m_2^2 - 8 k_5 m_2^3 - 3 k^2^4 + 16 j_4 m_2^3}{4 m_2^2}$$

> elimsolve (tmp1,j4);

$$\{16 m_2^3 \neq 0\}$$

j4 is set to:

$$- \frac{4 h_2 k^2^2 m_2 + 4 k_2 h_3 m_2^2 - 8 k_5 m_2^3 - 3 k^2^4}{16 m_2^3}$$

> tmp1 := cpcoeff(x3\*x5^2\*T^2);

$$tmp1 := \frac{2 h_2 k^2^3 m_2 - k^2^5 - 8 k_2 m_2^3 k_5 + 32 j_5 m_2^4}{4 m_2^2}$$

> elimsolve (tmp1,j5);

$$\{32 m_2^4 \neq 0\}$$

j5 is set to:

$$- \frac{k_2 (2 h_2 k^2^2 m_2 - k^2^4 - 8 k_5 m_2^3)}{32 m_2^4}$$

> tmp1 := cpcoeff(x4^2\*T^3);

$$tmp1 := - \frac{2 (-k^2^4 + 3 h_2 k^2^2 m_2 + 2 m_2^2 h_2^2 - 4 k_5 m_2^3 + 2 k_2 h_3 m_2^2)}{m_2^2}$$

> elimsolve (tmp1,k5);

$$\{-4 m_2^3 \neq 0\}$$

k5 is set to:

$$\frac{-k^2^4 + 3 h_2 k^2^2 m_2 + 2 m_2^2 h_2^2 + 2 k_2 h_3 m_2^2}{4 m_2^3}$$

> tmp1 := cpcoeff(x1\*x4^3\*T);

$$tmp1 := - \frac{2 h_3 k^2^2 m_2 + 3 h_2^2 k_2 m_2 + h_2 k^2^3 - 4 h_5 m_2^3}{m_2}$$

> elimsolve (tmp1,h5);

$$\{-4 m_2^3 \neq 0\}$$

h5 is set to:

$$\frac{k^2 (2 k^2 h^3 m^2 + 3 m^2 h^2 + h^2 k^2)}{4 m^2^3}$$

> **tmp1 := cpcoeff(x1\*x2\*x4\*T^2);**

$$tmp1 := \frac{-8 f^3 m^2 + 3 h^2 k^2 + 4 m^2 h^2 h^3}{2 m^2}$$

> **elimsolve (tmp1,f3);**

$$\{-8 m^2 \neq 0\}$$

f3 is set to:

$$\frac{h^2 (3 h^2 k^2 + 4 h^3 m^2)}{8 m^2^2}$$

> **tmp1 := cpcoeff(x2\*x5^2\*T^2);**

$$tmp1 := -\frac{-8 g^5 m^2 + 2 m^2 h^2 + 4 g^4 m^2 k^2 + h^2 k^2}{2 m^2}$$

> **elimsolve (tmp1,g5);**

$$\{-8 m^2 \neq 0\}$$

g5 is set to:

$$\frac{2 m^2 h^2 + 4 g^4 m^2 k^2 + h^2 k^2}{8 m^2^3}$$

> **tmp1 := cpcoeff(x2\*x4\*x5\*T^2);**

$$tmp1 := -\frac{16 f^5 m^2 + 8 f^4 m^2 k^2 + h^2 k^2 + 2 m^2 h^2 h^3}{2 m^2}$$

> **elimsolve (tmp1,f5);**

$$\{16 m^2 \neq 0\}$$

f5 is set to:

$$-\frac{8 f^4 m^2 k^2 + h^2 k^2 + 2 m^2 h^2 h^3}{16 m^2^3}$$

> **tmp1 := cpcoeff(x2\*x5\*T^3);**

$$tmp1 := \frac{h^2 k^2 + 4 h^2 k^2 m^2 + 2 h^3 k^2 m^2 + 4 m^2 h^2 h^3 + 8 g^4 m^2}{4 m^2^2}$$

> **elimsolve (tmp1,g4);**

$$\{8 m^2 \neq 0\}$$

g4 is set to:

$$-\frac{h^2 k^2 + 4 h^2 k^2 m^2 + 2 h^3 k^2 m^2 + 4 m^2 h^2 h^3}{8 m^2^3}$$

> **tmp1 := cpcoeff(x2\*x4\*T^3);**

$$tmp1 := -\frac{2 m^2 h^2 + 16 f^4 m^2 + h^2 k^2 - 4 m^2 h^2 k^2 h^3 - 4 h^3 m^2}{4 m^2^2}$$

> **elimsolve (tmp1,f4);**

$$\{16 m^2 \neq 0\}$$

f4 is set to:

$$-\frac{2 m_2 h_2^3 - h_2^2 k_2^2 - 4 m_2 h_2 k_2 h_3 - 4 h_3^2 m_2^2}{16 m_2^3}$$

> det (T - jacobian(H,X));

$$T^5$$

> H[1];

$$0$$

> U := evalm([[1/(2\*m2), 0, 0, 0, 0], [-1/8\*k2/m2^2, 8\*m2^3, 0, 0, 0], [1/16\*(k2^2-2\*m2\*h2)/m2^3, -4\*k2\*m2^2, 4\*m2^2, 0, 0], [-1/32\*k2\*(k2^2-4\*m2\*h2)/m2^4, 2\*(k2^2-2\*m2\*h2)\*m2, -2\*k2\*m2, 2\*m2, 0], [1/64\*(k2^4-10\*h2\*k2^2\*m2-4\*k2\*h3\*m2^2+4\*m2^2\*h2^2)/m2^5, -k2^3+8\*h2\*k2\*m2+4\*h3\*m2^2, k2^2-2\*m2\*h2, -k2, 1]]);

U:=

$$\left[ \frac{1}{2 m_2}, 0, 0, 0, 0 \right]$$

$$\left[ -\frac{k_2}{8 m_2^2}, 8 m_2^3, 0, 0, 0 \right]$$

$$\left[ \frac{k_2^2 - 2 m_2 h_2}{16 m_2^3}, -4 k_2 m_2^2, 4 m_2^2, 0, 0 \right]$$

$$\left[ -\frac{k_2 (k_2^2 - 4 m_2 h_2)}{32 m_2^4}, 2 (k_2^2 - 2 m_2 h_2) m_2, -2 k_2 m_2, 2 m_2, 0 \right]$$

$$\left[ \frac{k_2^4 - 10 h_2 k_2^2 m_2 - 4 k_2 h_3 m_2^2 + 4 m_2^2 h_2^2}{64 m_2^5}, -k_2^3 + 8 h_2 k_2 m_2 + 4 h_3 m_2^2, k_2^2 - 2 m_2 h_2 \right.$$

$$\left. , -k_2, 1 \right]$$

> G := evalm(U^(-1)&\*subs({seq(X[i]=evalm(U&\*X)[i],i=1..5)},H));

> simplify (jacobian (G, X));

$$\begin{bmatrix} 0 & 0 & 0 & 0 \\ \frac{x_1}{32 m_2^5} & 0 & 0 & x_4 & 0 \\ x_2 & x_1 & 0 & -x_5 & -x_4 \\ x_3 & 0 & x_1 & 0 & x_5 \\ -\frac{x_1 m_2 h_3 + x_1 h_2 k_2 - 8 m_2^4 x_4}{8 m_2^4} & 0 & 0 & x_1 & 0 \end{bmatrix}$$

> factor(evalm([0,0,0,0,1] &\* jacobian(G,X)^4 &\* X));

$$\frac{x_1^3 (x_1^2 + 4 m_2^2 x_4 x_1 h_3 + 4 m_2 x_4 x_1 h_2 k_2 - 32 m_2^5 x_4^2)}{32 m_2^5}$$

> contradict (1);

Contradiction on case level 1, so:

$$m_2 = 0$$

Variables to be uneliminated:

"f4 := 'f4"  
"g4 := 'g4"  
"f5 := 'f5"  
"g5 := 'g5"  
"f3 := 'f3"  
"h5 := 'h5"  
"k5 := 'k5"  
"j5 := 'j5"  
"j4 := 'j4"  
"f2 := 'f2"  
"g3 := 'g3"  
"m5 := 'm5"  
"h4 := 'h4"  
"j3 := 'j3"  
"k4 := 'k4"  
"k3 := 'k3"  
"m4 := 'm4"  
"g2 := 'g2"  
"j2 := 'j2"  
"m3 := 'm3"  
"f1 := 'f1"  
"g1 := 'g1"  
"j1 := 'j1"  
"h1 := 'h1"

Proceed on case level 0 with:

$$2 \neq 0$$

On account of:

$$m2 = 0$$

$$\{1 \neq 0\}$$

m2 is set to:

$$0$$

> **launchNZcase (h1);**

Launching case level 1:

$$h1 \neq 0$$

Assume from now on that:

$$2 \, h1 \neq 0$$

> **tmp1 := cpcoeff (x1^3\*x2\*x5,h1);**

$$tmp1 := 2 \, h1 \, (k2 + j1 + h1 + m3)$$

> **elimsolve (tmp1,j1);**

$$\{1 \neq 0\}$$

j1 is set to:





```
> elimsolve (tmp1,m4);
```

$$\{-2 \neq 0\}$$

```
m4 is set to:
```

$$\frac{h2}{2}$$

```
> tmp1 := cpcoeff(x4*x5*T^3);
```

$$tmp1 := -2jl(h2 - k3 - 2j2)$$

```
> elimsolve (tmp1,h2);
```

$$\{1 \neq 0\}$$

```
h2 is set to:
```

$$k3 + 2j2$$

```
> tmp1 := cpcoeff(x1*x3*x5*T^2);
```

$$tmp1 := -2(gl + k3 + 2j2)jl$$

```
> elimsolve (tmp1,k3);
```

$$\{1 \neq 0\}$$

```
k3 is set to:
```

$$-gl - 2j2$$

```
> tmp1 := cpcoeff(x3*x5*T^3);
```

$$tmp1 := -2jl(2fl + h3 + g2)$$

```
> elimsolve (tmp1,h3);
```

$$\{1 \neq 0\}$$

```
h3 is set to:
```

$$-2fl - g2$$

```
> tmp1 := cpcoeff(x1^2*x2*x4*T);
```

$$tmp1 := 4fljl - gl^2$$

```
> elimsolve (tmp1,fl);
```

$$\{4jl \neq 0\}$$

```
fl is set to:
```

$$\frac{gl^2}{4jl}$$

```
> tmp1 := cpcoeff(x1*x3*x4*T^2);
```

$$tmp1 := -gl^2 - 2glj2 + 2g2jl$$

```
> elimsolve (tmp1,g2);
```

$$\{-2jl \neq 0\}$$

```
g2 is set to:
```

$$\frac{gl(gl + 2j2)}{2jl}$$

```
> tmp1 := cpcoeff(x1^2*x3^2*T);
```

$$tmp1 := 2jl k4 - gl^2 - 2glj2$$

```
> elimsolve (tmp1,k4);
```

$$\{-2jl \neq 0\}$$

```
k4 is set to:
```

```

|                                     
$$\frac{gl (gl + 2 j2)}{2 j1}$$

| > tmp1 := cpcoeff(x4^2*T^3);
|                                     
$$tmp1 := -(3 gl + 2 j2)^2$$

| > elimsolve (tmp1,j2);
|                                     
$$\{2 \neq 0\}$$

| j2 is set to:
|                                     
$$-\frac{3 gl}{2}$$

| > tmp1 := cpcoeff(x4^3*T^2);
|                                     
$$tmp1 := gl^3 + 4 h4 j1^2$$

| > elimsolve (tmp1,h4);
|                                     
$$\{4 j1^2 \neq 0\}$$

| h4 is set to:
|                                     
$$-\frac{gl^3}{4 j1^2}$$

| > tmp1 := cpcoeff(x1*x3^2*T^2);
|                                     
$$tmp1 := 4 j4 j1 + 2 gl j3$$

| > elimsolve (tmp1,j4);
|                                     
$$\{2 j1 \neq 0\}$$

| j4 is set to:
|                                     
$$-\frac{gl j3}{2 j1}$$

| > tmp1 := cpcoeff(x1*x2*x4*T^2);
|                                     
$$tmp1 := \frac{gl^3 + 8 f2 j1^2}{2 j1}$$

| > elimsolve (tmp1,f2);
|                                     
$$\{8 j1^2 \neq 0\}$$

| f2 is set to:
|                                     
$$-\frac{gl^3}{8 j1^2}$$

| > tmp1 := cpcoeff(x1*x2*x3*T^2);
|                                     
$$tmp1 := 2 g4 j1 + g3 gl$$

| > elimsolve (tmp1,g4);
|                                     
$$\{2 j1 \neq 0\}$$

| g4 is set to:
|                                     
$$-\frac{g3 gl}{2 j1}$$

| > tmp1 := cpcoeff(x1*x3^3*T);
|                                     
$$tmp1 := 4 j1^2$$

| > contradict (tmp1);
| Contradiction on case level 1, so:

```

|                                           |                                       |
|-------------------------------------------|---------------------------------------|
|                                           | $j1 = 0$                              |
| Variables to be uneliminated:             |                                       |
|                                           | "g4 := 'g4'"                          |
|                                           | "f2 := 'f2'"                          |
|                                           | "j4 := 'j4'"                          |
|                                           | "h4 := 'h4'"                          |
|                                           | "j2 := 'j2'"                          |
|                                           | "k4 := 'k4'"                          |
|                                           | "g2 := 'g2'"                          |
|                                           | "f1 := 'f1'"                          |
|                                           | "h3 := 'h3'"                          |
|                                           | "k3 := 'k3'"                          |
|                                           | "h2 := 'h2'"                          |
|                                           | "m4 := 'm4'"                          |
| Proceed on case level 0 with:             |                                       |
|                                           | $2 \neq 0$                            |
| On account of:                            |                                       |
|                                           | $j1 = 0$                              |
|                                           | $\{1 \neq 0\}$                        |
| j1 is set to:                             |                                       |
|                                           | 0                                     |
| > <b>launchNZcase (g1);</b>               |                                       |
| Launching case level 1:                   |                                       |
|                                           | $g1 \neq 0$                           |
| Assume from now on that:                  |                                       |
|                                           | $2 g1 \neq 0$                         |
| > <b>tmp1 := cpcoeff (x1^3*x2*x3);</b>    |                                       |
|                                           | $tmp1 := -g1 (2 g1 + k3 + 2 j2 + h2)$ |
| > <b>elimsolve (tmp1,h2);</b>             |                                       |
|                                           | $\{1 \neq 0\}$                        |
| h2 is set to:                             |                                       |
|                                           | $-2 g1 - k3 - 2 j2$                   |
| > <b>tmp1 := cpcoeff (x1^2*x2*x3*x5);</b> |                                       |
|                                           | $tmp1 := -2 g1 (g1 + k3 + 2 j2)^2$    |
| > <b>elimsolve (tmp1,k3);</b>             |                                       |
|                                           | $\{1 \neq 0\}$                        |
| k3 is set to:                             |                                       |
|                                           | $-g1 - 2 j2$                          |
| > <b>tmp1 := cpcoeff (x1^2*x3^2*T);</b>   |                                       |
|                                           | $tmp1 := -g1 (g1 + 2 j2)$             |
| > <b>elimsolve (tmp1,j2);</b>             |                                       |
|                                           | $\{2 \neq 0\}$                        |
| j2 is set to:                             |                                       |

```

[

$$-\frac{gl}{2}$$

> tmp1 := cpcoeff (x1*x3^2*T^2);

$$tmp1 := 2\ gl\ j3$$

> elimsolve (tmp1,j3);

$$\{1 \neq 0\}$$

j3 is set to:

$$0$$

> tmp1 := cpcoeff (x1^2*x2*x4*T);

$$tmp1 := 2\ gl\ m4$$

> elimsolve (tmp1,m4);

$$\{1 \neq 0\}$$

m4 is set to:

$$0$$

> tmp1 := cpcoeff (x4^2*T^3);

$$tmp1 := -gl^2$$

> contradict (tmp1);
Contradiction on case level 1, so:

$$gl = 0$$

Variables to be uneliminated:
"m4 := 'm4'"
"j3 := 'j3'"
"j2 := 'j2'"
"k3 := 'k3'"
"h2 := 'h2'"
Proceed on case level 0 with:

$$2 \neq 0$$

On account of:

$$gl = 0$$


$$\{1 \neq 0\}$$

gl is set to:

$$0$$

> launchNZcase (h2);
Launching case level 1:

$$h2 \neq 0$$

Assume from now on that:

$$2\ h2 \neq 0$$

> tmp1 := cpcoeff (x1^3*x2^2);

$$tmp1 := -2\ fl\ h2$$

> elimsolve (tmp1,f1);

$$\{1 \neq 0\}$$

f1 is set to:

$$0$$

> tmp1 := cpcoeff (x1*x2*x5*T^2);

```

```

[                                      $tmp1 := -h2 (k3 + 2 m4)$ 
> elimsolve (tmp1,m4);
                                      $\{2 \neq 0\}$ 
m4 is set to:
                                      $-\frac{k3}{2}$ 
[
> tmp1 := cpcoeff (x1^2*x2*x4*T);
                                      $tmp1 := -2 h2^2$ 
> contradict (tmp1);
Contradiction on case level 1, so:
                                      $h2 = 0$ 
Variables to be uneliminated:
                                     "m4 := 'm4'"
                                     "f1 := 'f1'"
Proceed on case level 0 with:
                                      $2 \neq 0$ 
On account of:
                                      $h2 = 0$ 
                                      $\{1 \neq 0\}$ 
h2 is set to:
                                     0
[
> launchNZcase (j2);
Launching case level 1:
                                      $j2 \neq 0$ 
Assume from now on that:
                                      $2 j2 \neq 0$ 
[
> tmp1 := cpcoeff (x1^2*x3^2*T);
                                      $tmp1 := -2 j2 (k3 + 2 j2)$ 
> elimsolve (tmp1,k3);
                                      $\{1 \neq 0\}$ 
k3 is set to:
                                      $-2 j2$ 
[
> tmp1 := cpcoeff (x1*x3*x4*T^2);
                                      $tmp1 := 4 j2 m4$ 
> elimsolve (tmp1,m4);
                                      $\{1 \neq 0\}$ 
m4 is set to:
                                     0
[
> tmp1 := cpcoeff (x4^2*T^3);
                                      $tmp1 := -4 j2^2$ 
> contradict (tmp1);
Contradiction on case level 1, so:
                                      $j2 = 0$ 
Variables to be uneliminated:
                                     "m4 := 'm4'"

```

|                                                      |                                                             |
|------------------------------------------------------|-------------------------------------------------------------|
|                                                      | "k3 := 'k3'"                                                |
| Proceed on case level 0 with:                        |                                                             |
|                                                      | $2 \neq 0$                                                  |
| On account of:                                       |                                                             |
|                                                      | $j2 = 0$                                                    |
|                                                      | $\{1 \neq 0\}$                                              |
| j2 is set to:                                        |                                                             |
|                                                      | 0                                                           |
| > <b>launchNZcase (g2);</b>                          |                                                             |
| Launching case level 1:                              |                                                             |
|                                                      | $g2 \neq 0$                                                 |
| Assume from now on that:                             |                                                             |
|                                                      | $2 g2 \neq 0$                                               |
| > <b>tmp1 := cpcoeff (x1^2*x2*x3*T);</b>             |                                                             |
|                                                      | $tmp1 := -g2 k3$                                            |
| > <b>elimsolve (tmp1,k3);</b>                        |                                                             |
|                                                      | $\{1 \neq 0\}$                                              |
| k3 is set to:                                        |                                                             |
|                                                      | 0                                                           |
| > <b>tmp1 := cpcoeff (x4^2*T^3);</b>                 |                                                             |
|                                                      | $tmp1 := -4 m4^2$                                           |
| > <b>elimsolve (tmp1,m4);</b>                        |                                                             |
|                                                      | $\{1 \neq 0\}$                                              |
| m4 is set to:                                        |                                                             |
|                                                      | 0                                                           |
| > <b>tmp1 := cpcoeff (x1^2*x2^2*T);</b>              |                                                             |
|                                                      | $tmp1 := -4 fl g2 - g2 h3 - g2^2 - 4 fl^2$                  |
| > <b>elimsolve (tmp1,h3);</b>                        |                                                             |
|                                                      | $\{g2 \neq 0\}$                                             |
| h3 is set to:                                        |                                                             |
|                                                      | $-\frac{(2 fl + g2)^2}{g2}$                                 |
| > <b>tmp1 := cpcoeff(x3^4*T);</b>                    |                                                             |
|                                                      | $tmp1 := -2 g2 j3 k4 (k4 + g2 + 2 j3)$                      |
| > <b>tmp2 := cpcoeff(x3^3*T^2);</b>                  |                                                             |
|                                                      | $tmp2 := (2 j3 + k4) (k4 + g2) (g2 + 2 j3)$                 |
| > <b>tmp3 := cpcoeff(x3^2*T^3);</b>                  |                                                             |
|                                                      | $tmp3 := -g2 k4 - g2^2 - 2 g2 j3 - 2 j3 k4 - 4 j3^2 - k4^2$ |
| > <b>tmp4 := factor(tmp1 + g2*tmp2 + g2^2*tmp3);</b> |                                                             |
|                                                      | $tmp4 := -g2^4$                                             |
| > <b>contradict (tmp4);</b>                          |                                                             |
| Contradiction on case level 1, so:                   |                                                             |
|                                                      | $g2 = 0$                                                    |
| Variables to be uneliminated:                        |                                                             |

|                                    |                    |
|------------------------------------|--------------------|
|                                    | "h3 := 'h3'"       |
|                                    | "m4 := 'm4'"       |
|                                    | "k3 := 'k3'"       |
| Proceed on case level 0 with:      |                    |
|                                    | $2 \neq 0$         |
| On account of:                     |                    |
|                                    | $g2 = 0$           |
|                                    | $\{1 \neq 0\}$     |
| g2 is set to:                      |                    |
|                                    | 0                  |
| > tmp1 := cpcoeff (x1^2*x2^2*T);   |                    |
|                                    | $tmp1 := -4 f1^2$  |
| > elimsolve (tmp1,f1);             |                    |
|                                    | $\{1 \neq 0\}$     |
| f1 is set to:                      |                    |
|                                    | 0                  |
| > launchNZcase (m4);               |                    |
| Launching case level 1:            |                    |
|                                    | $m4 \neq 0$        |
| Assume from now on that:           |                    |
|                                    | $2 m4 \neq 0$      |
| > tmp1 := cpcoeff (x3*x5*T^3);     |                    |
|                                    | $tmp1 := -2 k3 m4$ |
| > elimsolve (tmp1,k3);             |                    |
|                                    | $\{1 \neq 0\}$     |
| k3 is set to:                      |                    |
|                                    | 0                  |
| > tmp1 := cpcoeff (x4^2*T^3);      |                    |
|                                    | $tmp1 := -4 m4^2$  |
| > contradict (tmp1);               |                    |
| Contradiction on case level 1, so: |                    |
|                                    | $m4 = 0$           |
| Variables to be uneliminated:      |                    |
|                                    | "k3 := 'k3'"       |
| Proceed on case level 0 with:      |                    |
|                                    | $2 \neq 0$         |
| On account of:                     |                    |
|                                    | $m4 = 0$           |
|                                    | $\{1 \neq 0\}$     |
| m4 is set to:                      |                    |
|                                    | 0                  |
| > tmp1 := cpcoeff (x4^2*T^3);      |                    |
|                                    | $tmp1 := -k3^2$    |
| > elimsolve (tmp1,k3);             |                    |
|                                    | $\{1 \neq 0\}$     |



```

k3 is set to:
0
> launchNZcase (h3);
Launching case level 1:
h3 ≠ 0
Assume from now on that:
2 h3 ≠ 0
> tmp1 := cpcoeff (x1*x2*x3*T^2);
tmp1 := -h3 (k4 + 4 j3)
> elimsolve (tmp1,k4);
{1 ≠ 0}
k4 is set to:
-4 j3
> tmp1 := cpcoeff (x3^3*T^2);
tmp1 := 16 j3^3
> elimsolve (tmp1,j3);
{1 ≠ 0}
j3 is set to:
0
> tmp1 := cpcoeff (x2*x4*T^3);
tmp1 := 2 h3 m5
> elimsolve (tmp1,m5);
{1 ≠ 0}
m5 is set to:
0
> tmp1 := cpcoeff (x2^2*x4*T^2);
tmp1 := k5 h3^2
> elimsolve (tmp1,k5);
{1 ≠ 0}
k5 is set to:
0
> tmp1 := cpcoeff (x2*x3*T^3);
tmp1 := -2 h3 j4
> elimsolve (tmp1,j4);
{1 ≠ 0}
j4 is set to:
0
> tmp1 := cpcoeff (x2^2*x3*T^2);
tmp1 := 2 j5 h3^2
> elimsolve (tmp1,j5);
{1 ≠ 0}
j5 is set to:
0
> tmp1 := cpcoeff (x1*x2^2*T^2);

```

```

[                                      $tmp1 := -h3 (2 g3 + h4 + 2 f2)$ 
> elimsolve (tmp1,h4);
                                      $\{1 \neq 0\}$ 
h4 is set to:
                                      $-2 g3 - 2 f2$ 
> tmp1 := cpcoeff (x2^2*T^3);
                                      $tmp1 := -3 g3^2 - 4 f2 g3 - 4 f2^2 - h3 g4 + h3 h5$ 
> elimsolve (tmp1,h5);
                                      $\{-h3 \neq 0\}$ 
h5 is set to:
                                      $\frac{3 g3^2 + 4 f2 g3 + 4 f2^2 + h3 g4}{h3}$ 
> tmp1 := cpcoeff (x2^3*T^2);
                                      $tmp1 := h3^2 g5 - 2 f2 g3^2 - 4 f2^2 g3 - 8 f2^3 - g3^3$ 
> elimsolve (tmp1,g5);
                                      $\{-h3^2 \neq 0\}$ 
g5 is set to:
                                      $\frac{(g3 + 2 f2) (g3^2 + 4 f2^2)}{h3^2}$ 
> tmp1 := cpcoeff (x2^4*T);
                                      $tmp1 := -16 f2^4$ 
> elimsolve (tmp1,f2);
                                      $\{1 \neq 0\}$ 
f2 is set to:
                                     0
> collect(det(T-jacobian(H,[x1,x2,x3,x4,x5])),T);
                                      $T^5$ 
> U := evalm([[1, 0, 0, 0, 0], [0, 1/h3, 0, 0, 0], [-1/2/h3*f3, 0,
1, 0, 0], [-1/h3+1/2*g3/h3^2*f3, -1/h3^2*f3, -g3/h3, 1, 0],
[2/h3^2*g3-1/2*(h3*g4+2*g3^2)/h3^3*f3, (f4*h3+2*f3*g3)/h3^3,
(h3*g4+2*g3^2)/h3^2, -g3/h3, 1]]);
                                     
$$U := \begin{bmatrix} 1 & 0 & 0 & 0 & 0 \\ 0 & \frac{1}{h3} & 0 & 0 & 0 \\ -\frac{f3}{2 h3} & 0 & 1 & 0 & 0 \\ -\frac{1}{h3} + \frac{g3 f3}{2 h3^2} & -\frac{f3}{h3^2} & -\frac{g3}{h3} & 1 & 0 \\ \frac{2 g3}{h3^2} - \frac{(h3 g4 + 2 g3^2) f3}{2 h3^3} & \frac{f4 h3 + 2 f3 g3}{h3^3} & \frac{h3 g4 + 2 g3^2}{h3^2} & -\frac{g3}{h3} & 1 \end{bmatrix}$$

> G := evalm(U^(-1)&*subs({seq(X[i]=evalm(U&*X)[i],i=1..5)},H)):
> simplify (jacobian (G, X));

```

$$\begin{bmatrix}
0, 0, 0, 0, 0 \\
x1 \, h3, 0, 0, 0, 0 \\
0, x4, 0, x2, 0 \\
x3, -x5, x1, 0, -x2 \\
-\frac{x1 \, h3 f3 g3 + x1 \, h3^2 f4 + 2 \, x1 \, h3^2 + f3 \, x2 \, h3 - x4 \, h3^3 + x2 \, g3^2 + x2 \, h3 \, g4}{h3^3}, \\
-\frac{2 \, g3^2 \, x2 \, f3 + 2 \, g4 \, x2 \, f3 \, h3 + f3 \, x1 \, h3^2 - 2 \, f5 \, x2 \, h3^2 + g3^2 \, x1 \, h3 + h3^2 \, g4 \, x1 - 2 \, g3 \, f4 \, x2 \, h3}{h3^4}, \\
0, x1, 0
\end{bmatrix}$$

```
> factor(evalm([0,0,0,0,1] &* jacobian(G,X)^4 &* X));
```

$$x1^3 (x4 \, h3^4 \, x1 + 2 \, g3^2 \, x2^2 \, f3 + 2 \, g4 \, x2^2 \, f3 \, h3 + x2 \, f3 \, x1 \, h3^2 - 2 \, f5 \, x2^2 \, h3^2 + x2 \, g3^2 \, x1 \, h3 + x2 \, h3^2 \, g4 \, x1 - 2 \, g3 \, f4 \, x2^2 \, h3) / h3^3$$

```
> contradict (1);
```

Contradiction on case level 1, so:

$$h3 = 0$$

Variables to be uneliminated:

"f2 := 'f2'"

"g5 := 'g5'"

"h5 := 'h5'"

"h4 := 'h4'"

"j5 := 'j5'"

"j4 := 'j4'"

"k5 := 'k5'"

"m5 := 'm5'"

"j3 := 'j3'"

"k4 := 'k4'"

Proceed on case level 0 with:

$$2 \neq 0$$

On account of:

$$h3 = 0$$

$$\{1 \neq 0\}$$

h3 is set to:

$$0$$

```
> tmp1 := cpcoeff (x3^2*T^3);
```

$$tmp1 := -2 \, j3 \, k4 - 4 \, j3^2 - k4^2$$

```
> tmp2 := cpcoeff (x3^3*T^2);
```

$$tmp2 := 2 \, j3 \, k4 (2 \, j3 + k4)$$

```
> tmp3 := factor (k4*tmp1 + tmp2);
```

$$tmp3 := -k4^3$$

```
> elimsolve (tmp3,k4);
```

```

                                {1 ≠ 0}
k4 is set to:
                                0
> tmp1 := cpcoeff (x3^2*T^3);
                                tmp1 := -4 j3^2
> elimsolve (tmp1,j3);
                                {1 ≠ 0}
j3 is set to:
                                0
> tmp1 := cpcoeff (x2^2*T^3);
                                tmp1 := -h4 g3 - 2 f2 h4 - g3^2 - 2 f2 g3 - 4 f2^2 - h4^2
> tmp2 := cpcoeff (x2^3*T^2);
                                tmp2 := (h4 + g3) (2 f2 + h4) (g3 + 2 f2)
> tmp3 := cpcoeff (x2^4*T);
                                tmp3 := -2 f2 g3 h4 (g3 + h4 + 2 f2)
> tmp4 := factor(h4^2*tmp1 + h4*tmp2 + tmp3);
                                tmp4 := -h4^4
> elimsolve (tmp4,h4);
                                {1 ≠ 0}
h4 is set to:
                                0
> tmp1 := cpcoeff (x2^2*T^3);
                                tmp1 := -g3^2 - 2 f2 g3 - 4 f2^2
> tmp2 := cpcoeff (x2^3*T^2);
                                tmp2 := 2 f2 g3 (g3 + 2 f2)
> tmp3 := factor(g3*tmp1 + tmp2);
                                tmp3 := -g3^3
> elimsolve (tmp3,g3);
                                {1 ≠ 0}
g3 is set to:
                                0
> tmp1 := cpcoeff (x2^2*T^3);
                                tmp1 := -4 f2^2
> elimsolve (tmp1,f2);
                                {1 ≠ 0}
f2 is set to:
                                0
> collect(det(T-jacobian(H, [x1,x2,x3,x4,x5])) , T);
                                T^5
> H;
[ 0,  $\frac{x1^2}{2}$ ,  $x1 x2 + f3 x2^2$ ,  $x1 x3 + f4 x2^2 + g4 x2 x3 + j4 x3^2$ ,

```

$$x1 x4 + f5 x2^2 + g5 x2 x3 + h5 x2 x4 + j5 x3^2 + k5 x3 x4 + m5 x4^2$$

> **jacobian**(H, [x1,x2,x3,x4,x5]);

$$\begin{bmatrix} 0 & 0 & 0 & 0 & 0 \\ x1 & 0 & 0 & 0 & 0 \\ x2 & x1 + 2f3x2 & 0 & 0 & 0 \\ x3 & 2f4x2 + g4x3 & x1 + g4x2 + 2j4x3 & 0 & 0 \\ x4 & 2f5x2 + g5x3 + h5x4 & g5x2 + 2j5x3 + k5x4 & x1 + h5x2 + k5x3 + 2m5x4 & 0 \end{bmatrix}$$

> **contradict** (1);

Contradiction on case level 0, so:

$$2 = 0$$

Variables to be uneliminated:

"f2 := 'f2'"  
 "g3 := 'g3'"  
 "h4 := 'h4'"  
 "j3 := 'j3'"  
 "k4 := 'k4'"  
 "h3 := 'h3'"  
 "k3 := 'k3'"  
 "m4 := 'm4'"  
 "f1 := 'f1'"  
 "g2 := 'g2'"  
 "j2 := 'j2'"  
 "h2 := 'h2'"  
 "g1 := 'g1'"  
 "j1 := 'j1'"  
 "m3 := 'm3'"  
 "k2 := 'k2'"  
 "h1 := 'h1'"  
 "m2 := 'm2'"  
 "k1 := 'k1'"  
 "m1 := 'm1'"  
 "n1 := 'n1'"  
 "o1 := 'o1'"  
 "l1 := 'l1'"  
 "i1 := 'i1'"  
 "n2 := 'n2'"  
 "o2 := 'o2'"  
 "l2 := 'l2'"  
 "i2 := 'i2'"

"n3 := 'n3'"

"o3 := 'o3'"

"l3 := 'l3'"

"i3 := 'i3'"

"n4 := 'n4'"

"o4 := 'o4'"

"l4 := 'l4'"

"i4 := 'i4'"

"n5 := 'n5'"

"o5 := 'o5'"

"l5 := 'l5'"

"i5 := 'i5'"

That is all, folks! Check that all variables are uneliminated:

```
[[a1, b1, c1, d1, e1, f1, g1, h1, i1, j1, k1, l1, m1, n1, o1],  
 [a2, b2, c2, d2, e2, f2, g2, h2, i2, j2, k2, l2, m2, n2, o2],  
 [a3, b3, c3, d3, e3, f3, g3, h3, i3, j3, k3, l3, m3, n3, o3],  
 [a4, b4, c4, d4, e4, f4, g4, h4, i4, j4, k4, l4, m4, n4, o4],  
 [a5, b5, c5, d5, e5, f5, g5, h5, i5, j5, k5, l5, m5, n5, o5]]
```

[ >
