# Supplementary material for: Quadratic homogeneous polynomial maps $H$ and Keller maps $x+H$ with $3 \le {\rm rk} J H \le 4$
Source: arXiv:1711.00904 ancillary file (2017-11-02)
Supplement: Supplementary file 2 [file dim6chr2qdr.pdf]

```

[ > restart;
  > efactors := proc (eq)
  >   local F, IF, i, c;
  >   F := factors (eq);
  >   for i from 1 to nops(F[2]) do
  >     c := content (F[2][i][1]);
  >     F[2][i][1] := F[2][i][1] / c;
  >     F[1] := F[1] * c ^ F[2][i][2];
  >   od;
  >   IF := ifactors (F[1]);
  >   return (IF[1], [op(IF[2]), op(F[2])]);
  > end;

```

*efactors* := **proc**(eq)

**local** F, IF, i, c;

F := factors(eq);

**for** i **to** nops(F[2]) **do**

c := content(F[2][i][1]);

F[2][i][1] := F[2][i][1] / c;

F[1] := F[1]\*c^F[2][i][2]

**end do**;

IF := ifactors(F[1]);

**return** IF[1], [op(IF[2]), op(F[2])]

**end proc**

```

[ > psqf := proc (eq)
  >   local EF, S, i;
  >   EF := efactors (eq);
  >   S := EF[1];
  >   for i from 1 to nops(EF[2]) do
  >     if (EF[2][i][2] > 0) then
  >       S := S * EF[2][i][1]
  >     fi
  >   od;
  >   return S
  > end;

```

*psqf* := **proc**(eq)

**local** EF, S, i;

EF := efactors(eq);

S := EF[1];

**for** i **to** nops(EF[2]) **do** **if** 0 < EF[2][i][2] **then** S := S\*EF[2][i][1] **end if** **end do**;

**return** S

**end proc**

```

[ > initcases := proc ()
  >   global nz, NZ, SV;

```

```

>   if nargs = 0 then
>       nz := 1
>   else
>       nz := args[1];
>       printf ("We assume the following in our calculation:");
>       print (psqf (nz) <> 0);
>   fi;
>   NZ := [convert (nz,string)];
>   SV := [[]];
>   return
> end;

```

*initcases* := **proc**()

**global** *nz, NZ, SV*;

**if** nargs = 0 **then** *nz* := 1

**else**

*nz* := args[ 1 ];

        printf ("We assume the following in our calculation:");

        print(psqf(*nz*) ≠ 0)

**end if**;

*NZ* := [ convert(*nz*, *string*) ];

*SV* := [ [ ] ];

**return**

**end proc**

> **launchNZcase** := **proc** (*nz*)

>     **global** *NZ, SV*;

>     **local** *t*;

>     *NZ* := [seq(*NZ*[*i*], *i*=1..*nops*(*NZ*)), convert (*nz*,*string*)];

>     *SV* := [seq(*SV*[*i*], *i*=1..*nops*(*SV*)), [ ]];

>     printf ("Launching case level %d:", *nops*(*NZ*) - 1);

>     print (*nz* <> 0);

>     printf ("Assume from now on that:");

>     *t* := mul (psqf (parse (*NZ*[*i*],*statement*)), *i*=1..*nops*(*NZ*));

>     print (*t* <> 0)

> **end**;

*launchNZcase* := **proc**(*nz*)

**local** *t*;

**global** *NZ, SV*;

*NZ* := [ seq(*NZ*[ *i* ], *i* = 1 .. *nops*(*NZ*)), convert(*nz*, *string*) ];

*SV* := [ seq(*SV*[ *i* ], *i* = 1 .. *nops*(*SV*)), [ ] ];

    printf ("Launching case level %d:", *nops*(*NZ*) - 1);

    print(*nz* ≠ 0);

    printf ("Assume from now on that:");

```

t := mul(psqf(parse(NZ[i], statement)), i = 1 .. nops(NZ));
print(t ≠ 0)

```

**end proc**

```

> contradict := proc (eq)
>   global NZ, SV, alph;
>   local t, EF, i, sv, nz;
>   t := mul (psqf (parse (NZ[i], statement)), i=1..nops(NZ));
>   EF := efactors (psqf (psqf (eq) / t));
>   if EF[1] = 0 or nops (EF[2]) > 0 then
>     error "No contradiction: 'eq' might be zero!"
>   fi;
>   printf ("Contradiction on case level %d, so:", nops(NZ) - 1);
>   for i from 1 to nops(SV[nops(SV)]) do
>     sv := cat (SV[nops(SV)][i], " := ");
>     sv := cat (sv, SV[nops(SV)][i], "");
>     parse (sv, statement)
>   od;
>   nz := parse (NZ[nops(NZ)], statement);
>   print (nz = 0);
>   if nops(SV[nops(SV)]) > 0 then
>     printf ("Variables to be uneliminated:");
>     for i from 1 to nops(SV[nops(SV)]) do
>       sv := cat (SV[nops(SV)][i], " := ");
>       sv := cat (sv, SV[nops(SV)][i], "");
>       print (sv);
>     od
>   fi;
>   if nops(NZ) <= 1 then
>     printf ("That is all, folks! ");
>     printf ("Check that all variables are uneliminated:");
>     print (alph);
>     return
>   fi;
>   NZ := [seq(NZ[i], i=1..nops(NZ)-1)];
>   SV := [seq(SV[i], i=1..nops(SV)-1)];
>   printf ("Proceed on case level %d with:", nops(NZ) - 1);
>   t := mul (psqf (parse (NZ[i], statement)), i=1..nops(NZ));
>   print (t <> 0);
>   printf ("On account of:");
>   print (nz = 0);
>   if nargs = 1 and nops(indets(nz)) = 1 and degree (nz) = 1 then
>     EF := efactors (psqf (psqf (coeff (nz, indets(nz)[1])) / t));
>     if nops (EF[2]) = 0 then
>       elimsolve(nz, indets(nz)[1]);
>       return
>     fi;
>   fi;

```

```

>   elif nargs > 1 then
>       elimsolve (nz, args[2]);
>       return
>   fi;
>   printf ("the following return value %s",
>           "can be used as an equation:");
>   return nz
> end;

contradict := proc(eq)
local t, EF, i, sv, nz;
global NZ, SV, alph;

    t := mul(psqf(parse(NZ[i], statement)), i = 1 .. nops(NZ));
    EF := efactors(psqf(psqf(eq) / t));
    if EF[1] = 0 or 0 < nops(EF[2]) then error "No contradiction: 'eq' might be zero!"
    end if;
    printf("Contradiction on case level %d, so:", nops(NZ) - 1);
    for i to nops(SV[nops(SV)]) do
        sv := cat(SV[nops(SV)][i], " := ");
        sv := cat(sv, SV[nops(SV)][i], "");
        parse(sv, statement)
    end do;
    nz := parse(NZ[nops(NZ)], statement);
    print(nz = 0);
    if 0 < nops(SV[nops(SV)]) then
        printf("Variables to be uneliminated:");
        for i to nops(SV[nops(SV)]) do
            sv := cat(SV[nops(SV)][i], " := ");
            sv := cat(sv, SV[nops(SV)][i], "");
            print(sv)
        end do
    end if;
    if nops(NZ) ≤ 1 then
        printf("That is all, folks! ");
        printf("Check that all variables are uneliminated:");
        print(alph);
        return
    end if;
    NZ := [seq(NZ[i], i = 1 .. nops(NZ) - 1)];
    SV := [seq(SV[i], i = 1 .. nops(SV) - 1)];
    printf("Proceed on case level %d with:", nops(NZ) - 1);

```

```

t := mul(psqf(parse(NZ[i], statement)), i = 1 .. nops(NZ));
print(t ≠ 0);
printf("On account of:");
print(nz = 0);
if nargs = 1 and nops(indets(nz)) = 1 and degree(nz) = 1 then
    EF := efactors(psqf(psqf(coeff(nz, indets(nz)[1])) / t));
    if nops(EF[2]) = 0 then elimsolve(nz, indets(nz)[1]); return end if
elif 1 < nargs then elimsolve(nz, args[2]); return
end if;
printf("the following return value %s", "can be used as an equation:");
return nz

```

**end proc**

```

> elimsolve := proc (eq, v)
>   global NZ, SV;
>   local t, EF, i, c1, c0, NZref, sv, F;
>   if not ({v} subset indets(v)) then
>     error "Second argument 'v' is not a variable!";
>   fi;
>   t := mul (psqf (parse (NZ[i], statement)), i=1..nops(NZ));
>   EF := efactors (psqf (psqf (eq) / t));
>   if EF[1] = 0 then error "First argument 'eq' is zero!" fi;
>   if nops(EF[2]) = 0 then
>     error "Contradiction: call 'contradict'!"
>   fi;
>   if nops(EF[2]) > 1 then
>     error "'eq' has different factors which may be zero!"
>   fi;
>   if degree (EF[2][1][1], v) <> 1 then
>     error "Degree of 'eq' w.r.t 'v' is not one!"
>   fi;
>   c1 := coeff(EF[2][1][1], v, 1);
>   c0 := coeff(EF[2][1][1], v, 0);
>   EF := efactors (psqf (psqf (c1) / t));
>   if nops(EF[2]) > 0 then
>     error "Coefficient of 'v' in 'eq' might be zero!"
>   fi;
>   EF := efactors (psqf (psqf (denom(eq)) / t));
>   if nops(EF[2]) > 0 then
>     error "Denominator of argument 'eq' may be zero!"
>   fi;
>   print ({c1 <> 0});
>   NZref := false;
>   for i from 1 to nops(NZ) do
>     NZref :=

```

```

>      NZref or ({v} subset indets (parse (NZ[i],statement)));
> od;
> sv := convert (v, string);
> F := factor (-c0/c1);
> SV[nops(SV)] :=
>   [sv, seq(SV[nops(SV)][i], i=1..nops(SV[nops(SV)]))];
> printf ("%s is set to:", sv);
> sv := cat (sv, " := ", convert (F, string));
> print (parse (sv,statement));
> if NZref then
>   printf ("Nonzero constraint refines to:");
>   t := mul (psqf (parse (NZ[i],statement)), i=1..nops (NZ));
>   print (t <> 0)
> fi;
> return
> end;

```

*elimsolve* := **proc**(eq, v)

**local** t, EF, i, c1, c0, NZref, sv, F;

**global** NZ, SV;

**if not** {v} subset indets(v) **then error** "Second argument 'v' is not a variable!" **end if**;

t := mul(psqf(parse(NZ[i], statement)), i = 1 .. nops(NZ));

EF := efactors(psqf(psqf(eq) / t));

**if** EF[1] = 0 **then error** "First argument 'eq' is zero!" **end if**;

**if** nops(EF[2]) = 0 **then error** "Contradiction: call 'contradict'!" **end if**;

**if** 1 < nops(EF[2]) **then error** "'eq' has different factors which may be zero!" **end if**;

**if** degree(EF[2][1][1], v) ≠ 1 **then error** "Degree of 'eq' w.r.t 'v' is not one!" **end if**;

c1 := coeff(EF[2][1][1], v, 1);

c0 := coeff(EF[2][1][1], v, 0);

EF := efactors(psqf(psqf(c1) / t));

**if** 0 < nops(EF[2]) **then error** "Coefficient of 'v' in 'eq' might be zero!" **end if**;

EF := efactors(psqf(psqf(denom(eq)) / t));

**if** 0 < nops(EF[2]) **then error** "Denominator of argument 'eq' may be zero!" **end if**;

print({c1 ≠ 0});

NZref := false;

**for** i **to** nops(NZ) **do** NZref := NZref **or** {v} subset indets(parse(NZ[i], statement))

**end do**;

sv := convert(v, string);

F := factor(-c0 / c1);

SV[nops(SV)] := [sv, seq(SV[nops(SV)][i], i = 1 .. nops(SV[nops(SV)]))];

printf ("%s is set to:", sv);

sv := cat(sv, " := ", convert(F, string));

```

print(parse(sv, statement));
if NZref then
    printf("Nonzero constraint refines to:");
    t := mul(psqf(parse(NZ[i], statement)), i = 1 .. nops(NZ));
    print(t ≠ 0)
end if;
return

```

end proc

```

> initcpcoeff := proc (cp)
>   global x1, x2, x3, x4, x5, x6, T, S, n;
>   local deg0, deg1, deg2, deg3, deg4, deg5, deg6,
>         cp1, cp2, cp3, cp4, cp5, cp6;
>   S := Array (0..(deg-1)*n, 0..(deg-1)*n, 0..(deg-1)*n,
>              0..(deg-1)*n, 0..(deg-1)*n, 0..(deg-1)*n, 0..n,
>              storage=sparse);
>   for deg0 from 0 to n-1 do
>     cp1 := coeff (cp, T, deg0);
>     for deg1 from 0 to (deg-1)*(n-deg0) do
>       cp2 := coeff (cp1, x1, deg1);
>       for deg2 from 0 to (deg-1)*(n-deg0)-deg1 do
>         cp3 := coeff (cp2, x2, deg2);
>         for deg3 from 0 to (deg-1)*(n-deg0)-deg1-deg2 do
>           cp4 := coeff (cp3, x3, deg3);
>           for deg4 from 0 to (deg-1)*(n-deg0)-deg1-deg2-deg3 do
>             cp5 := coeff (cp4, x4, deg4);
>             for deg5 from 0 to (deg-1)*(n-deg0)
>               -deg1-deg2-deg3-deg4 do
>               cp6 := coeff (cp5, x5, deg5);
>               deg6 := (deg-1)*(n-deg0)
>                 -deg1-deg2-deg3-deg4-deg5;
>               S[deg0,deg1,deg2,deg3,deg4,deg5,deg6] :=
>                 coeff (cp6, x6, deg6);
>             od
>           od
>         od
>       od
>     od;
>   return;
> end;

```

initcpcoeff := proc(cp)

local deg0, deg1, deg2, deg3, deg4, deg5, deg6, cp1, cp2, cp3, cp4, cp5, cp6;

global x1, x2, x3, x4, x5, x6, T, S, n;

S := Array(0 .. (deg - 1)\*n, 0 .. (deg - 1)\*n, 0 .. (deg - 1)\*n, 0 .. (deg - 1)\*n,

```

    0 .. (deg - 1)*n, 0 .. (deg - 1)*n, 0 .. n, storage = sparse);
for deg0 from 0 to n - 1 do
    cp1 := coeff(cp, T, deg0);
    for deg1 from 0 to (deg - 1)*(n - deg0) do
        cp2 := coeff(cp1, x1, deg1);
        for deg2 from 0 to (deg - 1)*(n - deg0) - deg1 do
            cp3 := coeff(cp2, x2, deg2);
            for deg3 from 0 to (deg - 1)*(n - deg0) - deg1 - deg2 do
                cp4 := coeff(cp3, x3, deg3);
                for deg4 from 0 to (deg - 1)*(n - deg0) - deg1 - deg2 - deg3 do
                    cp5 := coeff(cp4, x4, deg4);
                    for deg5 from 0 to
                        (deg - 1)*(n - deg0) - deg1 - deg2 - deg3 - deg4 do
                        cp6 := coeff(cp5, x5, deg5);
                        deg6 := (deg - 1)*(n - deg0) - deg1 - deg2 - deg3
                            - deg4 - deg5;
                        S[deg0, deg1, deg2, deg3, deg4, deg5, deg6] :=
                            coeff(cp6, x6, deg6)
                    end do
                end do
            end do
        end do
    end do
end do;
return

```

**end proc**

```

> cpcoeff := proc (t)
>   global x1, x2, x3, x4, x5, x6, T, S;
>   local deg0, deg1, deg2, deg3, deg4, deg5, deg6;
>   deg0 := degree (t, T);
>   deg1 := degree (t, x1);
>   deg2 := degree (t, x2);
>   deg3 := degree (t, x3);
>   deg4 := degree (t, x4);
>   deg5 := degree (t, x5);
>   deg6 := degree (t, x6);
>   factor (S[deg0, deg1, deg2, deg3, deg4, deg5, deg6]) ;
> end;

```

*cpcoeff* := proc(*t*)

local *deg0, deg1, deg2, deg3, deg4, deg5, deg6*;

global *x1, x2, x3, x4, x5, x6, T, S*;



```

deg0 := degree(t, T);
deg1 := degree(t, x1);
deg2 := degree(t, x2);
deg3 := degree(t, x3);
deg4 := degree(t, x4);
deg5 := degree(t, x5);
deg6 := degree(t, x6);
factor(S[deg0, deg1, deg2, deg3, deg4, deg5, deg6])

```

**end proc**

```

> cpCoeff := proc (t)
>   global x1, x2, x3, x4, x5, x6, T, S;
>   local deg0, deg1, deg2, deg3, deg4, deg5, deg6;
>   deg0 := degree (t, T);
>   deg1 := degree (t, x1);
>   deg2 := degree (t, x2);
>   deg3 := degree (t, x3);
>   deg4 := degree (t, x4);
>   deg5 := degree (t, x5);
>   deg6 := degree (t, x6);
>   (Factor (numer(S[deg0, deg1, deg2, deg3, deg4, deg5, deg6])) mod 2) /
>   (Factor (denom(S[deg0, deg1, deg2, deg3, deg4, deg5, deg6])) mod 2);
> end;

```

*cpCoeff* := **proc**(*t*)

**local** *deg0, deg1, deg2, deg3, deg4, deg5, deg6*;

**global** *x1, x2, x3, x4, x5, x6, T, S*;

```

deg0 := degree(t, T);
deg1 := degree(t, x1);
deg2 := degree(t, x2);
deg3 := degree(t, x3);
deg4 := degree(t, x4);
deg5 := degree(t, x5);
deg6 := degree(t, x6);

```

Factor(numer(S[deg0, deg1, deg2, deg3, deg4, deg5, deg6])) mod 2 /

Factor(denom(S[deg0, deg1, deg2, deg3, deg4, deg5, deg6])) mod 2

**end proc**

```

> n := 6;

```

*n* := 6

```

> deg := 2;

```

*deg* := 2

```

> alph :=

```

```

> [[a1, b1, c1, d1, e1, f1, g1, h1, i1, j1, k1, l1, m1, n1, o1],

```

```

> [a2, b2, c2, d2, e2, f2, g2, h2, i2, j2, k2, l2, m2, n2, o2],

```

```

> [a3,b3,c3,d3,e3,f3,g3,h3,i3,j3,k3,l3,m3,n3,o3] ,
> [a4,b4,c4,d4,e4,f4,g4,h4,i4,j4,k4,l4,m4,n4,o4] ,
> [a5,b5,c5,d5,e5,f5,g5,h5,i5,j5,k5,l5,m5,n5,o5] ,
> [a6,b6,c6,d6,e6,f6,g6,h6,i6,j6,k6,l6,m6,n6,o6]] ;

```

```

alph := [[a1,b1,c1,d1,e1,f1,g1,h1,i1,j1,k1,l1,m1,n1,o1],
[a2,b2,c2,d2,e2,f2,g2,h2,i2,j2,k2,l2,m2,n2,o2],
[a3,b3,c3,d3,e3,f3,g3,h3,i3,j3,k3,l3,m3,n3,o3],
[a4,b4,c4,d4,e4,f4,g4,h4,i4,j4,k4,l4,m4,n4,o4],
[a5,b5,c5,d5,e5,f5,g5,h5,i5,j5,k5,l5,m5,n5,o5],
[a6,b6,c6,d6,e6,f6,g6,h6,i6,j6,k6,l6,m6,n6,o6]]

```

```

> terms := [x1*x2,x1*x3,x1*x4,x1*x5,x1*x6,x2*x3,x2*x4,
>           x2*x5,x2*x6,x3*x4,x3*x5,x3*x6,x4*x5,x4*x6,x5*x6] ;

```

```

terms := [x1 x2, x1 x3, x1 x4, x1 x5, x1 x6, x2 x3, x2 x4, x2 x5, x2 x6, x3 x4, x3 x5, x3 x6, x4 x5,
x4 x6, x5 x6]

```

```

> M := evalm ([ [0,0,0,0,0,0], [0,0,0,0,0,0], [0,1,0,0,0,0],
>               [0,0,1,0,0,0], [0,0,0,1,0,0], [0,0,0,0,1,0]] ) ;

```

$$M := \begin{bmatrix} 0 & 0 & 0 & 0 & 0 & 0 \\ 0 & 0 & 0 & 0 & 0 & 0 \\ 0 & 1 & 0 & 0 & 0 & 0 \\ 0 & 0 & 1 & 0 & 0 & 0 \\ 0 & 0 & 0 & 1 & 0 & 0 \\ 0 & 0 & 0 & 0 & 1 & 0 \end{bmatrix}$$

```

> H := Vector (evalm (M &* [x1^2,seq(terms[k],k=1..n-1)] +
> ['add (alph[1,k]*terms[k],k=n..nops(terms)) '$1=1..n])) ;

```

```

H := [f1 x2 x3 + g1 x2 x4 + h1 x2 x5 + i1 x2 x6 + j1 x3 x4 + k1 x3 x5 + l1 x3 x6 + m1 x4 x5
+ n1 x4 x6 + o1 x5 x6, f2 x2 x3 + g2 x2 x4 + h2 x2 x5 + i2 x2 x6 + j2 x3 x4 + k2 x3 x5
+ l2 x3 x6 + m2 x4 x5 + n2 x4 x6 + o2 x5 x6, x1 x2 + f3 x2 x3 + g3 x2 x4 + h3 x2 x5 + i3 x2 x6
+ j3 x3 x4 + k3 x3 x5 + l3 x3 x6 + m3 x4 x5 + n3 x4 x6 + o3 x5 x6, x1 x3 + f4 x2 x3 + g4 x2 x4
+ h4 x2 x5 + i4 x2 x6 + j4 x3 x4 + k4 x3 x5 + l4 x3 x6 + m4 x4 x5 + n4 x4 x6 + o4 x5 x6, x1 x4
+ f5 x2 x3 + g5 x2 x4 + h5 x2 x5 + i5 x2 x6 + j5 x3 x4 + k5 x3 x5 + l5 x3 x6 + m5 x4 x5
+ n5 x4 x6 + o5 x5 x6, x1 x5 + f6 x2 x3 + g6 x2 x4 + h6 x2 x5 + i6 x2 x6 + j6 x3 x4 + k6 x3 x5
+ l6 x3 x6 + m6 x4 x5 + n6 x4 x6 + o6 x5 x6]

```

```

> with (linalg):

```

```

Warning, the protected names norm and trace have been redefined and
unprotected

```

```

> JH := jacobian (H,[x1,x2,x3,x4,x5,x6]):

```

```

> cp := Expand (det (T-JH)-T^n) mod 2:

```

```

> initcpcoeff (cp);

```

```

> initcases (1);

```

```

We assume the following in our calculation:

```

$$1 \neq 0$$

```

> for i from 1 by -1 to 0 do

```

```

>   for j from 1-i by -1 to 0 do

```

```

> for k from 0 to 1-i-j do
>   v := coeff (coeff (coeff (coeff (coeff (coeff (H[6],
>     x1,0),x2,i),x3,j),x4,k),x5,1-i-j-k),x6,1);
>   m := cpCoeff (x1^0 * x2^i * x3^j * x4^k *
>     x5^(1-i-j-k) * T^5);
>   elimsolve (m,v);
> od;
> od;
> od;

```

$\{1 \neq 0\}$

i6 is set to:

$-f3 - g4 - h5$

$\{1 \neq 0\}$

l6 is set to:

$-f2 - j4 - k5$

$\{1 \neq 0\}$

o6 is set to:

$-h2 - k3 - m4$

$\{1 \neq 0\}$

n6 is set to:

$-j3 - g2 - m5$

```

> for i from 1 by -1 to 0 do
>   for j from 1-i by -1 to 0 do
>     for k from 0 to 1-i-j do
>       v := coeff (coeff (coeff (coeff (coeff (coeff (H[5],
>         x1,0),x2,i),x3,j),x4,k),x5,1-i-j-k),x6,1);
>       m := cpCoeff (x1^1 * x2^i * x3^j * x4^k *
>         x5^(1-i-j-k) * T^4);
>       elimsolve (m,v);
>     od;
>   od;
> od;

```

$\{1 \neq 0\}$

i5 is set to:

$-f2 - g3 - h4$

$\{1 \neq 0\}$

l5 is set to:

$-j3 - k4$

$\{1 \neq 0\}$

o5 is set to:

$-k2 - m3$

$\{1 \neq 0\}$

n5 is set to:

$-j2 - m4$

```

> for i from 1 by -1 to 0 do

```

```

> for j from 1-i by -1 to 0 do
>   for k from 0 to 1-i-j do
>     v := coeff (coeff (coeff (coeff (coeff (coeff (H[4],
>       x1,0),x2,i),x3,j),x4,k),x5,1-i-j-k),x6,1);
>     m := cpCoeff (x1^2 * x2^i * x3^j * x4^k *
>       x5^(1-i-j-k) * T^3);
>     elimsolve (m,v);
>   od;
> od;
> od;

```

$\{1 \neq 0\}$

i4 is set to:

$-h3 - g2$

$\{1 \neq 0\}$

l4 is set to:

$-k3 - j2$

$\{1 \neq 0\}$

o4 is set to:

$-m2$

$\{1 \neq 0\}$

n4 is set to:

$-m3$

```

> for i from 1 by -1 to 0 do
>   for j from 1-i by -1 to 0 do
>     for k from 0 to 1-i-j do
>       v := coeff (coeff (coeff (coeff (coeff (coeff (H[3],
>         x1,0),x2,i),x3,j),x4,k),x5,1-i-j-k),x6,1);
>       m := cpCoeff (x1^3 * x2^i * x3^j * x4^k *
>         x5^(1-i-j-k) * T^2);
>       elimsolve (m,v);
>     od;
>   od;
> od;

```

$\{1 \neq 0\}$

i3 is set to:

$-h2$

$\{1 \neq 0\}$

l3 is set to:

$-k2$

$\{1 \neq 0\}$

o3 is set to:

0

$\{1 \neq 0\}$

n3 is set to:

$-m2$

```

> for i from 1 by -1 to 0 do
>   for j from 1-i by -1 to 0 do
>     for k from 0 to 1-i-j do
>       v := coeff (coeff (coeff (coeff (coeff (H[2],
>         x1,0),x2,i),x3,j),x4,k),x5,1-i-j-k),x6,1);
>       m := cpCoeff (x1^4 * x2^i * x3^j * x4^k *
>         x5^(1-i-j-k) * T);
>       elimsolve (m,v);
>     od;
>   od;
> od;

```

$\{1 \neq 0\}$

i2 is set to:

0

$\{1 \neq 0\}$

l2 is set to:

0

$\{1 \neq 0\}$

o2 is set to:

0

$\{1 \neq 0\}$

n2 is set to:

0

```

> tmp1 := cpCoeff (x2^2*T^4);

```

$tmp1 := f6 h2 + h5 f3 + f5 h3 + f4 g3 + f3 g4 + f1 + f3^2 + g6 h3 + g6 g2 + h4 g5 + h5 g4 + h5^2 + g4^2 + h6 f2 + h6 g3 + h6 h4$

```

> elimsolve (tmp1,f1);

```

$\{1 \neq 0\}$

f1 is set to:

$-f6 h2 - h5 f3 - f5 h3 - f4 g3 - f3 g4 - f3^2 - g6 h3 - g6 g2 - h4 g5 - h5 g4 - h5^2 - g4^2 - h6 f2 - h6 g3 - h6 h4$

```

> tmp1 := cpCoeff (x2*x3*T^4);

```

$tmp1 := f3 k5 + f5 k3 + f4 j3 + h4 j5 + h5 j4 + h3 j6 + f3 j4 + g2 j6 + f2 g4 + g6 j2 + k5 g4 + k4 g5 + f4 g2 + g1 + f6 k2 + f5 h2 + g3 k6 + k6 f2 + k3 g6 + k6 h4 + h6 j3 + h6 k4 + f2 h5$

```

> elimsolve (tmp1,g1);

```

$\{1 \neq 0\}$

g1 is set to:

$-f3 k5 - f5 k3 - f4 j3 - h4 j5 - h5 j4 - h3 j6 - f3 j4 - g2 j6 - f2 g4 - g6 j2 - k5 g4 - k4 g5 - f4 g2 - f6 k2 - f5 h2 - g3 k6 - k6 f2 - k3 g6 - k6 h4 - h6 j3 - h6 k4 - f2 h5$

```

> tmp1 := cpCoeff (x3^2*T^4);

```

$tmp1 :=$

$f4 j2 + f2 k5 + f2 j4 + f2^2 + j1 + f5 k2 + j6 k3 + j6 j2 + k4 j5 + k6 j3 + k6 k4 + k5 j4 + k5^2 + j4^2$

```

> elimsolve (tmp1,j1);

```

$\{1 \neq 0\}$

j1 is set to:

$$-f4 j2 - f2 k5 - f2 j4 - f2^2 - f5 k2 - j6 k3 - j6 j2 - k4 j5 - k6 j3 - k6 k4 - k5 j4 - k5^2 - j4^2$$

> **tmp1 := cpCoeff (x2\*x4\*T^4);**

$$\begin{aligned} tmp1 := & k6 j3 + k6 k4 + j6 k3 + g3 j4 + g4 m5 + g5 m4 + j3 g4 + h6 m4 + h3 j5 + k5 j4 + k4 j5 \\ & + j3 h5 + h2 g5 + f3 m5 + h4 m6 + f2 g3 + f2 j4 + f3 g2 + h5 g2 + h1 + f2 k5 + f5 k2 + f4 j2 \\ & + j6 j2 + k5^2 + j4^2 + f2^2 + h6 j2 + j6 h2 + g6 m3 + m6 f2 + m6 g3 + f6 m2 + f5 m3 \end{aligned}$$

> **elimsolve (tmp1,h1);**

$\{1 \neq 0\}$

h1 is set to:

$$\begin{aligned} & -k6 j3 - k6 k4 - j6 k3 - g3 j4 - g4 m5 - g5 m4 - j3 g4 - h6 m4 - h3 j5 - k5 j4 - k4 j5 - j3 h5 \\ & - h2 g5 - f3 m5 - h4 m6 - f2 g3 - f2 j4 - f3 g2 - h5 g2 - f2 k5 - f5 k2 - f4 j2 - j6 j2 - k5^2 \\ & - j4^2 - f2^2 - h6 j2 - j6 h2 - g6 m3 - m6 f2 - m6 g3 - f6 m2 - f5 m3 \end{aligned}$$

> **tmp1 := cpCoeff (x3\*x4\*T^4);**

$$\begin{aligned} tmp1 := & m6 k4 + m6 j3 + j6 m3 + j6 k2 + k6 m4 + k6 j2 + j5 m4 + g2 k5 + g5 k2 + f3 j2 + f2 j3 \\ & + j5 k3 + j3 k5 + g4 j2 + g2 j4 + f2 m5 + f5 m2 + j4 m5 + k1 \end{aligned}$$

> **elimsolve (tmp1,k1);**

$\{1 \neq 0\}$

k1 is set to:

$$\begin{aligned} & -m6 k4 - m6 j3 - j6 m3 - j6 k2 - k6 m4 - k6 j2 - j5 m4 - g2 k5 - g5 k2 - f3 j2 - f2 j3 - j5 k3 \\ & - j3 k5 - g4 j2 - g2 j4 - f2 m5 - f5 m2 - j4 m5 \end{aligned}$$

> **tmp1 := cpCoeff (x4^2\*T^4);**

$$\begin{aligned} tmp1 := & g2 j3 + g3 j2 + j6 m2 + g2 m5 + g2^2 + j3 m5 + j3^2 + j5 m3 + g5 m2 + m1 + m6 j2 \\ & + m6 m4 + m5^2 \end{aligned}$$

> **elimsolve (tmp1,m1);**

$\{1 \neq 0\}$

m1 is set to:

$$-g2 j3 - g3 j2 - j6 m2 - g2 m5 - g2^2 - j3 m5 - j3^2 - j5 m3 - g5 m2 - m6 j2 - m6 m4 - m5^2$$

> **tmp1 := cpCoeff (x2\*x5\*T^4);**

$$\begin{aligned} tmp1 := & m6 k4 + m6 j3 + j6 m3 + j6 k2 + k6 m4 + k6 j2 + h2 k6 + h6 k2 + h6 m3 + m6 h3 \\ & + m6 g2 + g6 m2 + j5 m4 + f4 m3 + f3 m4 + g2 k5 + g5 k2 + g3 k4 + g4 k3 + k5 h3 + h5 m4 \\ & + k3 h5 + h4 m5 + g2 h4 + g4 h2 + h2 f3 + h3 f2 + f3 j2 + f2 j3 + j5 k3 + j3 k5 + g4 j2 + g2 j4 \\ & + f2 m5 + f5 m2 + j4 m5 + i1 \end{aligned}$$

> **elimsolve (tmp1,i1);**

$\{1 \neq 0\}$

i1 is set to:

$$\begin{aligned} & -m6 k4 - m6 j3 - j6 m3 - j6 k2 - k6 m4 - k6 j2 - h2 k6 - h6 k2 - h6 m3 - m6 h3 - m6 g2 \\ & - g6 m2 - j5 m4 - f4 m3 - f3 m4 - g2 k5 - g5 k2 - g3 k4 - g4 k3 - k5 h3 - h5 m4 - k3 h5 \\ & - h4 m5 - g2 h4 - g4 h2 - h2 f3 - h3 f2 - f3 j2 - f2 j3 - j5 k3 - j3 k5 - g4 j2 - g2 j4 - f2 m5 \\ & - f5 m2 - j4 m5 \end{aligned}$$

> **tmp1 := cpCoeff (x3\*x5\*T^4);**

```

tmp1 := j3^2 + g2^2 + m5^2 + m6 m4 + h2 k5 + f2 k3 + f3 k2 + j3 m5 + j5 m3 + g2 m5 + g3 j2
      + g5 m2 + k4 m5 + k5 m4 + h2 j4 + m6 k3 + k6 m3 + j4 k3 + j3 k4 + g2 j3 + h5 k2 + h4 j2
      + f2 m4 + l1 + f4 m2

```

```

> elimsolve (tmp1,l1);

```

{1 ≠ 0}

l1 is set to:

```

-j3^2 - g2^2 - m5^2 - m6 m4 - h2 k5 - f2 k3 - f3 k2 - j3 m5 - j5 m3 - g2 m5 - g3 j2 - g5 m2
- k4 m5 - k5 m4 - h2 j4 - m6 k3 - k6 m3 - j4 k3 - j3 k4 - g2 j3 - h5 k2 - h4 j2 - f2 m4
- f4 m2

```

```

> tmp1 := cpCoeff (x4*x5*T^4);

```

```

tmp1 := g2 k3 + g3 k2 + k3 m5 + k5 m3 + h2 m5 + h5 m2 + j4 m3 + j3 m4 + g4 m2 + h3 j2
      + h2 j3 + m6 k2 + m2 k6 + n1 + g2 m4

```

```

> elimsolve (tmp1,n1);

```

{1 ≠ 0}

n1 is set to:

```

-g2 k3 - g3 k2 - k3 m5 - k5 m3 - h2 m5 - h5 m2 - j4 m3 - j3 m4 - g4 m2 - h3 j2 - h2 j3
- m6 k2 - m2 k6 - g2 m4

```

```

> tmp1 := cpCoeff (x5^2*T^4);

```

```

tmp1 := h4 m2 + h2 m4 + h2 k3 + k3 m4 + h3 k2 + k4 m3 + k3^2 + h2^2 + o1 + m6 m2 + m4^2

```

```

> elimsolve (tmp1,o1);

```

{1 ≠ 0}

o1 is set to:

```

-h4 m2 - h2 m4 - h2 k3 - k3 m4 - h3 k2 - k4 m3 - k3^2 - h2^2 - m6 m2 - m4^2

```

```

> launchNZcase (m2);

```

Launching case level 1:

m2 ≠ 0

Assume from now on that:

m2 ≠ 0

```

> tmp1 := cpCoeff (x3*x6*T^4);

```

```

tmp1 := j2 m5 + j5 m2 + h2 m5 + h5 m2 + h2 k4 + h4 k2 + k4 j2 + k2 j4 + g4 m2 + m6 k2
      + m2 k6 + g2 m4

```

```

> elimsolve (tmp1,g4);

```

{m2 ≠ 0}

g4 is set to:

```

_ j2 m5 + j5 m2 + h2 m5 + h5 m2 + h2 k4 + h4 k2 + k4 j2 + k2 j4 + m6 k2 + m2 k6 + g2 m4
  m2

```

```

> tmp1 := cpCoeff (x4*x6*T^4);

```

tmp1 :=

```

g3 m2 + g2 m3 + h2 k3 + h3 k2 + k2 m5 + k5 m2 + m4^2 + h2^2 + k3^2 + m6 m2 + k2 j3 + j2 k3

```

```

> elimsolve (tmp1,g3);

```

{m2 ≠ 0}

g3 is set to:

$$- \frac{g2 m3 + h2 k3 + h3 k2 + k2 m5 + k5 m2 + m4^2 + h2^2 + k3^2 + m6 m2 + k2 j3 + j2 k3}{m2}$$

> **tmp1 := cpCoeff (x5\*x6\*T^4);**

$$tmp1 := m3 j2 + m2 j3 + h2 m3 + h3 m2 + k4 m2 + k2 m4$$

> **elimsolve (tmp1,j3);**

$$\{m2 \neq 0\}$$

j3 is set to:

$$- \frac{m3 j2 + h2 m3 + h3 m2 + k4 m2 + k2 m4}{m2}$$

> **tmp1 := cpCoeff (x6^2\*T^4);**

$$tmp1 := k2 m3 + m2 k3 + k2^2 + m2 m4 + m3^2$$

> **elimsolve (tmp1,k3);**

$$\{m2 \neq 0\}$$

k3 is set to:

$$- \frac{k2 m3 + k2^2 + m2 m4 + m3^2}{m2}$$

> **tmp1 := cpCoeff (x1\*x6^2\*T^3);**

$$tmp1 := m2 m3$$

> **elimsolve (tmp1,m3);**

$$\{1 \neq 0\}$$

m3 is set to:

$$0$$

> **tmp1 := cpCoeff (x1\*x2\*x3\*T^3);**

$$\begin{aligned} tmp1 := & (m6 h2 m2 k2^2 + m6 m2^2 j2 m4 + m6 m2 j2 k2^2 + m6 h2 m2^2 m4 + k4 m2^2 h4 k2 \\ & + k2 m4 j5 m2^2 + k2 m4 m2^2 k6 + m5 m2^2 g2 m4 + m5 m2^2 h4 k2 + g6 k2 m2^3 + g5 m4 m2^3 \\ & + k6 k4 m2^3 + f2 h4 m2^3 + k4 j5 m2^3 + k5 j4 m2^3 + h4 m6 m2^3 + f3 k4 m2^3 + f3 m5 m2^3 \\ & + h2 g5 m2^3 + f4 h2 m2^3 + h5 g2 m2^3 + f2 j4 m2^3 + f4 j2 m2^3 + k5 m6 m2^3 + m2 k2 m4 j2 m5 \\ & + m2 k2 m4 h2 k4 + m2 k2 m4 h2 m5 + m2 k2^2 m4 h4 + m2 k2 m4 k4 j2 + m6 f2 m2^3 \\ & + k4 m2^3 h5 + k4^2 m2^2 h2 + k4^2 m2^2 j2 + g5 m2^3 j2 + h6 m2^2 k2^2 + f4 m2^3 m4 + f4 m2^2 k2^2 \\ & + j4 m6 m2^3 + j4 h2^2 m2^2 + m5^2 m2^2 h2 + m5 m2^3 j5 + m5^2 m2^2 j2 + m5 m2^3 k6 + m5 m2^3 h5 \\ & + j5 m2^3 g2 + m6 h2^2 m2^2 + k6 m2^3 g2 + h4 m2^3 k5 + h3 m2^2 h2 m5 + j4 m2^2 j2 m4 \\ & + j4 m2 j2 k2^2 + j4 h2 m2^2 m4 + j4 h2 m2 k2^2 + m2 k2 m4^2 g2 + h3 m2^2 h2 k4 + h3 m2^2 m6 k2 \\ & + h3 m2^2 j2 m5 + h3 m2^2 h4 k2 + h3 m2^2 k2 j4 + h3 m2^2 k4 j2 + m6^2 m2^3 + m6 k2^4 \\ & + h3 m2^2 g2 m4 + j4 k2^4 + f6 m2^4 + k4 m2^2 g2 m4) / m2^3 \end{aligned}$$

> **elimsolve (tmp1,f6);**

$$\{m2^4 \neq 0\}$$

f6 is set to:

$$\begin{aligned} - & (m6 h2 m2 k2^2 + m6 m2^2 j2 m4 + m6 m2 j2 k2^2 + m6 h2 m2^2 m4 + k4 m2^2 h4 k2 \\ & + k2 m4 j5 m2^2 + k2 m4 m2^2 k6 + m5 m2^2 g2 m4 + m5 m2^2 h4 k2 + g6 k2 m2^3 + g5 m4 m2^3 \\ & + k6 k4 m2^3 + f2 h4 m2^3 + k4 j5 m2^3 + k5 j4 m2^3 + h4 m6 m2^3 + f3 k4 m2^3 + f3 m5 m2^3 \end{aligned}$$



$$\begin{aligned}
& + h2 g5 m2^3 + f4 h2 m2^3 + h5 g2 m2^3 + f2 j4 m2^3 + f4 j2 m2^3 + k5 m6 m2^3 + m2 k2 m4 j2 m5 \\
& + m2 k2 m4 h2 k4 + m2 k2 m4 h2 m5 + m2 k2^2 m4 h4 + m2 k2 m4 k4 j2 + m6 f2 m2^3 \\
& + k4 m2^3 h5 + k4^2 m2^2 h2 + k4^2 m2^2 j2 + g5 m2^3 j2 + h6 m2^2 k2^2 + f4 m2^3 m4 + f4 m2^2 k2^2 \\
& + j4 m6 m2^3 + j4 h2^2 m2^2 + m5^2 m2^2 h2 + m5 m2^3 j5 + m5^2 m2^2 j2 + m5 m2^3 k6 + m5 m2^3 h5 \\
& + j5 m2^3 g2 + m6 h2^2 m2^2 + k6 m2^3 g2 + h4 m2^3 k5 + h3 m2^2 h2 m5 + j4 m2^2 j2 m4 \\
& + j4 m2 j2 k2^2 + j4 h2 m2^2 m4 + j4 h2 m2 k2^2 + m2 k2 m4^2 g2 + h3 m2^2 h2 k4 + h3 m2^2 m6 k2 \\
& + h3 m2^2 j2 m5 + h3 m2^2 h4 k2 + h3 m2^2 k2 j4 + h3 m2^2 k4 j2 + m6^2 m2^3 + m6 k2^4 \\
& + h3 m2^2 g2 m4 + j4 k2^4 + k4 m2^2 g2 m4) / m2^4
\end{aligned}$$

> **tmp1 := cpCoeff (x1\*x3^2\*T^3) ;**

$$\begin{aligned}
tmp1 := & (f4 k2 m2 + f2 k4 m2 + k6 j2 m2 + j4 m5 m2 + f2 m5 m2 + g2 j4 m2 + g5 k2 m2 \\
& + g2 k5 m2 + m6 k2 m4 + m6 h3 m2 + j2 h2 k4 + j2 h5 m2 + j2 h2 m5 + k2 m4 k5 + j2 m6 k2 \\
& + j2 k2 j4 + j2 h4 k2 + j2 g2 m4 + j5 k2^2 + f5 m2^2 + k5 h3 m2 + k4 j2^2 + j2^2 m5 + k6 k2^2) / m2
\end{aligned}$$

> **elimsolve (tmp1,f5) ;**

$$\{m2^2 \neq 0\}$$

f5 is set to:

$$\begin{aligned}
- & (f4 k2 m2 + f2 k4 m2 + k6 j2 m2 + j4 m5 m2 + f2 m5 m2 + g2 j4 m2 + g5 k2 m2 + g2 k5 m2 \\
& + m6 k2 m4 + m6 h3 m2 + j2 h2 k4 + j2 h5 m2 + j2 h2 m5 + k2 m4 k5 + j2 m6 k2 + j2 k2 j4 \\
& + j2 h4 k2 + j2 g2 m4 + j5 k2^2 + k5 h3 m2 + k4 j2^2 + j2^2 m5 + k6 k2^2) / m2^2
\end{aligned}$$

> **tmp1 := cpCoeff (x1\*x4^2\*T^3) ;**

$$\begin{aligned}
tmp1 := & (h2 m2 k2^3 + k2 h2^2 m2^2 + k2 k5 m2^3 + m2 j2 k2^3 + k2^2 m2^2 k4 + k2^3 m2 m4 \\
& + m2^3 h2 k4 + m2^3 h2 h3 + m2^3 g2 m4 + m2^2 g2 k2^2 + h3 j2 m2^3 + h2 m5 m2^3 + m2^2 j2 m4 k2 \\
& + k2^5 + h5 m2^4 + m2^4 k6) / m2^3
\end{aligned}$$

> **elimsolve (tmp1,h5) ;**

$$\{m2^4 \neq 0\}$$

h5 is set to:

$$\begin{aligned}
- & (h2 m2 k2^3 + k2 h2^2 m2^2 + k2 k5 m2^3 + m2 j2 k2^3 + k2^2 m2^2 k4 + k2^3 m2 m4 + m2^3 h2 k4 \\
& + m2^3 h2 h3 + m2^3 g2 m4 + m2^2 g2 k2^2 + h3 j2 m2^3 + h2 m5 m2^3 + m2^2 j2 m4 k2 + k2^5 \\
& + m2^4 k6) / m2^4
\end{aligned}$$

> **tmp1 := cpCoeff (x1\*x2\*x5\*T^3) ;**

$$\begin{aligned}
tmp1 := & (k2^6 + h2^3 m2^3 + m2^4 k4^2 + j6 m2^5 + m5^2 m2^4 + m2^5 h6 + f4 m2^5 + g2^2 m2^4 + m2^4 h3^2 \\
& + k2^2 h2 m2^2 m4 + m6 m4 m2^4 + k2^2 k5 m2^3 + f2 m4 m2^4 + m5 h3 m2^4 + k4 h3 m2^4 \\
& + k2^3 m2^2 k4 + k2^2 m6 m2^3 + k2^4 m2 m4 + k2^2 m4^2 m2^2 + m2^3 m4 h2^2 + m2^4 m4 h4 \\
& + k5 m2^4 h2 + m2^2 g2 k2^3 + k2^2 m2^3 j4 + k2 m2^4 j5 + m2^3 j2 h2^2 + m2^4 j2 k5 + m2^3 j2^2 m4 \\
& + m2^2 j2^2 k2^2 + m5 m2^4 k4 + m2^3 m4 k2 m5 + k2 m5 m2^3 h2 + k2 m2^3 k4 h2 + k2 m2^3 h2 h3 \\
& + k2 m2^3 g2 m4 + k2 h3 j2 m2^3) / m2^4
\end{aligned}$$

> **elimsolve (tmp1,f4) ;**

$$\{m2^5 \neq 0\}$$

f4 is set to:

$$\begin{aligned}
& - (k2^6 + h2^3 m2^3 + m2^4 k4^2 + j6 m2^5 + m5^2 m2^4 + m2^5 h6 + g2^2 m2^4 + m2^4 h3^2 \\
& + k2^2 h2 m2^2 m4 + m6 m4 m2^4 + k2^2 k5 m2^3 + f2 m4 m2^4 + m5 h3 m2^4 + k4 h3 m2^4 \\
& + k2^3 m2^2 k4 + k2^2 m6 m2^3 + k2^4 m2 m4 + k2^2 m4^2 m2^2 + m2^3 m4 h2^2 + m2^4 m4 h4 \\
& + k5 m2^4 h2 + m2^2 g2 k2^3 + k2^2 m2^3 j4 + k2 m2^4 j5 + m2^3 j2 h2^2 + m2^4 j2 k5 + m2^3 j2^2 m4 \\
& + m2^2 j2^2 k2^2 + m5 m2^4 k4 + m2^3 m4 k2 m5 + k2 m5 m2^3 h2 + k2 m2^3 k4 h2 + k2 m2^3 h2 h3 \\
& + k2 m2^3 g2 m4 + k2 h3 j2 m2^3) / m2^5
\end{aligned}$$

> **tmp1 := cpCoeff (x1\*x3\*x5\*T^3);**

$$\begin{aligned}
tmp1 := & (h2 h3 m2 + h2 k2 m4 + k4 m2 j2 + k6 m2^2 + m2 j2 m5 + m2^2 j5 + k2 m2 j4 \\
& + k2 m2 h4 + m2 j2 h3 + m2^2 f3 + m6 k2 m2) / m2
\end{aligned}$$

> **elimsolve (tmp1,f3);**

$$\{m2^2 \neq 0\}$$

f3 is set to:

$$\begin{aligned}
& - (h2 h3 m2 + h2 k2 m4 + k4 m2 j2 + k6 m2^2 + m2 j2 m5 + m2^2 j5 + k2 m2 j4 + k2 m2 h4 \\
& + m2 j2 h3 + m6 k2 m2) / m2^2
\end{aligned}$$

> **tmp1 := cpCoeff (x1\*x4\*x5\*T^3);**

$$tmp1 := \frac{k2 m2 k4 + k2^2 m4 + k2 m2 m5 + m2^2 k5 + m2^2 j4 + k2 m2 h3 + k2^2 j2}{m2}$$

> **elimsolve (tmp1,j4);**

$$\{m2^2 \neq 0\}$$

j4 is set to:

$$- \frac{k2 m2 k4 + k2^2 m4 + k2 m2 m5 + m2^2 k5 + k2 m2 h3 + k2^2 j2}{m2^2}$$

> **tmp1 := cpCoeff (x1\*x5^2\*T^3);**

$$tmp1 := k4 m2 + k2 m4 + m2 m5 + h3 m2$$

> **elimsolve (tmp1,h3);**

$$\{m2 \neq 0\}$$

h3 is set to:

$$- \frac{k4 m2 + k2 m4 + m2 m5}{m2}$$

> **tmp1 := cpCoeff (x1\*x3\*x6\*T^3);**

$$tmp1 := \frac{j2 m4 m2^2 + h2 m2^2 m4 + m2 j2 k2^2 + m6 m2^3 + h2^2 m2^2 + k5 m2^3 + k2^4 + h4 m2^3}{m2^2}$$

> **elimsolve (tmp1,h4);**

$$\{m2^3 \neq 0\}$$

h4 is set to:

$$- \frac{j2 m4 m2^2 + h2 m2^2 m4 + m2 j2 k2^2 + m6 m2^3 + h2^2 m2^2 + k5 m2^3 + k2^4}{m2^3}$$

> **tmp1 := cpCoeff (x1\*x4\*x6\*T^3);**

$$tmp1 := k4 m2 + k2 m4 + m2 m5$$

> **elimsolve (tmp1,k4);**

```

                                {m2 ≠ 0}
k4 is set to:
                                -  $\frac{k2\ m4 + m2\ m5}{m2}$ 
> tmp1 := cpCoeff (x1*x5*x6*T^3);
                                tmp1 := k2^2 + m2 m4
> elimsolve (tmp1,m4);
                                {m2 ≠ 0}
m4 is set to:
                                -  $\frac{k2^2}{m2}$ 
> tmp1 := cpCoeff (x5*x6^2*T^3);
                                tmp1 := m2^2 k5
> elimsolve (tmp1,k5);
                                {1 ≠ 0}
k5 is set to:
                                0
> tmp1 := cpCoeff (x3*x6^2*T^3);
tmp1 :=
                                 $-\frac{m2^2\ h2^3 + m2^2\ j2\ h2^2 + h2\ k2^4 + m2^4\ j6 + m2^4\ h6 + k2^3\ m5\ m2 + m2^4\ g5 + k2\ m2^3\ j5 + k2^4\ j2}{m2^2}$ 
> elimsolve (tmp1,g5);
                                {m2^4 ≠ 0}
g5 is set to:
                                -  $\frac{m2^2\ h2^3 + m2^2\ j2\ h2^2 + h2\ k2^4 + m2^4\ j6 + m2^4\ h6 + k2^3\ m5\ m2 + k2\ m2^3\ j5 + k2^4\ j2}{m2^4}$ 
> tmp1 := cpCoeff (x5^2*x6*T^3);
                                tmp1 := m5 k2^2 + m2^2 j5
> elimsolve (tmp1,j5);
                                {m2^2 ≠ 0}
j5 is set to:
                                -  $\frac{m5\ k2^2}{m2^2}$ 
> tmp1 := cpCoeff (x4*x5*x6*T^3);
                                tmp1 :=  $\frac{(k2^3 + h2\ k2\ m2 + m2^2\ m5 + g2\ m2^2)^2}{m2^3}$ 
> elimsolve (tmp1,g2);
                                {m2^2 ≠ 0}
g2 is set to:
                                -  $\frac{k2^3 + h2\ k2\ m2 + m2^2\ m5}{m2^2}$ 

```

> tmp1 := cpCoeff (x3\*x5\*x6\*T^3);

$$tmp1 := \frac{k2^7 + k2 h2^3 m2^3 + k2^5 h2 m2 + m2^2 k2^3 h2^2 + m5 k2^4 m2^2 + h2^2 m2^4 m5 + g6 m2^6}{m2^4}$$

> elimsolve (tmp1,g6);

$$\{m2^6 \neq 0\}$$

g6 is set to:

$$- \frac{(k2^4 + h2^2 m2^2) (k2^3 + h2 k2 m2 + m2^2 m5)}{m2^6}$$

> tmp1 := cpCoeff (x2\*x3\*x6\*T^3);

$$tmp1 := \frac{(h2 m2 k2^3 + m2^4 k6 + k2 m6 m2^3 + h2 m5 m2^3 + k2^5 + j2 m2^2 h2 k2 + f2 k2 m2^3)^2}{m2^7}$$

> elimsolve (tmp1,k6);

$$\{m2^4 \neq 0\}$$

k6 is set to:

$$- \frac{h2 m2 k2^3 + k2 m6 m2^3 + h2 m5 m2^3 + k2^5 + j2 m2^2 h2 k2 + f2 k2 m2^3}{m2^4}$$

> tmp1 := cpCoeff (x5^4\*T^2);

$$tmp1 := \frac{(j2 m2^2 h2 + h2 m2 k2^2 + k2^4 + k2 m2^2 m5 + f2 m2^3)^2}{m2^4}$$

> elimsolve (tmp1,f2);

$$\{m2^3 \neq 0\}$$

f2 is set to:

$$- \frac{j2 m2^2 h2 + h2 m2 k2^2 + k2^4 + k2 m2^2 m5}{m2^3}$$

> tmp1 := cpCoeff (x4^4\*T^2);

$$tmp1 := \frac{(h2 m2 m5 k2 + j6 m2^3 + m5^2 m2^2 + k2^3 m5 + j2 m2^2 m6)^2}{m2^4}$$

> elimsolve (tmp1, j6);

$$\{m2^3 \neq 0\}$$

j6 is set to:

$$- \frac{h2 m2 m5 k2 + m5^2 m2^2 + k2^3 m5 + j2 m2^2 m6}{m2^3}$$

> launchNZcase (m2\*h2+j2\*m2+k2^2);

Launching case level 2:

$$h2 m2 + j2 m2 + k2^2 \neq 0$$

Assume from now on that:

$$m2 (h2 m2 + j2 m2 + k2^2) \neq 0$$

> tmp1 := cpCoeff (x2^2\*x4^2\*T^2);

tmp1 :=

$$\frac{(h2^3 m2^3 + m2^2 k2^2 h2^2 + k2^4 h2 m2 + m2^5 h6 + k2^2 m6 m2^3 + k2^6)^2 (h2 m2 + j2 m2 + k2^2)^2}{m2^{12}}$$

> **elimsolve** (tmp1,h6);

$$\{m2^5 \neq 0\}$$

h6 is set to:

$$-\frac{h2^3 m2^3 + m2^2 k2^2 h2^2 + k2^4 h2 m2 + k2^2 m6 m2^3 + k2^6}{m2^5}$$

> **tmp1 := cpCoeff** (x1^2\*x2^2\*T^2);

$$tmp1 := \frac{h2^2 (h2 m2 + j2 m2 + k2^2)^2}{m2^4}$$

> **elimsolve** (tmp1,h2);

$$\{1 \neq 0\}$$

h2 is set to:

$$0$$

Nonzero constraint refines to:

$$m2 (j2 m2 + k2^2) \neq 0$$

> **tmp1 := cpCoeff** (x1^2\*x3^2\*T^2);

$$tmp1 := \frac{(j2 m2 + k2^2)^2 k2^2}{m2^4}$$

> **elimsolve** (tmp1,k2);

$$\{1 \neq 0\}$$

k2 is set to:

$$0$$

Nonzero constraint refines to:

$$j2 m2^2 \neq 0$$

> **tmp1 := cpCoeff** (x1^2\*x4^2\*T^2);

$$tmp1 := j2^2$$

> **eq1 := contradict** (tmp1);

Contradiction on case level 2, so:

$$h2 m2 + j2 m2 + k2^2 = 0$$

Variables to be uneliminated:

$$"k2 := 'k2"$$

$$"h2 := 'h2"$$

$$"h6 := 'h6"$$

Proceed on case level 1 with:

$$m2 \neq 0$$

On account of:

$$h2 m2 + j2 m2 + k2^2 = 0$$

the following return value can be used as an equation:

$$eq1 := h2 m2 + j2 m2 + k2^2$$

> **elimsolve** (eq1,j2);

$$\{m2 \neq 0\}$$

j2 is set to:

$$-\frac{h^2 m^2 + k^2}{m^2}$$

> #det (T - jacobian(H,[x1,x2,x3,x4,x5,x6])) mod 2;

> expand(diff(H[2],x2,x3)) mod 2;

$$\frac{h^2}{m^2} + \frac{k^2}{m^2} + \frac{k^2 m^5}{m^2}$$

> expand(diff(H[1],x2,x3) \* H[2] - diff(H[2],x2,x3) \* H[1]) mod 2;

$$0$$

> contradict (1);

Contradiction on case level 1, so:

$$m^2 = 0$$

Variables to be uneliminated:

"j2 := 'j2'"

"j6 := 'j6'"

"f2 := 'f2'"

"k6 := 'k6'"

"g6 := 'g6'"

"g2 := 'g2'"

"j5 := 'j5'"

"g5 := 'g5'"

"k5 := 'k5'"

"m4 := 'm4'"

"k4 := 'k4'"

"h4 := 'h4'"

"h3 := 'h3'"

"j4 := 'j4'"

"f3 := 'f3'"

"f4 := 'f4'"

"h5 := 'h5'"

"f5 := 'f5'"

"f6 := 'f6'"

"m3 := 'm3'"

"k3 := 'k3'"

"j3 := 'j3'"

"g3 := 'g3'"

"g4 := 'g4'"

Proceed on case level 0 with:

$$1 \neq 0$$

On account of:

$$m^2 = 0$$

|                                                       |                                       |
|-------------------------------------------------------|---------------------------------------|
|                                                       | $\{1 \neq 0\}$                        |
| m2 is set to:                                         |                                       |
|                                                       | 0                                     |
| > tmp1 := cpCoeff (x6^2*T^4);                         |                                       |
|                                                       | $tmp1 := k2\ m3 + k2^2 + m3^2$        |
| > tmp2 := cpCoeff (x6^3*T^3);                         |                                       |
|                                                       | $tmp2 := k2\ m3\ (k2 + m3)$           |
| > tmp3 := expand(k2 * tmp1 - tmp2);                   |                                       |
|                                                       | $tmp3 := k2^3$                        |
| > tmp4 := expand(m3 * tmp1 - tmp2);                   |                                       |
|                                                       | $tmp4 := m3^3$                        |
| > elimsolve (tmp3,k2);                                |                                       |
|                                                       | $\{1 \neq 0\}$                        |
| k2 is set to:                                         |                                       |
|                                                       | 0                                     |
| > elimsolve (tmp4,m3);                                |                                       |
|                                                       | $\{1 \neq 0\}$                        |
| m3 is set to:                                         |                                       |
|                                                       | 0                                     |
| > tmp1 := cpCoeff (x1^2*x4^2*T^2);                    |                                       |
|                                                       | $tmp1 := j2^2$                        |
| > elimsolve (tmp1,j2);                                |                                       |
|                                                       | $\{1 \neq 0\}$                        |
| j2 is set to:                                         |                                       |
|                                                       | 0                                     |
| > tmp1 := cpCoeff (x1^2*x3*x5*T^2);                   |                                       |
|                                                       | $tmp1 := k3^2 + h2\ m4 + m4^2 + h2^2$ |
| > tmp2 := cpCoeff (x1*x4*x5*T^3);                     |                                       |
|                                                       | $tmp2 := m4^2 + h2\ k3 + h2^2 + k3^2$ |
| > tmp3 := Factor (tmp1*(h2+k3) - (h2+m4)*tmp2) mod 2; |                                       |
|                                                       | $tmp3 := (m4 + k3)^3$                 |
| > elimsolve (tmp3,k3);                                |                                       |
|                                                       | $\{1 \neq 0\}$                        |
| k3 is set to:                                         |                                       |
|                                                       | -m4                                   |
| > tmp1 := cpCoeff (x5^4*T^2);                         |                                       |
|                                                       | $tmp1 := m4^4$                        |
| > elimsolve (tmp1,m4);                                |                                       |
|                                                       | $\{1 \neq 0\}$                        |
| m4 is set to:                                         |                                       |
|                                                       | 0                                     |
| > tmp1 := cpCoeff (x5^3*T^3);                         |                                       |
|                                                       | $tmp1 := h2^3$                        |

> **elimsolve** (tmp1,h2);

$$\{1 \neq 0\}$$

h2 is set to:

$$0$$

> **launchNZcase** (j3);

Launching case level 1:

$$j3 \neq 0$$

Assume from now on that:

$$j3 \neq 0$$

> **launchNZcase** (g2);

Launching case level 2:

$$g2 \neq 0$$

Assume from now on that:

$$g2 j3 \neq 0$$

> **tmp1** := **cpCoeff** (x1\*x3\*x4\*T^3);

$$tmp1 := g2 (k4 + j3)$$

> **elimsolve** (tmp1,k4);

$$\{1 \neq 0\}$$

k4 is set to:

$$-j3$$

> **launchNZcase** (g2 + m5);

Launching case level 3:

$$g2 + m5 \neq 0$$

Assume from now on that:

$$j3 g2 (g2 + m5) \neq 0$$

> **tmp1** := **cpCoeff** (x1\*x3\*x4^2\*T^2);

$$tmp1 := (g2^2 + g2 j3 + g2 m5 + m5^2) (g2 + m5)$$

> **elimsolve** (tmp1,j3);

$$\{g2 \neq 0\}$$

j3 is set to:

$$-\frac{g2^2 + g2 m5 + m5^2}{g2}$$

Nonzero constraint refines to:

$$(-g2^2 - g2 m5 - m5^2) g2 (g2 + m5) \neq 0$$

> **tmp1** := **cpCoeff** (x4^4\*T^2);

$$tmp1 := \frac{(g2^2 + g2 m5 + m5^2)^4}{g2^4}$$

> **eq1** := **contradict** (tmp1);

Contradiction on case level 3, so:

$$g2 + m5 = 0$$

Variables to be uneliminated:

$$"j3 := j3"$$

Proceed on case level 2 with:

$$g2 j3 \neq 0$$

On account of:



```

g2 + m5 = 0
the following return value can be used as an equation:
eq1 := g2 + m5

> elimsolve (eq1,m5);

{1 ≠ 0}

m5 is set to:

-g2

> tmp1 := cpCoeff (x4^4*T^2);

tmp1 := j3^4

> contradict (tmp1);
Contradiction on case level 2, so:

g2 = 0

Variables to be uneliminated:

"m5 := 'm5'"
"k4 := 'k4'"

Proceed on case level 1 with:

j3 ≠ 0

On account of:

g2 = 0
{1 ≠ 0}

g2 is set to:

0

> tmp1 := cpCoeff (x1*x3*x4^2*T^2);

tmp1 := m5^3

> elimsolve (tmp1,m5);

{1 ≠ 0}

m5 is set to:

0

> tmp1 := cpCoeff (x4^4*T^2);

tmp1 := j3^4

> contradict (tmp1);
Contradiction on case level 1, so:

j3 = 0

Variables to be uneliminated:

"m5 := 'm5'"
"g2 := 'g2'"

Proceed on case level 0 with:

1 ≠ 0

On account of:

j3 = 0
{1 ≠ 0}

j3 is set to:

0

> tmp1 := cpCoeff (x4^3*T^3);

tmp1 := m5^3

```

```

> elimsolve (tmp1,m5);
m5 is set to:  $\{1 \neq 0\}$ 
0
> tmp1 := cpCoeff (x4^4*T^2);
tmp1 :=  $g2^4$ 
> elimsolve (tmp1,g2);
g2 is set to:  $\{1 \neq 0\}$ 
0
> launchNZcase (k4);
Launching case level 1:
Assume from now on that:
k4  $\neq 0$ 
k4  $\neq 0$ 
> tmp1 := cpCoeff (x2*x6*T^4);
tmp1 :=  $k4\ h3$ 
> elimsolve (tmp1,h3);
h3 is set to:  $\{1 \neq 0\}$ 
0
> tmp1 := cpCoeff (x1*x2*x4*T^3);
tmp1 :=  $k4\ (m6 + g3)$ 
> elimsolve (tmp1,g3);
g3 is set to:  $\{1 \neq 0\}$ 
 $-m6$ 
> tmp1 := cpCoeff (x1*x3^2*T^3);
tmp1 :=  $k4\ (m6 + f2 + k5)$ 
> elimsolve (tmp1,k5);
k5 is set to:  $\{1 \neq 0\}$ 
 $-m6 - f2$ 
> tmp1 := cpCoeff (x1*x2*x3*T^3);
tmp1 :=  $m6\ j4 + k4\ h5 + f3\ k4 + f2\ j4 + m6\ f2 + m6^2$ 
> elimsolve (tmp1,f3);
f3 is set to:  $\{k4 \neq 0\}$ 

$$-\frac{m6\ j4 + k4\ h5 + f2\ j4 + m6\ f2 + m6^2}{k4}$$

> tmp1 := cpCoeff (x2^2*x6*T^3);
tmp1 :=  $(m6\ f2 + f2^2 + k6\ k4 + k4\ j5 + j4^2)\ k4$ 
> elimsolve (tmp1,j5);
k4  $\neq 0$ 

```

j5 is set to:

$$-\frac{m6 f2 + f2^2 + k6 k4 + j4^2}{k4}$$

> tmp1 := cpCoeff (x3^3\*T^3);

$$tmp1 := k4^2 j6 + f2^3 + j4^3 + m6^2 f2 + f2^2 j4 + f2 j4^2 + m6 j4 f2$$

> elimsolve (tmp1,j6);

$$\{k4^2 \neq 0\}$$

j6 is set to:

$$-\frac{f2^3 + j4^3 + m6^2 f2 + f2^2 j4 + f2 j4^2 + m6 j4 f2}{k4^2}$$

> tmp1 := cpCoeff (x1^2\*x2^2\*T^2);

$$tmp1 := (m6 + f2)^2$$

> elimsolve (tmp1,m6);

$$\{1 \neq 0\}$$

m6 is set to:

$$-f2$$

> tmp1 := cpCoeff (x3^4\*T^2);

$$tmp1 := f2^4$$

> elimsolve (tmp1,f2);

$$\{1 \neq 0\}$$

f2 is set to:

$$0$$

> tmp1 := cpCoeff (x2\*x3\*x4\*T^3);

$$tmp1 := h4 j4^2 + k4^2 g5 + h6 k4^2$$

> elimsolve (tmp1,g5);

$$\{k4^2 \neq 0\}$$

g5 is set to:

$$-\frac{h4 j4^2 + h6 k4^2}{k4^2}$$

> tmp1 := cpCoeff (x2\*x3^2\*T^3);

$$tmp1 := k4^2 g6 + j4^2 g4 + h5 j4^2$$

> elimsolve (tmp1,g6);

$$\{k4^2 \neq 0\}$$

g6 is set to:

$$-\frac{j4^2 (g4 + h5)}{k4^2}$$

> tmp1 := cpCoeff (x2^4\*T^2);

$$tmp1 := \frac{(g4 k4 + h4 j4)^4}{k4^4}$$

> elimsolve (tmp1,g4);

$$\{k4 \neq 0\}$$

g4 is set to:

$$-\frac{h_4 j_4}{k_4}$$

**> tmp1 := cpCoeff(x2^3\*T^3);**

$$tmp1 := h_5^3$$

**> elimsolve (tmp1,h5);**

$$\{1 \neq 0\}$$

h5 is set to:

$$0$$

**> det (T - jacobian(H,[x1,x2,x3,x4,x5,x6])) mod 2;**

$$T^6$$

**> H[2];**

$$0$$

**> contradict (1);**

Contradiction on case level 1, so:

$$k_4 = 0$$

Variables to be uneliminated:

"h5 := 'h5'"

"g4 := 'g4'"

"g6 := 'g6'"

"g5 := 'g5'"

"f2 := 'f2'"

"m6 := 'm6'"

"j6 := 'j6'"

"j5 := 'j5'"

"f3 := 'f3'"

"k5 := 'k5'"

"g3 := 'g3'"

"h3 := 'h3'"

Proceed on case level 0 with:

$$1 \neq 0$$

On account of:

$$k_4 = 0$$

$$\{1 \neq 0\}$$

k4 is set to:

$$0$$

**> launchNZcase (h3);**

Launching case level 1:

$$h_3 \neq 0$$

Assume from now on that:

$$h_3 \neq 0$$

**> tmp1 := cpCoeff (x1^2\*x2\*x3\*T^2);**

$$tmp1 := h_3 (m_6 + j_4)$$

```

> elimsolve (tmp1,j4);
                                     {1 ≠ 0}
j4 is set to:
                                     -m6
> tmp1 := cpCoeff (x1*x2^2*x6*T^2);
                                     tmp1 := h3^2 (m6 + k5)
> elimsolve (tmp1,k5);
                                     {1 ≠ 0}
k5 is set to:
                                     -m6
> tmp1 := cpCoeff (x2^2*x5^2*T^2);
                                     tmp1 := h3^2 (f2 + m6)^2
> elimsolve (tmp1,f2);
                                     {1 ≠ 0}
f2 is set to:
                                     -m6
> tmp1 := cpCoeff (x3^4*T^2);
                                     tmp1 := m6^4
> elimsolve (tmp1,m6);
                                     {1 ≠ 0}
m6 is set to:
                                     0
> tmp1 := cpCoeff (x1*x2^2*x4*T^2);
                                     tmp1 := j6 h3^2
> elimsolve (tmp1,j6);
                                     {1 ≠ 0}
j6 is set to:
                                     0
> tmp1 := cpCoeff (x1*x2^2*x5*T^2);
                                     tmp1 := (k6 + j5) h3^2
> elimsolve (tmp1,j5);
                                     {1 ≠ 0}
j5 is set to:
                                     -k6
> tmp1 := cpCoeff (x1*x2^2*T^3);
                                     tmp1 := h4 f3 + h5 h4 + g3 k6 + h3 h6 + h3 f4
> elimsolve (tmp1,f4);
                                     {h3 ≠ 0}
f4 is set to:
                                     -  $\frac{h4 f3 + h5 h4 + g3 k6 + h3 h6}{h3}$ 
> tmp1 := cpCoeff (x1^2*x2^2*T^2);
                                     tmp1 := g3^2 + g3 h4 + h3 g4 + h3 h5 + h3 k6

```

> **elimsolve** (tmp1,g4);

$$\{h3 \neq 0\}$$

g4 is set to:

$$-\frac{g3^2 + g3 h4 + h3 h5 + h3 k6}{h3}$$

> **tmp1 := cpCoeff**(x1\*x2^3\*T^2);

$$tmp1 := (g3^2 h3 h4 f3 + g3 k6 h5 h3^2 + g3^2 h3 k6 h4 + g3^2 h3 h5 h4 + g3^3 h4^2 + f6 h3^4 + g3^2 h3^2 h6 + h4 g6 h3^3 + g3^5 + g5 h3^2 g3^2 + h5^2 h3^2 g3 + f3^2 h3^2 g3) / h3^2$$

> **elimsolve** (tmp1,f6);

$$\{h3^4 \neq 0\}$$

f6 is set to:

$$-(g3^2 h3 h4 f3 + g3 k6 h5 h3^2 + g3^2 h3 k6 h4 + g3^2 h3 h5 h4 + g3^3 h4^2 + g3^2 h3^2 h6 + h4 g6 h3^3 + g3^5 + g5 h3^2 g3^2 + h5^2 h3^2 g3 + f3^2 h3^2 g3) / h3^4$$

> **tmp1 := cpCoeff**(x2^2\*x4\*T^3);

$$tmp1 := (g6 h3^3 + h5^2 h3^2 + g3^2 h4^2 + f5 h3^3 + f3^2 h3^2 + h6 h4 h3^2 + h4 g5 h3^2 + g3^2 h3 k6 + h3^2 h5 k6 + h3 h5 g3^2 + f3 h3 g3^2 + g3^4) / h3$$

> **elimsolve** (tmp1,f5);

$$\{h3^3 \neq 0\}$$

f5 is set to:

$$-(g6 h3^3 + h5^2 h3^2 + g3^2 h4^2 + f3^2 h3^2 + h6 h4 h3^2 + h4 g5 h3^2 + g3^2 h3 k6 + h3^2 h5 k6 + h3 h5 g3^2 + f3 h3 g3^2 + g3^4) / h3^3$$

> **launchNZcase** (k6);

Launching case level 2:

$$k6 \neq 0$$

Assume from now on that:

$$h3 k6 \neq 0$$

> **launchNZcase**

$$(f3^2 h3 + f3 g3^2 + f3 h3 h5 + g3^2 h5 + g3^2 k6 + g3 g5 h3 + g3 h3 h6 + g6 h3^2 + h3 h5^2) ;$$

Launching case level 3:

$$f3^2 h3 + f3 g3^2 + f3 h3 h5 + h5 g3^2 + g3^2 k6 + g3 g5 h3 + h3 h6 g3 + g6 h3^2 + h3 h5^2 \neq 0$$

Assume from now on that:

$$h3 k6 (f3^2 h3 + f3 g3^2 + f3 h3 h5 + h5 g3^2 + g3^2 k6 + g3 g5 h3 + h3 h6 g3 + g6 h3^2 + h3 h5^2) \neq 0$$

> **tmp1 := cpCoeff** (x2^5\*T);

$$tmp1 := (g6 h3^2 + k6 h3 h5 + h3 k6^2 + f3 h3 h5 + h3 k6 f3 + g3 h3 h6 + g3 g5 h3 + g3^2 k6 + g3^2 h5 + f3 g3^2) k6 (f3^2 h3 + f3 g3^2 + f3 h3 h5 + g3^2 h5 + g3^2 k6 + g3 g5 h3 + g3 h3 h6 + g6 h3^2 + h3 h5^2) / h3^2$$

> **elimsolve** (tmp1,g6);

$$\{h3^2 \neq 0\}$$

g6 is set to:

$$-\frac{k6\ h3\ h5 + h3\ k6^2 + f3\ h3\ h5 + h3\ k6\ f3 + g3\ h3\ h6 + g3\ g5\ h3 + g3^2\ k6 + g3^2\ h5 + f3\ g3^2}{h3^2}$$

Nonzero constraint refines to:

$$h3^2\ k6\ (f3^2 - h5\ k6 - k6^2 - f3\ k6 + h5^2) \neq 0$$

> **tmp1 := cpCoeff (x2^3\*T^3);**

$$tmp1 := (k6 + h5 + f3)^3$$

> **elimsolve (tmp1, f3);**

$$\{1 \neq 0\}$$

f3 is set to:

$$-k6 - h5$$

Nonzero constraint refines to:

$$h3^2\ k6\ (k6^2 + 2\ h5\ k6 + 2\ h5^2) \neq 0$$

> **tmp1 := cpCoeff (x2^4\*T^2);**

$$tmp1 := k6^4$$

> **eq1 := contradict (tmp1);**

Contradiction on case level 3, so:

$$f3^2\ h3 + f3\ g3^2 + f3\ h3\ h5 + g3^2\ h5 + g3^2\ k6 + g3\ g5\ h3 + g3\ h3\ h6 + g6\ h3^2 + h3\ h5^2 = 0$$

Variables to be uneliminated:

$$"f3 := 'f3"$$

$$"g6 := 'g6"$$

Proceed on case level 2 with:

$$h3\ k6 \neq 0$$

On account of:

$$f3^2\ h3 + f3\ g3^2 + f3\ h3\ h5 + g3^2\ h5 + g3^2\ k6 + g3\ g5\ h3 + g3\ h3\ h6 + g6\ h3^2 + h3\ h5^2 = 0$$

the following return value can be used as an equation:

$$eq1 := f3^2\ h3 + f3\ g3^2 + f3\ h3\ h5 + g3^2\ h5 + g3^2\ k6 + g3\ g5\ h3 + g3\ h3\ h6 + g6\ h3^2 + h3\ h5^2$$

> **elimsolve (eq1, g6);**

$$\{h3^2 \neq 0\}$$

g6 is set to:

$$-\frac{f3^2\ h3 + f3\ g3^2 + f3\ h3\ h5 + g3^2\ h5 + g3^2\ k6 + g3\ g5\ h3 + g3\ h3\ h6 + h3\ h5^2}{h3^2}$$

> **tmp1 := cpCoeff (x2^3\*T^3);**

$$tmp1 := (h5 + f3)^3$$

> **elimsolve (tmp1, f3);**

$$\{1 \neq 0\}$$

f3 is set to:

$$-h5$$

> **tmp1 := cpCoeff (x2^4\*T^2);**

$$tmp1 := k6^4$$

> **contradict (tmp1);**

Contradiction on case level 2, so:

$$k6 = 0$$

Variables to be uneliminated:

|                                                  |                                            |
|--------------------------------------------------|--------------------------------------------|
|                                                  | "f3 := 'f3'"                               |
|                                                  | "g6 := 'g6'"                               |
| Proceed on case level 1 with:                    |                                            |
|                                                  | $h3 \neq 0$                                |
| On account of:                                   |                                            |
|                                                  | $k6 = 0$                                   |
|                                                  | $\{1 \neq 0\}$                             |
| k6 is set to:                                    |                                            |
|                                                  | 0                                          |
| > tmp1 := cpCoeff (x2^3*T^3);                    |                                            |
|                                                  | $tmp1 := (h5 + f3)^3$                      |
| > elimsolve (tmp1,f3);                           |                                            |
|                                                  | $\{1 \neq 0\}$                             |
| f3 is set to:                                    |                                            |
|                                                  | $-h5$                                      |
| > tmp1 := cpCoeff (x2^4*T^2);                    |                                            |
|                                                  | $tmp1 := (g6 h3 + h6 g3 + g5 g3 + h5^2)^2$ |
| > elimsolve (tmp1,g6);                           |                                            |
|                                                  | $\{h3 \neq 0\}$                            |
| g6 is set to:                                    |                                            |
|                                                  | $-\frac{h6 g3 + g5 g3 + h5^2}{h3}$         |
| > det (T-jacobian(H,[x1,x2,x3,x4,x5,x6])) mod 2; |                                            |
|                                                  | $T^6$                                      |
| > H[2];                                          |                                            |
|                                                  | 0                                          |
| > contradict (1);                                |                                            |
| Contradiction on case level 1, so:               |                                            |
|                                                  | $h3 = 0$                                   |
| Variables to be uneliminated:                    |                                            |
|                                                  | "g6 := 'g6'"                               |
|                                                  | "f3 := 'f3'"                               |
|                                                  | "k6 := 'k6'"                               |
|                                                  | "f5 := 'f5'"                               |
|                                                  | "f6 := 'f6'"                               |
|                                                  | "g4 := 'g4'"                               |
|                                                  | "f4 := 'f4'"                               |
|                                                  | "j5 := 'j5'"                               |
|                                                  | "j6 := 'j6'"                               |
|                                                  | "m6 := 'm6'"                               |
|                                                  | "f2 := 'f2'"                               |
|                                                  | "k5 := 'k5'"                               |



|                                                       |                                                                             |
|-------------------------------------------------------|-----------------------------------------------------------------------------|
|                                                       | <code>"j4 := 'j4'"</code>                                                   |
| Proceed on case level 0 with:                         |                                                                             |
|                                                       | $1 \neq 0$                                                                  |
| On account of:                                        |                                                                             |
|                                                       | $h3 = 0$                                                                    |
|                                                       | $\{1 \neq 0\}$                                                              |
| h3 is set to:                                         |                                                                             |
|                                                       | 0                                                                           |
| <b>&gt; launchNZcase (f2);</b>                        |                                                                             |
| Launching case level 1:                               |                                                                             |
|                                                       | $f2 \neq 0$                                                                 |
| Assume from now on that:                              |                                                                             |
|                                                       | $f2 \neq 0$                                                                 |
| <b>&gt; launchNZcase (k5);</b>                        |                                                                             |
| Launching case level 2:                               |                                                                             |
|                                                       | $k5 \neq 0$                                                                 |
| Assume from now on that:                              |                                                                             |
|                                                       | $f2 k5 \neq 0$                                                              |
| <b>&gt; tmp1 := cpcoeff(x3^3*T^3);</b>                |                                                                             |
|                                                       | $tmp1 := -f2 j4 k5 - f2^2 k5 - f2 k5^2 + j4^3$                              |
| <b>&gt; tmp2 := cpcoeff(x3^5*T);</b>                  |                                                                             |
|                                                       | $tmp2 := f2 (f2 k5 + f2 j4 + f2^2 + k5 j4 + k5^2 + j4^2) k5 (f2 + j4 + k5)$ |
| <b>&gt; tmp3 := Factor (tmp2 - f2*k5*tmp1) mod 2;</b> |                                                                             |
|                                                       | $tmp3 := f2 k5 (k5 + f2)^3$                                                 |
| <b>&gt; elimsolve (tmp3,k5);</b>                      |                                                                             |
|                                                       | $\{1 \neq 0\}$                                                              |
| k5 is set to:                                         |                                                                             |
|                                                       | $-f2$                                                                       |
| Nonzero constraint refines to:                        |                                                                             |
|                                                       | $-f2^2 \neq 0$                                                              |
| <b>&gt; tmp1 := cpCoeff(x3^4*T^2);</b>                |                                                                             |
|                                                       | $tmp1 := f2^4$                                                              |
| <b>&gt; contradict (tmp1);</b>                        |                                                                             |
| Contradiction on case level 2, so:                    |                                                                             |
|                                                       | $k5 = 0$                                                                    |
| Variables to be uneliminated:                         |                                                                             |
|                                                       | <code>"k5 := 'k5'"</code>                                                   |
| Proceed on case level 1 with:                         |                                                                             |
|                                                       | $f2 \neq 0$                                                                 |
| On account of:                                        |                                                                             |
|                                                       | $k5 = 0$                                                                    |
|                                                       | $\{1 \neq 0\}$                                                              |
| k5 is set to:                                         |                                                                             |
|                                                       | 0                                                                           |
| <b>&gt; tmp1 := cpCoeff(x3^3*T^3);</b>                |                                                                             |

```

[                                      $tmp1 := j4^3$ 
> elimsolve (tmp1,j4);
                                      $\{1 \neq 0\}$ 
j4 is set to:
                                     0
[ > tmp1 := cpCoeff(x3^4*T^2);
                                      $tmp1 := f2^4$ 
> contradict (tmp1);
Contradiction on case level 1, so:
                                      $f2 = 0$ 
Variables to be uneliminated:
                                     "j4 := 'j4'"
                                     "k5 := 'k5'"
Proceed on case level 0 with:
                                      $1 \neq 0$ 
On account of:
                                      $f2 = 0$ 
                                      $\{1 \neq 0\}$ 
f2 is set to:
                                     0
[ > tmp1 := cpCoeff(x3^3*T^3);
                                      $tmp1 := j4^3$ 
> elimsolve (tmp1,j4);
                                      $\{1 \neq 0\}$ 
j4 is set to:
                                     0
[ > tmp1 := cpCoeff(x3^4*T^2);
                                      $tmp1 := k5^4$ 
> elimsolve (tmp1,k5);
                                      $\{1 \neq 0\}$ 
k5 is set to:
                                     0
[ > launchNZcase (m6);
Launching case level 1:
                                      $m6 \neq 0$ 
Assume from now on that:
                                      $m6 \neq 0$ 
[ > tmp1 := cpCoeff (x1*x2*x3*T^3);
                                      $tmp1 := m6 (g3 + h4)$ 
> elimsolve (tmp1,g3);
                                      $\{1 \neq 0\}$ 
g3 is set to:
                                      $-h4$ 
[ > launchNZcase (h4);
Launching case level 2:

```



```

0
> contradict (1);
Contradiction on case level 2, so:

$$h4 = 0$$

Variables to be uneliminated:

$$\begin{aligned} "g4 &:= 'g4'" \\ "j5 &:= 'j5'" \\ "f5 &:= 'f5'" \\ "f4 &:= 'f4'" \\ "f3 &:= 'f3'" \end{aligned}$$

Proceed on case level 1 with:

$$m6 \neq 0$$

On account of:

$$\begin{aligned} h4 &= 0 \\ \{1 &\neq 0\} \end{aligned}$$

h4 is set to:
0
> launchNZcase (g4);
Launching case level 2:

$$g4 \neq 0$$

Assume from now on that:

$$m6 \, g4 \neq 0$$

> launchNZcase (h5);
Launching case level 3:

$$h5 \neq 0$$

Assume from now on that:

$$m6 \, g4 \, h5 \neq 0$$

> tmp1 := cpcoeff (x2^3*T^3);

$$tmp1 := -f3 \, g4 \, h5 + f3^3 - h5 \, g4^2 - h5^2 \, g4$$

> tmp2 := cpcoeff (x2^5*T);

$$tmp2 := (h5 \, f3 + f3 \, g4 + f3^2 + h5 \, g4 + h5^2 + g4^2) \, g4 \, h5 \, (f3 + g4 + h5)$$

> tmp3 := Factor (tmp2 - g4*h5*tmp1) mod 2;

$$tmp3 := h5 \, (h5 + g4)^3 \, g4$$

> elimsolve (tmp3,h5);

$$\{1 \neq 0\}$$

h5 is set to:

$$-g4$$

Nonzero constraint refines to:

$$-m6 \, g4^2 \neq 0$$

> tmp1 := cpCoeff (x2^4*T^2);

$$tmp1 := g4^4$$

> contradict (tmp1);
Contradiction on case level 3, so:

$$h5 = 0$$

Variables to be uneliminated:

```

```

" h5 := 'h5'"

Proceed on case level 2 with:

On account of:

h5 is set to:

0

> tmp1 := cpCoeff (x2^3*T^3);
tmp1 := f3^3

> elimsolve (tmp1,f3);
{ 1 ≠ 0 }

f3 is set to:

0

> tmp1 := cpCoeff (x2^4*T^2);
tmp1 := g4^4

> contradict (tmp1);
Contradiction on case level 2, so:

Variables to be uneliminated:

" f3 := 'f3'"
" h5 := 'h5'"

Proceed on case level 1 with:

On account of:

g4 is set to:

0

> tmp1 := cpCoeff (x2^3*T^3);
tmp1 := f3^3

> elimsolve (tmp1,f3);
{ 1 ≠ 0 }

f3 is set to:

0

> tmp1 := cpCoeff (x2^4*T^2);
tmp1 := h5^4

> elimsolve (tmp1,h5);
{ 1 ≠ 0 }

h5 is set to:

0

> det (T - jacobian(H,[x1,x2,x3,x4,x5,x6])) mod 2;
T^6

> H[2];

```

```

0
> contradict (1);
Contradiction on case level 1, so:

$$m6 = 0$$

Variables to be uneliminated:

$$\begin{aligned} &"h5 := 'h5'" \\ &"f3 := 'f3'" \\ &"g4 := 'g4'" \\ &"h4 := 'h4'" \\ &"g3 := 'g3'" \end{aligned}$$

Proceed on case level 0 with:

$$1 \neq 0$$

On account of:

$$\begin{aligned} &m6 = 0 \\ &\{1 \neq 0\} \end{aligned}$$

m6 is set to:

$$0$$

> launchNZcase (g3);
Launching case level 1:

$$g3 \neq 0$$

Assume from now on that:

$$g3 \neq 0$$

> tmp1 := cpCoeff (x1^2*x2^2*T^2);

$$tmp1 := -g3 (g3 + h4)$$

> elimsolve (tmp1,g3);

$$\{1 \neq 0\}$$

g3 is set to:

$$-h4$$

Nonzero constraint refines to:

$$-h4 \neq 0$$

> tmp1 := cpCoeff (x1*x2^2*T^3);

$$tmp1 := -h4 (h5 + j5 - f3)$$

> elimsolve (tmp1,f3);

$$\{-1 \neq 0\}$$

f3 is set to:

$$h5 + j5$$

> tmp1 := cpCoeff (x2^2*x3*T^3);

$$tmp1 := h4 (f4 h4 + h4 g5 + h5^2 + g4^2 + g4 j5 + j5^2)$$

> elimsolve (tmp1,f4);

$$\{h4 \neq 0\}$$

f4 is set to:

$$-\frac{h4 g5 + h5^2 + g4^2 + g4 j5 + j5^2}{h4}$$

> tmp1 := cpCoeff (x2^3*T^3);

```

```

[      tmp1 := h5^3 + h5 g4^2 + h5 j5 g4 + f5 h4^2 + h5^2 g4 + h5 j5^2 + g4^3
> elimsolve (tmp1,f5);
                                     {h4^2 ≠ 0}
f5 is set to:
      -  $\frac{h5^3 + h5 g4^2 + h5 j5 g4 + h5^2 g4 + h5 j5^2 + g4^3}{h4^2}$ 
[> tmp1 := cpCoeff (x2^4*T^2);
                                     tmp1 := g4^4 + j5^4 + g4^3 j5
[> tmp2 := cpCoeff (x2^5*T);
                                     tmp2 := (j5 + g4) j5 g4^3
[> tmp3 := expand(tmp2 - j5*tmp1);
                                     tmp3 := -j5^5
[> elimsolve (tmp3,j5);
                                     {1 ≠ 0}
j5 is set to:
                                     0
[> tmp1 := cpCoeff (x2^4*T^2);
                                     tmp1 := g4^4
[> elimsolve (tmp1,g4);
                                     {1 ≠ 0}
g4 is set to:
                                     0
[> det (T - jacobian(H,[x1,x2,x3,x4,x5,x6])) mod 2;
                                     T^6
[> H[2];
                                     0
[> contradict (1);
Contradiction on case level 1, so:
                                     g3 = 0
Variables to be uneliminated:
                                     "g4 := 'g4'"
                                     "j5 := 'j5'"
                                     "f5 := 'f5'"
                                     "f4 := 'f4'"
                                     "f3 := 'f3'"
                                     "g3 := 'g3'"
Proceed on case level 0 with:
                                     1 ≠ 0
On account of:
                                     g3 = 0
                                     {1 ≠ 0}
g3 is set to:
                                     0

```

```

> launchNZcase (h4);
Launching case level 1:



#### ≠ 0 Assume from now on that: ≠ 0 > tmp1 := cpCoeff (x2^2*x4*T^3); tmp1 := -h4^2 (j5 + k6) > elimsolve (tmp1,j5); {1 ≠ 0} j5 is set to: -k6 > tmp1 := cpCoeff (x1*x2^2*T^3); tmp1 := -h4 (f3 + 2 g4 + h5) > elimsolve (tmp1,f3); {1 ≠ 0} f3 is set to: -2 g4 - h5 > tmp1 := cpCoeff (x2^2*x3*T^3); tmp1 := j6 h4^2 > elimsolve (tmp1,j6); {1 ≠ 0} j6 is set to: 0 > tmp1 := cpCoeff (x2^3*T^3); tmp1 := h5 g4^2 + h5^3 + h6 h4 g4 + g6 h4^2 + h4 g5 g4 > elimsolve (tmp1,g6); {h4^2 ≠ 0} g6 is set to: - $\frac{h5 g4^2 + h5^3 + h6 h4 g4 + h4 g5 g4}{h4^2}$ > launchNZcase (h5); Launching case level 2: ≠ 0 Assume from now on that: h5 ≠ 0 > tmp1 := cpCoeff (x2^5*T); tmp1 := h5^3 (g4^2 + h6 h4 + h4 g5 + h5^2) > elimsolve (tmp1,g5); {h4 ≠ 0} g5 is set to: - $\frac{g4^2 + h6 h4 + h5^2}{h4}$ > tmp1 := cpCoeff (x2^4*T^2);


```



$$tmp1 := h5^4$$

```
> contradict (tmp1);
```

Contradiction on case level 2, so:

$$h5 = 0$$

Variables to be uneliminated:

```
"g5" := "g5"
```

Proceed on case level 1 with:

$$h4 \neq 0$$

On account of:

$$h5 = 0$$

$$\{1 \neq 0\}$$

## h5 is set to:

0

```
> tmp1 := cpCoeff (x2^4*T^2) ;
```

$$tmp1 := (g4^2 + h4\,g5 + h6\,h4)^2$$

```
> elimsolve (tmp1,g5);
```

$\{h4 \neq 0\}$

g5 is set to:

$$-\frac{g^4 + h^6}{h^4}$$

```
> det (T - jacobian(H,[x1,x2,x3,x4,x5,x6])) mod 2;
```

$$T^6$$

```
> H[2];
```

0

```
> contradict (1);
```

Contradiction on case level 1, so:

$$h4 = 0$$

Variables to be uneliminated:

```
"g5 := 'g5'"
```

### "h5 := 'h5'"

```
"g6 := 'g6'"
```

```
"j6" := "j6"
```

```
"f3 := 'f3'"
```

```
"j5" := "j5"
```

Proceed on case level 0 with:

$$1 \neq 0$$

On account of:

$$h_4 = 0$$

$\{1 \neq 0\}$

#### h4 is set to:

0

```
> launchNZcase (g4) ;
```

Launching case level 1:

$$g_4 \neq 0$$

Assume from now on that:

$$g4 \neq 0$$

> **launchNZcase** (h5);

Launching case level 2:

$$h5 \neq 0$$

Assume from now on that:

$$h5 \, g4 \neq 0$$

> **tmp1** := **cpcoeff** (x2^3\*T^3);

$$tmp1 := -h5^2 \, g4 - h5 \, g4^2 - f3 \, g4 \, h5 + f3^3$$

> **tmp2** := **cpcoeff** (x2^5\*T);

$$tmp2 := (h5 \, f3 + f3 \, g4 + f3^2 + h5 \, g4 + h5^2 + g4^2) \, g4 \, h5 \, (f3 + g4 + h5)$$

> **tmp3** := **Factor** (tmp2 - g4\*h5\*tmp1) mod 2;

$$tmp3 := (h5 + g4)^3 \, h5 \, g4$$

> **elimsolve** (tmp3,h5);

$$\{1 \neq 0\}$$

h5 is set to:

$$-g4$$

Nonzero constraint refines to:

$$-g4^2 \neq 0$$

> **tmp1** := **cpCoeff** (x2^4\*T^2);

$$tmp1 := g4^4$$

> **contradict** (tmp1);

Contradiction on case level 2, so:

$$h5 = 0$$

Variables to be uneliminated:

$$"h5 := 'h5'"$$

Proceed on case level 1 with:

$$g4 \neq 0$$

On account of:

$$h5 = 0$$

$$\{1 \neq 0\}$$

h5 is set to:

$$0$$

> **tmp1** := **cpCoeff** (x2^3\*T^3);

$$tmp1 := f3^3$$

> **elimsolve** (tmp1,f3);

$$\{1 \neq 0\}$$

f3 is set to:

$$0$$

> **tmp1** := **cpCoeff** (x2^4\*T^2);

$$tmp1 := g4^4$$

> **contradict** (tmp1);

Contradiction on case level 1, so:

$$g4 = 0$$

Variables to be uneliminated:

|                                                    |                |
|----------------------------------------------------|----------------|
|                                                    | "f3 := 'f3'"   |
|                                                    | "h5 := 'h5'"   |
| Proceed on case level 0 with:                      |                |
|                                                    | $1 \neq 0$     |
| On account of:                                     |                |
|                                                    | $g4 = 0$       |
|                                                    | $\{1 \neq 0\}$ |
| g4 is set to:                                      |                |
|                                                    | 0              |
| > tmp1 := cpCoeff (x2^3*T^3);                      |                |
|                                                    | $tmp1 := f3^3$ |
| > elimsolve (tmp1,f3);                             |                |
|                                                    | $\{1 \neq 0\}$ |
| f3 is set to:                                      |                |
|                                                    | 0              |
| > tmp1 := cpCoeff (x2^4*T^2);                      |                |
|                                                    | $tmp1 := h5^4$ |
| > elimsolve (tmp1,h5);                             |                |
|                                                    | $\{1 \neq 0\}$ |
| h5 is set to:                                      |                |
|                                                    | 0              |
| > det (T - jacobian(H,[x1,x2,x3,x4,x5,x6])) mod 2; |                |
|                                                    | $T^6$          |
| > H[2];                                            |                |
|                                                    | 0              |
| > contradict (1);                                  |                |
| Contradiction on case level 0, so:                 |                |
|                                                    | $1 = 0$        |
| Variables to be uneliminated:                      |                |
|                                                    | "h5 := 'h5'"   |
|                                                    | "f3 := 'f3'"   |
|                                                    | "g4 := 'g4'"   |
|                                                    | "h4 := 'h4'"   |
|                                                    | "g3 := 'g3'"   |
|                                                    | "m6 := 'm6'"   |
|                                                    | "k5 := 'k5'"   |
|                                                    | "j4 := 'j4'"   |
|                                                    | "f2 := 'f2'"   |
|                                                    | "h3 := 'h3'"   |
|                                                    | "k4 := 'k4'"   |
|                                                    | "g2 := 'g2'"   |
|                                                    | "m5 := 'm5'"   |

```
"j3 := 'j3'"
"h2 := 'h2'"
"m4 := 'm4'"
"k3 := 'k3'"
"j2 := 'j2'"
"m3 := 'm3'"
"k2 := 'k2'"
"m2 := 'm2'"
"o1 := 'o1'"
"n1 := 'n1'"
"l1 := 'l1'"
"i1 := 'i1'"
"m1 := 'm1'"
"k1 := 'k1'"
"h1 := 'h1'"
"j1 := 'j1'"
"g1 := 'g1'"
"f1 := 'f1'"
"n2 := 'n2'"
"o2 := 'o2'"
"l2 := 'l2'"
"i2 := 'i2'"
"n3 := 'n3'"
"o3 := 'o3'"
"l3 := 'l3'"
"i3 := 'i3'"
"n4 := 'n4'"
"o4 := 'o4'"
"l4 := 'l4'"
"i4 := 'i4'"
"n5 := 'n5'"
"o5 := 'o5'"
"l5 := 'l5'"
"i5 := 'i5'"
"n6 := 'n6'"
"o6 := 'o6'"
"l6 := 'l6'"
"i6 := 'i6'"
```

That is all, folks! Check that all variables are uneliminated:

```
[[a1,b1,c1,d1,e1,f1,g1,h1,i1,j1,k1,l1,m1,n1,o1],  
 [a2,b2,c2,d2,e2,f2,g2,h2,i2,j2,k2,l2,m2,n2,o2],  
 [a3,b3,c3,d3,e3,f3,g3,h3,i3,j3,k3,l3,m3,n3,o3],  
 [a4,b4,c4,d4,e4,f4,g4,h4,i4,j4,k4,l4,m4,n4,o4],  
 [a5,b5,c5,d5,e5,f5,g5,h5,i5,j5,k5,l5,m5,n5,o5],  
 [a6,b6,c6,d6,e6,f6,g6,h6,i6,j6,k6,l6,m6,n6,o6]]
```

```
>
```
